# Supplementary material for: A spline-assisted semiparametric approach to non-parametric measurement error models
Source: arXiv:1804.00793 source file (2019-08-19)
Supplement: Supplementary file 1 [file suppmerror1.tex]

\documentclass[12pt]{article}
\usepackage{xr}
\externaldocument{errorratejasa}
\usepackage{amsmath,epsfig,amssymb,amsfonts,amsthm,epsfig,verbatim}
\usepackage{color,graphicx,lscape,longtable, subfig}
\usepackage[usenames,dvipsnames]{xcolor}
\usepackage{fancyhdr}
\usepackage{amsmath}
\usepackage{natbib}
\usepackage{enumitem}
\addtolength{\oddsidemargin}{-.5in}%
\addtolength{\evensidemargin}{-.5in}%
\addtolength{\textwidth}{1in}%
\addtolength{\textheight}{-.3in}%
\addtolength{\topmargin}{-.8in}%

\def\boxit#1{\vbox{\hrule\hbox{\vrule\kern6pt
          \vbox{\kern6pt#1\kern6pt}\kern6pt\vrule}\hrule}}

\newcommand{\mystrut}{\vphantom{\int_0^1}}

\newtheorem{Lem}{\underline{\bf Lemma}}

\def\bse{\begin{eqnarray*}}
\def\ese{\end{eqnarray*}}
\def\be{\begin{eqnarray}}
\def\ee{\end{eqnarray}}
\def\bsq{\begin{equation*}}
\def\esq{\end{equation*}}
\def\bq{\begin{equation}}
\def\eq{\end{equation}}

\def\wh{\widehat}

\def\n{\nonumber}

\def\sumi{\sum_{i=1}^n}

\def\trans{^{\rm T}}

\def\bb{\boldsymbol\beta}

\def\0{{\bf 0}}

\def\a{{\bf a}}
\def\B{{\bf B}}
\def\c{{\bf c}}
\def\C{{\bf C}}

\def\T{{\bf T}}

\def\R{{\bf R}}

\def\S{{\bf S}}

\def\u{{\bf u}}

\def\T{{\bf T}}

\def\X{{\bf X}}

\def\bq{\begin{equation}}
\def\eq{\end{equation}}
\def\pr{\hbox{pr}}
\def\wh{\widehat}

\def\trans{^{\rm T}}

\def\log{\hbox{log}}

\def\squarebox#1{\hbox to #1{\hfill\vbox to #1{\vfill}}}
\def\btheta{{\boldsymbol \theta}}

\def\bse{\begin{eqnarray*}}
\def\ese{\end{eqnarray*}}
\def\be{\begin{eqnarray}}
\def\ee{\end{eqnarray}}
\def\bsq{\begin{equation*}}
\def\esq{\end{equation*}}
\def\bq{\begin{equation}}
\def\eq{\end{equation}}
\def\pr{\hbox{pr}}
\def\wh{\widehat}

\def\log{\hbox{log}}

\def\trans{^{\rm T}}

\def\boxit#1{\vbox{\hrule\hbox{\vrule\kern6pt\vbox{\kern6pt#1\kern6pt}\kern6pt\vrule}\hrule}}

\setlength{\oddsidemargin}{0.5in} \setlength{\evensidemargin}{1in}
\setlength{\textwidth}{5.5in}     \setlength{\headsep}{0.3in}
\setlength{\parindent}{0.2in}     \setlength{\topmargin}{0.0in}
\setlength{\voffset}{-0.3in}      \setlength{\hoffset}{-0in}
\setlength{\textheight}{8.5in}    \setlength{\footskip}{0.5in}

\begin{document}
\allowdisplaybreaks 
\thispagestyle{empty}
\baselineskip=28pt
\vskip 5mm
\begin{center}
{\LARGE{\bf Supplementary Document for  ``A spline-assisted semiparametric approach to 
  nonparametric measurement error models"
\protect}}
\end{center}

\baselineskip=20pt

\section{Definitions}\label{sec:sup1}

Let $\mathcal H$ be the separable Hilbert space of square integrable functions
on $[0, 1]$, and let $<\phi_1,\phi_2>\equiv\int_0^1\phi_1(x)\phi_2(x)dx$ denote the inner product of
the functions $\phi_1, \phi_2$ in $\mathcal H$. Then the $L_2$ norm  $\|\cdot\|_2$ is the
norm induced by the inner product. 
We denote the functional $\sup$ norm as  $\|\cdot\|_\infty$,
and the $L_p$ norm as $\|\cdot\|_p$. Further, we define $\a_L$ to the
subvector of $\a$ without the first element. 

In addition, for any random function $g(x)$ with the $i$th observation
$g_i(x)$,
we define  $\Gamma (g)$ to be
a second moment based linear operator such that 
\bse  \Gamma (g) \phi(x) &\equiv&\int_0^1
E\{g_i(x)g_i(s)\} \phi(s) ds\\
&=& E\{<g_i, \phi> g_i(x)\}
\ese  while its empirical version can be written
as 
\bse
\Gamma_n (g) \phi(x) \equiv 
n^{-1}\sumi <g_i, \phi>  g_i(x) .
\ese  
Using these definitions, we can write
\bse 
<\Gamma(g) B_{rk}, B_{rl}>&=&E \left(\int_0^1 B_{rk}(x)g_i(x) dx \int_0^1 B_{rl}(x)
g_i(x) dx \right),\\
<\Gamma_n(g) B_{rk}, B_{rl}>&= & n^{-1}\sumi \int_0^1 B_{rk}(x)g_i(x) dx \int_0^1 B_{rl}(x)
g_i(x) dx.
\ese
Define ${\C}(g)$ as a $d_{\btheta} \times d_{\btheta}$ matrix with its $(k, l)$ element 
$<\Gamma(g) B_{rk}, B_{rl}>$, and $\wh{\C}(g)$ as a $d_{\btheta}
\times d_{\btheta}$  matrix matrix with its $(k, l)$  element 
$<\Gamma_n(g) B_{rk}, B_{rl}>$.   

\section{Lemmas and their Proofs}\label{sec:sup2}

\begin{Lem}\label{lem:devore1} 
There is a constant $D_r > 0 $ such that for each spline $\sum_{k=
  1}^{d_{\btheta}} c_k B_{rk}(t)$, and for each $1\leq p \leq \infty$ 
\bse
D_r \|\c'\|_p \leq \left[\int_0^1 \{\sum_{k=
  1}^{d_{\btheta}} c_k B_{rk}(t)\}^p dt\right]^{1/p} \leq \|\c'\|_p, 
\ese
where $\c' = \{c_k \{(t_k - t_{k- r} )/ r\}^{1/p}, k = 1, \ldots,
d_{\btheta}\}\trans$.
\end{Lem}
\noindent Proof: This is a direct consequence of Theorem 5.4.2 on page
145 in \cite{devore1993}. \qed

\begin{Lem}\label{lem:covC}
Let $\u$ be a $d_{\btheta}$-dimensional vector with
$\|\u\|_2 = 1$. 
There exist positive constants $D_1, D_2, D_3, D_4$ such that 
\bse
&&D_1 h_b\leq \u\trans \C(g) \u \leq D_2
h_b, \\
&& D_2^{-1} h_b^{-1}\leq \u\trans \C(g) ^{-1}\u \leq D_1^{-1}
h_b^{-1}, 
\ese
and 
\bse
&&D_3 h_b\leq \u\trans \wh{\C} (g)\u \leq D_4
h_b, \\
&&D_4^{-1} h_b^{-1}\leq \u\trans \wh{\C} (g) ^{-1}\u \leq D_3^{-1}
h_b^{-1}
\ese
in probability.

\end{Lem}
\noindent Proof: 
 First note that by the Cauchy-Schwartz inequality, 
Lemma \ref{lem:devore1} and Condition (A6), we have 
\bse 
&& E\left[\left\{\u\trans \int_0^1\B_r(x) g_i(x)dx\right\}
  ^2\right]\\
&\leq& E\left[ \int_0^1 \left\{\sum_{k = 1}^{d_{\btheta}} u_k B_{rk}(x) 
     \right\}^2dx \int_0^1 g_i(x)^2 dx\right]\\
&= & \int_0^1 \left\{\sum_{k = 1}^{d_{\btheta}} u_k B_{rk}(x) \right\}^2dx 
E\left\{\int_0^1 g_i(x)^2 dx\right\}\\
&\leq & \|\u'\|_2 ^2O(1)\\
&=& O(h_b), 
\ese 
where $\u' = \{u_k \{(t_k - t_{k- r} )/ r\}^{1/2}, k = 1, \ldots,
d_{\btheta}\}\trans$, whose $L_2$ norm is of order $O(h_b^{1/2})$. Thus 
we have 
$ \u\trans \C(\bb) \u \leq D_2 h_b$ for some positive constant $D_2 <\infty$.  

As shown in (28) in \cite{cardot2003}, since the eigenvalues of 
the covariance operator $\Gamma(g)$ are strictly positive, there is 
a positive constant $D$ such that 
$$<\Gamma(g) \phi, \phi> \geq D \|\phi\|^2, \text{ for } \phi \in 
\mathcal{H}. $$ 
Note that $\B_r\trans \u \in \mathcal{H}$, so we have 
\bse 
\u\trans \C(g) \u  = <\Gamma(g) \B_r\trans \u , \B_r\trans \u > \geq D 
\|\B_r\trans \u \|_2 \ge D_1  \|\u \|^2 h_b= D_1 h_b 
\ese 
for a positive constant $D_1$
by Lemma \ref{lem:devore1} and Condition (A4). 
Therefore, $D_1 h_b\leq \u\trans \C (g) \u \leq D_2 
h_b$. And so $D_2^{-1} h_b^{-1}\leq \u\trans \C^{-1}(g) \u \leq D_1^{-1}
h_b^{-1}$. 
Further, with Theorem 1.19 in \cite{chatelin1983}, we have 
\bse 
\|\wh{\C} (g)- \C(g)\|_2 \leq \sup_{1 \leq l\leq d_{\btheta}}\sum_{k = 1}^{d_{\btheta}}
\|\Gamma_n - \Gamma\|_2 |<B_{rk}, B_{rl}>|
\ese 
As shown in \cite{cardot2003}, Lemma 5.3 in \cite{cardot1999} implies 
$\|\Gamma_n - \Gamma\|_2 = o_p(n^{(h_b - 1)/2})$. Further, by the property of B-spline basis, we 
have when $|k - l| > r$, $B_{rk} B_{rl} = 0$. Therefore, $\sup_{1 \leq 
  l\leq d_{\btheta}}\sum_{k = 1}^{d_{\btheta}}|<B_{rk}, B_{rl}>| = O(h_b)$,
which implies \be\label{eq:disC}
\|\wh{\C} (g)- \C(g)\|_2\leq  o_p(h_b n^{(h_b - 1)/2}). 
\ee 
Now 
because $h_b<1$,  combine with the result that $D_1 h_b\leq \u\trans 
\C (g)\u \leq D_2 
h_b$, by the triangular inequality we obtain 

\bse 
 \u\trans\wh{\C} (g)\u&=& \u\trans\C (g)\u+\u\trans\{\wh{\C}(g)-\C 
 (g)\}\u\\
&\le&
D_2h_b+\|\u\|_2 \|\{\wh{\C}(g)-\C (g)\}\u\|_2\\
&\le& D_2h_b+ \|\{\wh{\C}(g)-\C (g)\}\|_2 \|\u\|_2\\
&=& D_2h_b+ o_p(h_b) 
\ese 
and 
\bse 
\u\trans\wh{\C} (g)\u&=& \u\trans\C (g)\u+\u\trans\{\wh{\C}(g)-\C 
 (g)\}\u\\
&\ge&
D_1h_b-\|\u\|_2 \|\{\wh{\C}(g)-\C (g)\}\u\|_2\\
&\ge& D_1h_b- \|\{\wh{\C}(g)-\C (g)\}\|_2 \|\u\|_2\\
&=& D_1h_b+ o_p(h_b). 
\ese 
Thus, $D_3 h_b\leq \u\trans 
\wh{\C} (g)\u \leq 
D_4 h_b$  in probability 
for some positive constant $D_3, D_4 <\infty$. And so $D^{-1}_4 h_b\leq \u\trans 
\wh{\C} (g)^{-1}\u \leq 
D_3^{-1} h_b^{-1}$  in probability. This proves the result. \qed

\begin{Lem}\label{lem:asymBr}
Assume $C_i(\cdot)$ is a continuous random function of $x \in [0, 1]$.  At
each $x$, 
$|E\{C_i(x)\}| <\infty$. $\|C_i(\cdot)\|_2 <\infty ~a.s.$.  Then 
\bse
|n^{-1}\sumi\int_0^1 B_{rk}(x) C_i (t) d x | = O_p(h_b)
\ese
if $E\{C_i (x)\}\neq 0$ and 
\bse
|n^{-1}\sumi\int_0^1 B_{rk}(x) C_i (x) d x | = O_p\{\sqrt{h_b n^{-1} \log
  (n) }\}
\ese
if $E\{C_i (x)\} =  0$. 
\end{Lem}
\noindent Proof: 
 By the Bernstein's inequality in 
\cite{bosq1998}, we have 
\bse 
&&\bigg |1/n \sumi \int_0^1 B_{rk}(x)  C_i(x) dx - E\left\{ \int_0^1 B_{rk}(x) 
  C_i(x) dx \right\}\bigg| \nonumber\\
 &=&O_p\left[ \left[\sumi E \left\{1/n\int_0^1 B_{rk}(x)  C_i(x) dx \right\}^2\log 
   n\right]^{1/2}\right] \nonumber\\
&=& O_p\{\sqrt{h_b n^{-1} \log (n)}\}. 
\ese 
The last equality 
holds from Lemma {\ref{lem:devore1}} by choosing $g_i = C_i$. 
Now if $E\{C_i (x)\}\neq 0$, 
then because $B_{rk}$ is positive in the 
interval $(t_{k - r}, t_k)$, and is 0 otherwise (page 88 in \cite{de1978}) 
\be\label{eq:expectbound}
\bigg|E \left\{\int_0^1 B_{rk}(x) C_i(x) dx\right\}\bigg| 
&=& \bigg| \int_0^1 B_{rk}(x)E\{C_i(x)\} dx \bigg|\n\\
&= &|E \{C_i(\xi) \}  \int_0^1 B_{rk}(x) dx|\n\\
&=&|E \{C_i(\xi) \} | \int_0^1 B_{rk}(x) dx \n\\
&\leq & D_9 (t_k - t_{k - r}) \n \\
&=& O_p(h_b). 
\ee 
where $\xi$ is a point in the interval $[0, 1]$, $D_9$ is a finite 
constant. The second equality holds by the assumption that $C_i(\cdot)$ is 
continuous function in $x$ and  the mean  value theorem. The inequality holds 
because the support of $B_{rk}$ is the interval $(t_{k-r}, t_k)$  and 
$|E\{C_i(x)\}| <\infty$ for any $x\in [0, 1]$. 
Therefore, by Condition (A4) that $N^{-1} n(\log n )^{-1}
\rightarrow \infty $ we have 
\bse 
\|n^{-1}\sumi \int_0^1 B_{rk}(x) C_i (x) dx\|_2 = O_p(h_b) 
\ese 
for $E\{C_i (x)\}\neq 0$ and 
\bse 
\|n^{-1}\sumi \int_0^1 B_{rk}(x) C_i (x) dx\|_2 = \sqrt{h_b n^{-1} \log (n)}
\ese 
for $E\{C_i (x)\} =  0$. 
This proves the results. \qed

\section{Proof of Proposition \ref{pro:consist}}\label{sec:appconsist}
First note that for any $h(x)$, we have
\be\label{eq:score}
&&E \left(\frac{\int_0^1\exp[\log \{f_{X0}(x)\}]f_U(W_i-x) h(x) 
dx }{\int_0^1\exp[\log \{f_{X0}(x)\}]f_U(W_i-x) dx}\right.\\
&&\left.- \frac{\int_0^1\exp[\log \{f_{X0}(x)\}]h(x)dx 
}{\int_0^1\exp[\log \{f_{X0}(x)\}]dx}\right)\n\\
&=& \int \left\{\frac{\int_0^1f_{X0}(x)f_U(y_i-x) h(x) 
dx }{\int_0^1 f_{X0}(x)f_U(y_i-x) dx}
- \int_0^1f_{X0}(x)h(x)dx\right\}\n\\
&&\times
\int_0^1 f_{X0}(x) 
f_U(w_i-x)dx d\mu(y_i)\n\\
&=&\int_0^1 \int f_{X0}(x)f_U(w_i-x) h(x) d\mu(w_i)
dx 
- \int_0^1f_{X0}(x)h(x)dx\n\\
&=&0,
\ee
hence
\bse
&&E \left[\frac{\int_0^1\exp[\log \{f_{X0}(x)\}]f_U(W_i-x) B_{rk}(x)
dx }{\int_0^1\exp[\log \{f_{X0}(x)\}]f_U(W_i-x) dx}\right.\\
&&\left.-\frac{ \int_0^1\exp[\log \{f_{X0}(x)\}] B_{rk}(x) dx
}{\int_0^1\exp[\log \{f_{X0}(x)\}]dx}\right]= 0
\ese
for each $B_{rk}(x)$, $k = 2, \ldots, d_{\btheta}$. 
Therefore, by Condition \ref{ass:dis}, we have 
\bse
&&E \left[\frac{\int_0^1\exp\{\B_r(x)\trans{\btheta}_0\}f_U(W_i-x) B_{rk}(x)
dx }{\int_0^1\exp\{\B_r(x)\trans{\btheta}_0\}f_U(W_i-x) dx}\right.\\
&&\left.- 
\frac{\int_0^1\exp\{\B_r(x)\trans{\btheta}_0\}B_{rk}(x) dx
}{\int_0^1\exp\{\B_r(x)\trans{\btheta}_0\}dx}\right]= O_p(h_b^q),
\ese
which suggests that 
\bse
&&n^{-1}\sumi \left[ \frac{\int_0^1\exp\{\B_r(x)\trans{\btheta}_0\}f_U(W_i-x) B_{rk}(x)
dx }{\int_0^1\exp\{\B_r(x)\trans{\btheta}_0\}f_U(W_i-x) dx}\right.\\
&&\left.-
\frac{ \int_0^1\exp\{\B_r(x)\trans{\btheta}_0\}B_{rk}(x) dx
}{\int_0^1\exp\{\B_r(x)\trans{\btheta}_0\}dx}\right]= o_p(1). 
\ese
Further, since 
\be\label{eq:root}
&&n^{-1}\sumi \left[ \frac{\int_0^1\exp\{\B_r(x)\trans \wh{\btheta}\}f_U(W_i-x) B_{rk}(x)
dx }{\int_0^1\exp\{\B_r(x)\trans\wh{\btheta}\}f_U(W_i-x) dx}\right.\n\\
&&\left.-\frac{ \int_0^1\exp\{\B_r(x)\trans\wh{\btheta}\}B_{rk}(x) dx
}{\int_0^1\exp\{\B_r(x)\trans\wh{\btheta}\}dx}\right]= 0,  
\ee
we have 
\be\label{eq:diff}
&&n^{-1}\sumi \left[ \frac{\int_0^1\exp\{\B_r(x)\trans{\btheta}_0\}f_U(W_i-x) \B_{rL}(x)
dx }{\int_0^1\exp\{\B_r(x)\trans{\btheta}_0\}f_U(W_i-x) dx}\right.\n\\
&&\left.-\frac{ \int_0^1\exp\{\B_r(x)\trans{\btheta}_0\}\B_{rL}(x) dx
}{\int_0^1\exp\{\B_r(x)\trans{\btheta}_0\}dx}\right]\n\\
&&- n^{-1}\sumi \left[ \frac{\int_0^1\exp\{\B_r(x)\trans \wh{\btheta}\}f_U(W_i-x) \B_{rL}(x)
dx }{\int_0^1\exp\{\B_r(x)\trans\wh{\btheta}\}f_U(W_i-x) dx}\right.\n\\
&&\left.
-\frac{ \int_0^1\exp\{\B_r(x)\trans\wh{\btheta}\}\B_{rL}(x) dx
}{\int_0^1\exp\{\B_r(x)\trans\wh{\btheta}\}dx}\right] 
= o_p(1)
\ee
element-wise.  
By Condition \ref{ass:unique}, as a function of $\btheta_L$,  
$$E\left(\left[\frac{\int_0^1\exp\{\B_r(x)\trans{\btheta}\}f_U(W_i-x) \B_{rL}(x)
dx }{\int_0^1\exp\{\B_r(x)\trans{\btheta}\}f_U(W_i-x) dx }
-\frac{ \int_0^1\exp\{\B_r(x)\trans{\btheta}\}\B_{rL}(x) dx
}{\int_0^1\exp\{\B_r(x)\trans{\btheta}\}dx}\right]\right) $$
has its derivative with respect to $\btheta_L$ being
 a nonsingular matrix in the neighborhood of its zero.
Thus,
\bse
&&n^{-1}\sumi \left[ \frac{\int_0^1\exp\{\B_r(x)\trans{\btheta}\}f_U(W_i-x) \B_{rL}(x)
dx }{\int_0^1\exp\{\B_r(x)\trans{\btheta}\}f_U(W_i-x) dx}-
\frac{ \int_0^1\exp\{\B_r(x)\trans{\btheta}\}\B_{rL}(x) dx
}{\int_0^1\exp\{\B_r(x)\trans{\btheta}\}dx}\right], 
\ese
also has nonsingular derivative with respect to $\btheta_L$
and  hence  is  an invertible function of $\btheta_L$ in the
neighborhood. Therefore, from (\ref{eq:root}) and (\ref{eq:diff}),
by the continuous mapping theorem, we
have
$\wh{\btheta}_L - \btheta_{0L} = o_p(1)$ element-wise. This proves the
results.
\qed

\section{Proof of Proposition \ref{pro:theta}}\label{sec:apptheta}

\noindent Proof: 
First note by using (\ref{eq:score}) at $h(x)=\delta(x-x_0)$ and then
set $x_0=x$,
we have 
\be\label{eq:funderiv}
&&E \left(\frac{\exp[\log\{f_{X0}(x)\}]f_U(W_i-x) 
 }{\int_0^1\exp[\log\{f_{X0}(x)\}]f_U(W_i-x) dx}
- \frac{\exp[\log\{f_{X0}(x)\}]
}{\int_0^1\exp[\log\{f_{X0}(x)\}]dx}\right)\\
&&= 0.\n
\ee
Since $\wh{\btheta}$ is the maximum likelihood estimator, we have 
\be\label{eq:theta}
{\bf 0} &=&\frac{\partial}{\partial\btheta_L} \left[n^{-1}\sumi\log\int_0^1\exp\{\B_r(x)\trans\wh{\btheta}\}f_U(W_i-x) dx \right.\n\\
&&\left.-\log\int_0^1\exp\{\B_r(x)\trans\wh\btheta\}dx\right]\n\\
&=&\R_0 + \R_1(\btheta_0) (\wh{\btheta}_L - \btheta_{0L}) + o_p\{\|\R_1(\btheta_0)(\wh{\btheta}_L - \btheta_{0L})\|_2\}, 
\ee
where for any $\btheta_L$, 
\be\label{eq:R1def}
\R_1(\btheta)&=&\frac{\partial^2}{\partial\btheta_L\partial\btheta_L\trans} 
\left[n^{-1}\sumi\log\int_0^1\exp\{\B_r(x)\trans{\btheta}\}f_U(W_i-x) dx\right.\n\\
&&\left.-\log\int_0^1\exp\{\B_r(x)\trans{\btheta}\}dx\right],
\ee
and $\btheta_L^*$ is on the line connecting $\btheta_{0L}$ and
$\wh\btheta_L$, and
\bse
\R_0 &=&n^{-1} \sumi\frac{\int_0^1\exp\{\B_r(x)\trans\btheta_0\}f_U(W_i-x) \B_{rL}(x)
dx }{\int_0^1\exp\{\B_r(x)\trans\btheta_0\}f_U(W_i-x) dx }\n\\
&&
- \frac{\int_0^1\exp\{\B_r(x)\trans \btheta_0\}\B_{rL}(x)dx
}{\int_0^1\exp\{\B_r(x)\trans \btheta_0\}dx}\\
&=& \R_{00} + \R_{01}, 
\ese
where 
\bse
\R_{00}&\equiv& n^{-1} \sumi\int_0^1\left(
\frac{\exp[\log\{f_{X0}(x)\}]f_U(W_i-x) }{\int_0^1\exp[\log\{f_{X0}(x)\}]f_U(W_i-x) dx}\right.\n\\
&&\left.
- \frac{\exp[\log\{f_{X0}(x)\}]
}{\int_0^1\exp[\log\{f_{X0}(x)\}]dx}\right)\B_r(x)dx\\
&=&  n^{-1} \sumi\int_0^1\left\{\frac{f_{X0}(x)f_U(W_i-x)
  }{\int_0^1f_{X0}(x)f_U(W_i-x) dx}- 
f_{X0}(x)\right\}\B_{rL}(x)dx
\ese 
and 
\be\label{eq:R01def}
\R_{01}&\equiv & n^{-1} \sumi\int_0^1\left[
\frac{\exp\{\B_r(x)\trans\btheta_0\}f_U(W_i-x) }{\int_0^1\exp\{\B_r(x)\trans\btheta_0\}f_U(W_i-x) dx} \right.\\
&&\left.
- \frac{\exp\{\B_r(x)\trans \btheta_0\}}{
\int_0^1\exp\{\B_r(x)\trans \btheta_0\}dx}\right]\B_{rL}(x)dx\n\\
&&- n^{-1} \sumi\int_0^1\left(\frac{\exp[\log\{f_{X0}(x)\}]f_U(W_i-x) }{\int_0^1\exp[\log\{f_{X0}(x)\}]f_U(W_i-x) dx}\right.\n\\
&&\left.- \frac{\exp[\log\{f_{X0}(x)\}]
}{\int_0^1\exp[\log\{f_{X0}(x)\}]dx}\right)\B_{rL}(x)dx.\n
\ee
Now 
\be\label{eq:R00}
\|\R_{00}\|_\infty
&=& \sup_{k = 2, \ldots,  d_{\btheta}} \bigg| n^{-1} \sumi\int_0^1\left(\frac{\exp[\log\{f_{X0}(x)\}]f_U(W_i-x) }{\int_0^1\exp[\log\{f_{X0}(x)\}]f_U(W_i-x) dx}\right.\n\\
&&\left.-\frac{ \exp[\log\{f_{X0}(x)\}]
}{\int_0^1\exp[\log\{f_{X0}(x)\}]dx}\right) B_{rk}(x)dx\bigg|\nonumber\\
&=& O_p\{\sqrt{h_b n^{-1}\log(n)}\}. 
\ee
The last equality holds by  Lemma \ref{lem:asymBr} in the supplementary material
 with 
\bse
C_i(x) &=&\frac{f_{X0}(x)f_U(W_i-x)
  }{\int_0^1f_{X0}(x)f_U(W_i-x) dx}- \frac{f_{X0}(x)
}{\int_0^1f_{X0}(x)dx}, 
\ese
 which satisfies $E\{C_i(x)\} =
0$ by (\ref{eq:funderiv}), and $\|C_i(x)\|_2 <\infty$ by Condition
\ref{ass:f}. 
Further, 
\be\label{eq:R01}
&&\|\R_{01}\|_\infty\\
&= & \sup _{k = 2, \ldots, d_{\btheta}}\left[\bigg| n^{-1} \sumi\int_0^1\left\{\left[\frac{\exp\{\B_r(x)\trans\btheta_0\}f_U(W_i-x) }{\int_0^1\exp\{\B_r(x)\trans\btheta_0\}f_U(W_i-x) dx} \right.\right.\right.\n\\
&&\left.
- \frac{\exp\{\B_r(x)\trans \btheta_0\}
}{\int_0^1\exp\{\B_r(x)\trans \btheta_0\}dx}\right]- \left(\frac{\exp[\log\{f_{X0}(x)\}]f_U(W_i-x) }{\int_0^1\exp\{f_{X0}(x)\}f_U(W_i-x) dx}\right.\n\\
&&\left.\left.\left.- \frac{\exp[\log\{f_{X0}(x)\}]
}{\int_0^1\exp[\log\{f_{X0}(x)\}]dx}\right)\right\}B_{rk}(x)dx\bigg|\right]\nonumber\\
&=& h_b^{q}\sup _{k = 2, \ldots, d_{\btheta}} \left[\bigg| n^{-1} \sumi h_b^{-q}
  \int_0^1\left\{\left[
\frac{\exp\{\B_r(x)\trans\btheta_0\}f_U(W_i-x) }{\int_0^1\exp\{\B_r(x)\trans\btheta_0\}f_U(W_i-x) dx }\right.\right.\right.\n\\
&&\left.- \frac{\exp\{\B_r(x)\trans \btheta_0\}
}{\int_0^1\exp\{\B_r(x)\trans \btheta_0\}dx}\right]
- \left(\frac{\exp[\log\{f_{X0}(x)\}]f_U(W_i-x) }{\int_0^1\exp[\log\{f_{X0}(x)\}]f_U(W_i-x) dx}\right.
\n\\
&&\left.\left.\left.- \frac{\exp[\log\{f_{X0}(x)\}]
}{\int_0^1\exp[\log\{f_{X0}(x)\}]dx}\right)\right\}B_{rk}(x)dx\bigg|\right]\nonumber\\
&=& O_p(h_b^{q + 1}).\n
\ee
The last equality holds by using Lemma \ref{lem:asymBr} in
  the supplementary material. 
  with 
\bse
&&C_i(x) \\
 &=& h_b^{-q} \left\{\left[\frac{\exp\{\B_r(x)\trans\btheta_0\}f_U(W_i-x) }{\int_0^1\exp\{\B_r(x)\trans\btheta_0\}f_U(W_i-x) dx }\right.
- \frac{\exp\{\B_r(x)\trans \btheta_0\}
}{\int_0^1\exp\{\B_r(x)\trans \btheta_0\}dx}\right]\nonumber\\
&& - \left(\frac{\exp[\log\{f_{X0}(x)\}]f_U(W_i-x) }{\int_0^1\exp[\log\{f_{X0}(x)\}]f_U(W_i-x) dx}\left.- \frac{\exp[\log\{f_{X0}(x)\}]
}{\int_0^1\exp[\log\{f_{X0}(x)\}]dx}\right)\right\}, 
\ese
which satisfies $\|C_i(x)\|_2 <\infty$.  
Combining (\ref{eq:R00}) and (\ref{eq:R01}) we have $\R_0 = \R_{00}
\{1 + o_p(1)\}$ by Conditions \ref{ass:Bknots} and
\ref{ass:Bdistance}. 
Further, 
\bse
&&E(\R_{00}\trans\R_{00})\\
  &\leq& n^{-1} E\left[\left\{\sup_{\xi}\bigg|
      \frac{f_{X0}(\xi)f_U(W_i-\xi) }{\int_0^1f_{X0}(x)f_U(W_i-x) dx}-
      f_{X0}(\xi)\bigg|\right\}^2\sum_{k = 2}^{d_{\btheta}}\left\{\int_0^1 B_{rk}(x)dx\right\}^2\right]\\
&=& O_p(n^{-1} h_b).
\ese
where $\xi$ is a point in $(0, 1)$.
 The last equality holds because
\bse
\sup_{\xi}\bigg|\frac{f_{X0}(\xi)f_U(W_i-\xi)
    }{\int_0^1f_{X0}(x)f_U(W_i-x) dx}-
    f_{X0}(\xi)\bigg|
\ese
 is bounded by Condition
\ref{ass:f}.
Further, 
\bse
\sum_{k=2}^{d_{\btheta}}\left\{\int_0^1 B_{rk}(x)dx\right\}^2
&=&\sum_{ k= 2}^{d_\btheta} D_k(t_k - t_{k - r})^2\\
&=& \sup_{k = 2, \ldots, d_{\btheta}} |t_k - t_{k - r}| D\\
&=& O_p(h_b), 
\ese
for some finite constant $D_k$ and $D$. The second equality holds 
because the support of $B_{rk}$ is the interval $(t_{k-r}, t_k)$. The
last equality holds because $D_k$ is bounded above since
$B_{rk}(x) <1$ for
any $x$.
Therefore, 
\be\label{eq:R0} \|\R_0\|_2  = O_p(n^{-1/2}h_b^{1/2}).
\ee

To analyze $\R_1(\btheta_0)$, we first
have that for any $\u$ such that $\|\u\|_2=1$,
\begin{comment}\bse
&&\left|\u\trans\frac{\partial^2 f_W(w,\btheta_0)/\partial
      \btheta_0 \partial\btheta_0\trans  }{
  f_W(w,\btheta_0)}\u\right|\\
&=&\left|\u\trans\left[\frac{\int_0^1\B_r(x)\B_r\trans(x) \exp\{\B_r(x)\trans\btheta_0\}f_U(w-x)dx}
{\int_0^1 \exp\{\B_r(x)\trans\btheta_0\}f_U(w-x)dx }\right.\right.\\
&&-\frac{\int_0^1\B_r(x)\exp\{\B_r(x)\trans\btheta_0\}f_U(w-x)dx
\int_0^1\B_r\trans(x)\exp\{\B_r(x)\trans\btheta_0\}dx}
{\int_0^1 \exp\{\B_r(x)\trans\btheta_0\}f_U(w-x)dx \int_0^1 \exp\{\B_r(x)\trans\btheta_0\}dx}\\
&&-\frac{\int_0^1\B_r(x)\exp\{\B_r(x)\trans\btheta_0\}dx
\int_0^1\B_r\trans(x)\exp\{\B_r(x)\trans\btheta_0\}f_U(w-x)dx}
{\int_0^1 \exp\{\B_r(x)\trans\btheta_0\}dx \int_0^1 \exp\{\B_r(x)\trans\btheta_0\}f_U(w-x)dx}\\
&&-\frac{\int_0^1\B_r(x)\B_r\trans(x) \exp\{\B_r(x)\trans\btheta_0\}dx}
{\int_0^1 \exp\{\B_r(x)\trans\btheta_0\}dx}\\
&&\left.\left.+2 \frac{\int_0^1\B_r(x)\exp\{\B_r(x)\trans\btheta_0\}dx
\int_0^1\B_r\trans(x)\exp\{\B_r(x)\trans\btheta_0\}dx}
{\{\int_0^1 \exp\{\B_r(x)\trans\btheta_0\}dx\}^2}\right]\u\right|\\
&\le&6\sup_{x\in[0,1]}\{\u\trans\B_r(x)\}^2\\
&\le&6N.
\ese
Further,\end{comment}
 from Lemma \ref{lem:devore1} in the supplementary material,
\bse
&&\u\trans\frac{\int_0^1\B_{rL}(x)\B_{rL}\trans(x) \exp\{\B_r(x)\trans\btheta_0\}f_U(W_i-x)dx}
{\int_0^1 \exp\{\B_r(x)\trans\btheta_0\}f_U(W_i-x)dx }\u\\
&=&\left\|\B_{rL}(x)\trans \frac{\u\exp\{\B_r(x)\trans\btheta_0/2\}f_U^{1/2}(W_i-x)}
{[\int_0^1 \exp\{\B_{r}(x)\trans\btheta_0\}f_U(W_i-x)dx]^{1/2}
}\right\|_2^2\\
&=&O_p\left[h_b\left\| \frac{\u\exp\{\B_r(x)\trans\btheta_0/2\}f_U^{1/2}(W_i-x)}
{[\int_0^1 \exp\{\B_{rL}(x)\trans\btheta_0\}f_U(W_i-x)dx]^{1/2}
}\right\|_2^2\right]\\
&=&O_p(h_b),
\ese
and
\bse
\u\trans\frac{\int_0^1\B_{rL}(x)\B_{rL}\trans(x) \exp\{\B_r(x)\trans\btheta_0\}dx}
{\int_0^1 \exp\{\B_r(x)\trans\btheta_0\}dx }\u
&=&\left\|\B_{rL}(x)\trans \frac{\u\exp\{\B_r(x)\trans\btheta_0/2\}}
{[\int_0^1 \exp\{\B_r(x)\trans\btheta_0\}dx]^{1/2}
}\right\|_2^2\\
&=&O\left[h_b\left\| \frac{\u\exp\{\B_r(x)\trans\btheta_0/2\}}
{[\int_0^1 \exp\{\B_r(x)\trans\btheta_0\}dx]^{1/2}
}\right\|_2^2\right]\\
&=&O(h_b).
\ese
Similarly
\bse
&&\u\trans\frac{\int_0^1\B_{rL}(x)\exp\{\B_r(x)\trans\btheta_0\}f_U(W_i-x)dx
\int_0^1\B_{rL}\trans(x)\exp\{\B_r(x)\trans\btheta_0\}dx}
{\int_0^1 \exp\{\B_r(x)\trans\btheta_0\}f_U(W_i-x)dx \int_0^1
  \exp\{\B_r(x)\trans\btheta_0\}dx}\u\\
&\le&\left[\frac{\int_0^1 \u\trans\B_{rL}(x)\exp\{\B_r(x)\trans\btheta_0\}f_U(W_i-x)dx}
{\int_0^1 \exp\{\B_r(x)\trans\btheta_0\}f_U(W_i-x)dx}\right]^2\\
&&+\left[\frac{
\int_0^1\B_{rL}\trans(x) \u\exp\{\B_r(x)\trans\btheta_0\}dx}
{\int_0^1 \exp\{\B_r(x)\trans\btheta_0\}dx}\right]^2,
\ese
while
\bse
&&\left[\frac{
\int_0^1\B_{rL}\trans(x) \u\exp\{\B_r(x)\trans\btheta_0\}f_U(W_i-x)dx}
{\int_0^1 \exp\{\B_r(x)\trans\btheta_0\}f_U(W_i-x)dx }\right]^2\\
&\le&\left\|\frac{
\B_{rL}\trans(x) \u\exp\{\B_r(x)\trans\btheta_0\}f_U(W_i-x)}
{\int_0^1 \exp\{\B_r(x)\trans\btheta_0\}f_U(W_i-x)dx}\right\|_1^2\\
&\le&O_p\left[h_b \left\|\frac{ \u\exp\{\B_r(x)\trans\btheta_0\}f_U(W_i-x)}
{\int_0^1 \exp\{\B_r(x)\trans\btheta_0\}dxf_U(W_i-x)}\right\|_1\right]^2\\
&\le&O_p(h_b^2),
\ese
and
\bse
\left[\frac{
\int_0^1\B_{rL}\trans(x) \u\exp\{\B_r(x)\trans\btheta_0\}dx}
{\int_0^1 \exp\{\B_r(x)\trans\btheta_0\}dx}\right]^2
&\le&\left\|\frac{
\B_{rL}\trans(x) \u\exp\{\B_r(x)\trans\btheta_0\}}
{\int_0^1 \exp\{\B_r(x)\trans\btheta_0\}dx}\right\|_1^2\\
&\le&O\left[h_b \left\|\frac{ \u\exp\{\B_r(x)\trans\btheta_0\}}
{\int_0^1 \exp\{\B_r(x)\trans\btheta_0\}dx}\right\|_1\right]^2\\
&\le&O(h_b^2).
\ese
Combining these results, we have
\bse
&&\left|\u\trans\frac{\partial^2 f_W(w,\btheta_0)/\partial
      \btheta_0 \partial\btheta_0\trans  }{
  f_W(w,\btheta_0)}\u\right|\\
&=&\left|\u\trans\left[\frac{\int_0^1\B_{rL}(x)\B_{rL}\trans(x) \exp\{\B_r(x)\trans\btheta_0\}f_U(w-x)dx}
{\int_0^1 \exp\{\B_r(x)\trans\btheta_0\}f_U(w-x)dx }\right.\right.\\
&&-\frac{\int_0^1\B_{rL}(x)\exp\{\B_{rL}(x)\trans\btheta_0\}f_U(w-x)dx
\int_0^1\B_{rL}\trans(x)\exp\{\B_r(x)\trans\btheta_0\}dx}
{\int_0^1 \exp\{\B_r(x)\trans\btheta_0\}f_U(w-x)dx \int_0^1 \exp\{\B_r(x)\trans\btheta_0\}dx}\\
&&-\frac{\int_0^1\B_{rL}(x)\exp\{\B_r(x)\trans\btheta_0\}dx
\int_0^1\B_{rL}\trans(x)\exp\{\B_r(x)\trans\btheta_0\}f_U(w-x)dx}
{\int_0^1 \exp\{\B_r(x)\trans\btheta_0\}dx \int_0^1 \exp\{\B_r(x)\trans\btheta_0\}f_U(w-x)dx}\\
&&-\frac{\int_0^1\B_{rL}(x)\B_{rL}\trans(x) \exp\{\B_r(x)\trans\btheta_0\}dx}
{\int_0^1 \exp\{\B_r(x)\trans\btheta_0\}dx}\\
&&\left.\left.+2 \frac{\int_0^1\B_{rL}(x)\exp\{\B_r(x)\trans\btheta_0\}dx
\int_0^1\B_{rL}\trans(x)\exp\{\B_r(x)\trans\btheta_0\}dx}
{\{\int_0^1 \exp\{\B_r(x)\trans\btheta_0\}dx\}^2}\right]\u\right|\\
&=&O_p(h_b),
\ese
and
\bse
&&E\left[\left\{\u\trans \frac{\partial^2 f_W(W_i,\btheta_0)/\partial
      \btheta_{0L} \partial\btheta_{0L}\trans}{
  f_W(W_i,\btheta_0)}\u\right\}^2\right]\\
&=&E\left\{\left(\u\trans\left[\frac{\int_0^1\B_{rL}(x)\B_{rL}\trans(x) \exp\{\B_r(x)\trans\btheta_0\}f_U(W_i-x)dx}
{\int_0^1 \exp\{\B_r(x)\trans\btheta_0\}f_U(W_i-x)dx }\right.\right.\right.\\
&&-\frac{\int_0^1\B_{rL}(x)\exp\{\B_r(x)\trans\btheta_0\}f_U(W_i-x)dx
\int_0^1\B_{rL}\trans(x)\exp\{\B_r(x)\trans\btheta_0\}dx}
{\int_0^1 \exp\{\B_r(x)\trans\btheta_0\}f_U(W_i-x)dx \int_0^1 \exp\{\B_r(x)\trans\btheta_0\}dx}\\
&&-\frac{\int_0^1\B_{rL}(x)\exp\{\B_r(x)\trans\btheta_0\}dx
\int_0^1\B_{rL}\trans(x)\exp\{\B_r(x)\trans\btheta_0\}f_U(W_i-x)dx}
{\int_0^1 \exp\{\B_r(x)\trans\btheta_0\}dx \int_0^1 \exp\{\B_r(x)\trans\btheta_0\}f_U(W_i-x)dx}\\
&&-\frac{\int_0^1\B_{rL}(x)\B_{rL}\trans(x) \exp\{\B_r(x)\trans\btheta_0\}dx}
{\int_0^1 \exp\{\B_r(x)\trans\btheta_0\}dx}\\
&&\left.\left.\left.+2 \frac{\int_0^1\B_{rL}(x)\exp\{\B_r(x)\trans\btheta_0\}dx
\int_0^1\B_{rL}\trans(x)\exp\{\B_r(x)\trans\btheta_0\}dx}
{\{\int_0^1
  \exp\{\B_r(x)\trans\btheta_0\}dx\}^2}\right]\u\right)^2\right\}\\
&=&O_p(h_b^2).
\ese
Now using Bernstein's inequality, for $\epsilon=h_b/\log(n)$, 
\bse
&&\pr\left[\u\trans\R_1(\btheta_0)\u-\u\trans
E\{\R_1(\btheta_0)\}\u>\epsilon\right]\\
&\le& \exp\left[\frac{-n^2\epsilon^2/2}{
nE(
\u\trans
[{\partial^2 f_W(W_i,\btheta_0)/\partial
      \btheta_{0L} \partial\btheta_{0L}\trans}/{
  f_W(W_i,\btheta_0)}
-E\{\R_1(\btheta_0)\}]\u)^2+nh_b\epsilon/3}\right]\\
&\le& \exp\left(\frac{-n\epsilon^2/2}{
E[\{\u\trans {\partial^2 f_W(W_i,\btheta_0)/\partial
      \btheta_{0L} \partial\btheta_{0L}\trans}/{
  f_W(W_i,\btheta_0)}
\u\}^2]+h_b\epsilon/3}\right)\\
&\le& \exp\left(\frac{-n\epsilon^2/2}{h_b^2+h_b\epsilon/3}\right)\to 0
\ese
when $n\to\infty$. Thus, 
\be\label{eqn:RE}
|\u\trans\R_1(\btheta_0)\u-\u\trans
E\{\R_1(\btheta_0)\}\u|=o_p(h_b).
\ee
Further, 
\be\label{eqn:RE2}
 && E\{\R_1(\btheta_0 )\} \\
&=&E\left\{ \frac{\partial^2 f_W(W_i,\btheta_0)/\partial
      \btheta_{0L} \partial\btheta_{0L}\trans  }{
  f_W(W_i,\btheta_0)}\right\}-  E \left[\left\{\frac{\partial \log
    f_W(W_i,\btheta_0)}{\partial \btheta_{0L}}\right\}^{\otimes2}\right]\n\\
&=& \int \left\{ \frac{\partial^2 f_W(w,\btheta_0)/\partial
      \btheta_{0L} \partial\btheta_{0L}\trans  }{
  f_W(w,\btheta_0)}\right\} f_{W0}(w) dw -  E \left[\left\{\frac{\partial \log
    f_W(W_i,\btheta_0)}{\partial \btheta_{0L}}\right\}^{\otimes2}\right]\n\\
&=& O_p(h_b^{q - 1}) - E \left[\left\{\frac{\partial \log
    f_W(W_i,\btheta_0)}{\partial \btheta_{0L}}\right\}^{\otimes2}\right]\n, 
\ee
where $f_{W0}(w)$ is the true density of $W$. The last equality holds
by Condition \ref{ass:dis} so that 
\bse
&&\bigg\| \int \left\{ \frac{\partial^2 f_W(w,\btheta_0)/\partial
      \btheta_{0L} \partial\btheta_{0L}\trans  }{
  f_W(w,\btheta_0)}\right\} f_{W0}(w) dw \n\\
&&- \int \left\{ \frac{\partial^2 f_W(w,\btheta_0)/\partial
      \btheta_{0L} \partial\btheta_{0L}\trans  }{
  f_W(w,\btheta_0)}\right\}f_W(w,\btheta_0) dw\bigg\|_2 = O_p(h_b^{q-1})
\ese
and the fact that  $\int
f_{W}(w,\btheta) dw = 1$ so 
\bse
&& \int \left\{ \frac{\partial^2 f_W(w,\btheta_0)/\partial
      \btheta_{0L} \partial\btheta_{0L}\trans  }{
  f_W(w,\btheta_0)}\right\}f_W(w,\btheta_0) dw\\
&=& \frac{\partial^2 \int  f_W(w,\btheta_0) d w}{\partial
      \btheta_{0L} \partial\btheta_{0L}\trans}\\
&=& \bf 0.
\ese 
Now 
\be\label{eqn:RE3}
&& E \left[\left\{\frac{\partial \log
    f_W(W_i,\btheta)}{\partial \btheta_L}\right\}^{\otimes2}\right]\\
&= & E \left(\left[\frac{\int_0^1\exp\{\B_r(x)\trans{\btheta}\}f_U(W_i-x) \B_{rL}(x)
dx }{\int_0^1\exp\{\B_r(x)\trans{\btheta}\}f_U(W_i-x) dx }\right.\right.\n\\
&&\left.\left.-\frac{ \int_0^1\exp\{\B_r(x)\trans{\btheta}\}\B_{rL}(x) dx
}{\int_0^1\exp\{\B_r(x)\trans{\btheta}\}dx}\right]^{\otimes2}\right)\n. 
\ee
First,  $$E \left(\left[\frac{\int_0^1\exp\{\B_r(x)\trans{\btheta}\}f_U(W_i-x) \B_{rL}(x)
dx }{\int_0^1\exp\{\B_r(x)\trans{\btheta}\}f_U(W_i-x) dx }
-\frac{ \int_0^1\exp\{\B_r(x)\trans{\btheta}\}\B_{rL}(x) dx
}{\int_0^1\exp\{\B_r(x)\trans{\btheta}\}dx}\right]^{\otimes2}\right)
\neq 0 $$ by Condition \ref{ass:unique}. Also, 
it is easy to see that, $$E\left(\left[\frac{\int_0^1\exp\{\B_r(x)\trans{\btheta}\}f_U(W_i-x) \B_{rL}(x)
dx }{\int_0^1\exp\{\B_r(x)\trans{\btheta}\}f_U(W_i-x) dx }
-\frac{ \int_0^1\exp\{\B_r(x)\trans{\btheta}\}\B_{rL}(x) dx
}{\int_0^1\exp\{\B_r(x)\trans{\btheta}\}dx}\right]^{\otimes2}\right)$$ is $\C(g)$
defined in Section \ref{sec:sup1} in the supplementary material with 
\bse
g_i(x)=\frac{\exp\{\B_r(x)\trans\btheta\}f_U(W_i-x)}{\int_0^1\exp\{\B_r(x)\trans\btheta\}f_U(W_i-x)
dx}
  - \frac{\exp\{\B_r(x)\trans{\btheta}\}}{\int_0^1\exp\{\B_r(x)\trans{\btheta}\}dx}.
\ese
Hence by using Lemma \ref{lem:covC} in the supplementary material, for  $\u$ such that
$\|\u\|_2=1$, we have that there exist constants $C >c>0$, such that
\be\label{eqn:RE4}
c  h_b&\leq&  \u\trans E \left(\left[\frac{\int_0^1\exp\{\B_r(x)\trans{\btheta}\}f_U(W_i-x) \B_{rL}(x)
dx }{\int_0^1\exp\{\B_r(x)\trans{\btheta}\}f_U(W_i-x) dx }\right.\right.\\
&&\left.\left.-\frac{ \int_0^1\exp\{\B_r(x)\trans{\btheta}\}\B_{rL}(x) dx
}{\int_0^1\exp\{\B_r(x)\trans{\btheta}\}dx}\right]^{\otimes2}\right)\u
\leq C h_b\n. 
\ee
Combining the results in (\ref{eqn:RE}), (\ref{eqn:RE2}),
(\ref{eqn:RE3}) and (\ref{eqn:RE4}), there exist constants $0<c_1 < C_1
$, such that
\bse
-C_1 h_b \leq \u\trans \R_{1}(\btheta_0) \u \leq -c_1 h_b
\ese
in probability, and  in turn 
\be\label{eq:R1inver}
-c_1^{-1} h_b^{-1} \leq \u\trans \R_{1}(\btheta_0)^{-1} \u \leq
-C_1^{-1} h_b^{-1}
\ee
in probability.
Therefore, red
$
\|\wh{\btheta}_L - \btheta_{0L}\|_2  
=O_p(\|\R_1(\btheta_0)^{-1}\R_0\|_2)
\leq O_p\{\|\R_1(\btheta_0)^{-1}\|_2 \|\R_0\|_2\} = O_p\{(nh_b)^{-1/2}\}. 
$
 Therefore, for any vector $\a$ with $\|\a\|_2 = O_p(1)$ we have
$|\a\trans (\wh{\btheta}_L - \btheta_{0L})| \leq  \|\a\|_2 \|(\wh{\btheta}_L
- \btheta_{0L})\|_2 = O_p\{(nh_b)^{-1/2}\}$. 

\begin{comment}
By the consistency of $\B_r(x)\trans\btheta ^* $ to $\log\{f_{X0}(x)\}$, 
\bse
&&\R_1(\btheta^*)\\
&=&E\left( \frac{\int_0^1\exp[\log\{f_{X0}(x)\}]f_U(W_i-x) \B_r(x)\B_r(x)\trans
dx }{\int_0^1\exp[\log\{f_{X0}(x)\}]f_U(W_i-x) dx}\right. \\
&& - \frac{\left[\int_0^1\exp[\log\{f_{X0}(x)\}]f_U(W_i-x) \B_r(x)
dx \right]^{\otimes2}}{\left[\int_0^1\exp[\log\{f_{X0}(x)\}]f_U(W_i-x) dx \right]^2}\\
&& - \frac{\int_0^1\exp[\log\{f_{X0}(x)\}]\B_r(x)
\B_r(x)\trans dx
}{\int_0^1\exp[\log\{f_{X0}(x)\}]dx }
 \\
&&\left.+\frac{ \left[\int_0^1\exp[\log\{f_{X0}(x)\}]\B_r(x) dx\right]^{\otimes2}
}{\left[\int_0^1\exp[\log\{f_{X0}(x)\}]dx\right]^2}\right)\{1 +
o_p(1)\}\\
&=&E \left[\frac{\int_0^1 f_{X0}(x)f_U(W_i-x) \B_r(x)\B_r(x)\trans
dx }{\int_0^1 f_{X0}(x)f_U(W_i-x) dx}\right. \\
&&- \frac{\left\{\int_0^1f_{X0}(x)f_U(W_i-x) \B_r(x)
dx \right\}^{\otimes2}}{\left\{\int_0^1 f_{X0}(x)f_U(W_i-x) dx \right\}^2}\\
&& \left.- \int_0^1 f_{X0}(x)\B_r(x)
\B_r(x)\trans dx+ \left\{\int_0^1 f_{X0}(x)\B_r(x)
  dx\right\}^{\otimes2}\right]\{1 + o_p(1)\}.
\ese
\end{comment}
Further,  expanding the second derivative, 
we can write 
\bse
&&\R_1(\btheta_0)\\
&=&E\left( \frac{\int_0^1\exp[\log\{f_{X0}(x)\}]f_U(W_i-x) \B_{rL}(x)\B_{rL}(x)\trans
dx }{\int_0^1\exp[\log\{f_{X0}(x)\}]f_U(W_i-x) dx}\right. \\
&& - \frac{\left[\int_0^1\exp[\log\{f_{X0}(x)\}]f_U(W_i-x) \B_{rL}(x)
dx \right]^{\otimes2}}{\left[\int_0^1\exp[\log\{f_{X0}(x)\}]f_U(W_i-x) dx \right]^2}\\
&& - \frac{\int_0^1\exp[\log\{f_{X0}(x)\}]\B_r(x)
\B_r(x)\trans dx
}{\int_0^1\exp[\log\{f_{X0}(x)\}]dx }
 \\
&&\left.+\frac{ \left[\int_0^1\exp[\log\{f_{X0}(x)\}]\B_{rL}(x) dx\right]^{\otimes2}
}{\left[\int_0^1\exp[\log\{f_{X0}(x)\}]dx\right]^2}\right)\{1 +
o_p(1)\}\\
&=&E \left[\frac{\int_0^1 f_{X0}(x)f_U(W_i-x) \B_{rL}(x)\B_{rL}(x)\trans
dx }{\int_0^1 f_{X0}(x)f_U(W_i-x) dx}\right. \\
&&- \frac{\left\{\int_0^1f_{X0}(x)f_U(W_i-x) \B_{rL}(x)
dx \right\}^{\otimes2}}{\left\{\int_0^1 f_{X0}(x)f_U(W_i-x) dx \right\}^2}\\
&& \left.- \int_0^1 f_{X0}(x)\B_{rL}(x)
\B_{rL}(x)\trans dx+ \left\{\int_0^1 f_{X0}(x)\B_{rL}(x)
  dx\right\}^{\otimes2}\right]\{1 + o_p(1)\}.
\ese

Hence we can write 
\bse
&&\wh{\btheta}_L -\btheta_{0L} \\
&=& \left(E \left[\frac{\int_0^1 f_{X0}(x)f_U(W_i-x) \B_{rL}(x)\B_{rL}(x)\trans
dx }{\int_0^1 f_{X0}(x)f_U(W_i-x) dx}\right.\right.\\
&&- \frac{\left\{\int_0^1f_{X0}(x)f_U(W_i-x) \B_{rL}(x)
dx \right\}^{\otimes2}}{\left\{\int_0^1 f_{X0}(x)f_U(W_i-x) dx \right\}^2}\\
&&- \int_0^1 f_{X0}(x)\B_{rL}(x)
\B_{rL}(x)\trans dx\\
&&\left.\left.+ \left\{\int_0^1 f_{X0}(x)\B_{rL}(x)
  dx\right\}^{\otimes2}\right]\right)^{-1} \R_{00} \{1 + o_p(1)\}. 
\ese
This proves the results. \qed

\section{Proof of Proposition \ref{pro:betaconsis}}\label{sec:appbetaconsis}
First note that by the definition of $\a(\X,m)$, we have
\bse 
E[\S^*_{\bb}(W_i, Y_i, m) -E^*\{\a(X,m) \mid Y_i, W_i, m\}\mid\X,
m]=\0. 
\ese
This leads to
\be\label{eq:ebb0}
E[\S^*_{\bb}(W_i, Y_i,\bb_0) -E^*\{\a(X,\bb_0) \mid Y_i,
W_i,\bb_0\}]= o_p(1)
\ee
element-wise by Condition \ref{ass:mdis}. 
By Condition \ref{ass:munique}, $E[\S^*_{\bb}(W_i, Y_i,\bb) -E^*\{\a(X,\bb) \mid Y_i,
W_i,\bb\}]$ is invertible near $\bb^*$ and its inverse
function is a one-to-one function with bounded first derivative 
in the neighborhood of zero. Therefore
$\|\bb^*-\bb_0\|_2=o_p(1)$.
On the other hand, since 
\be\label{eq:hattheta}
 n^{-1}\sumi \S^*_{\bb}(W_i, Y_i,\wh{\bb}) -E^*\{\a(X, \wh{\bb}) \mid Y_i, W_i, \wh{\bb}\}=\0,
\ee
we obtain
\bse
E[\S^*_{\bb}(W_i, Y_i,\wh{\bb}) -E^*\{\a(X, \wh{\bb}) \mid Y_i, W_i,
\wh{\bb}\}]=o_p(1).
\ese
Using the same argument regarding $\bb_0$ in (\ref{eq:ebb0}), we obtain
$\|\wh\bb-\bb^*\|_2=o_p(1)$.  Thus, $\|\wh\bb-\bb_0\|_2=o_p(1)$.
\qed

\section{Proof of Proposition \ref{pro:beta}}\label{sec:appbeta}
By the Taylor expansion, we have 
\be\label{eq:beta}
\bf 0 &=& \sumi \S^*_{\bb}(W_i, Y_i,\wh{\bb}) -E^*\{\a(X, \wh\bb) \mid Y_i, W_i,
\wh{\bb}\}\nonumber\\
&=&\T_{0} +\T_1(\bb^*)(\wh{\bb} - \bb_0),   
\ee
where $\bb^*$ is a point on the line connecting $\bb_0$ and
$\wh{\bb}$ , and for any $\bb$
\bse
\T_1(\bb) = n^{-1}\sumi \frac{\partial[\S^*_{\bb}(W_i, Y_i, {\bb})
  -E^*\{\a(X, \bb) \mid Y_i, W_i,
{\bb}\}]}{\partial \bb\trans}, 
\ese
and 
\bse
\T_0 &=& n^{-1}\sumi \S^*_{\bb}(W_i, Y_i, {\bb}_0) -E^*\{\a(X, \bb_0) \mid Y_i, W_i,
{\bb}_0\}\\
&=& \T_{00} + \T_{01},
\ese
where 
\bse
\T_{00} = n^{-1}\sumi \S^*_{\bb}(W_i, Y_i, m) -E^*\{\a(X, m) \mid Y_i, W_i,
m \},
\ese
and  
\bse
\T_{01} &=&  n^{-1}\sumi \S^*_{\bb}(W_i, Y_i, {\bb}_0) -E^*\{\a(X, \bb_0) \mid Y_i, W_i,
{\bb}_0\} \\
&&- \left[n^{-1}\sumi \S^*_{\bb}(W_i, Y_i, m) -E^*\{\a(X, m) \mid Y_i, W_i,
m \}\right].
\ese
By the definition of $\S^*_{\bb}(W_i, Y_i,m)$, we can write 
\be\label{eq:T000}
\|\T_{00}\|_\infty &=& \sup_k \bigg|n^{-1}\sumi \int_0^1\left[-\frac{
    f'_\epsilon\{Y_i-m(x)\}f_U(W_i-x) f^*_X(x)}{\int_0^1
    f_\epsilon\{Y_i- m(x)\}f_U(W_i-x) f^*_X(x) 
d\mu(x)}\nonumber\right.\\
&&\left.- P(x, W_i, Y_i, m)\mystrut\right]B_{rk}(x) d\mu(x)\bigg|.
\ee
Now define \bse
C_{1i}(x) = \left[-\frac{f'_\epsilon\{Y_i-m(x)\}f_U(W_i-x) f^*_X(x)}{\int_0^1 
f_\epsilon\{Y_i- m(x)\}f_U(W_i-x) f^*_X(x) 
d\mu(x)}- P(x, W_i, Y_i, m)\right], 
\ese by the Bernstein's inequality in 
\cite{bosq1998}, we have 
\be\label{eq:bosq} 
&&\bigg |1/n \sumi \int_0^1 B_{rk}(x)  C_{1i}(x) d x - E\left\{ \int_0^1 B_{rk}(x) 
  C_{1i}(x) d x \right\}\bigg| \nonumber\\
 &=&O_p\left(\left[\sumi E \left\{1/n\int_0^1 B_{rk}(x)  C_{1i}(x) dx \right\}^2\log 
   n\right]^{1/2}\right) \nonumber\\
&=& O_p\{\sqrt{h_b n^{-1} \log (n)}\}. 
\ee 
The last equality 
holds from Lemma \ref{lem:covC} in the supplementary material, by choosing $g_i(x)=
C_{1i}(x)$ and setting $\u$  with $u_{k} = 1$ and $u_{l} = 0$,
for $l\neq k$. 
Now 
\bse
&&E[\S^*_{\bb}(W_i, Y_i,m ) -E^*\{\a(X, m) \mid Y_i, W_i, m\} ] \\
&=& 
E\left(\int_0^1\left[ -\frac{ f'_\epsilon\{Y-m(x)\}f_U(W-x) f^*_X(x) }{\int_0^1
f_\epsilon\{Y-m(x)\}f_U(W-x) f^*_X(x) dx} - P(x, W, Y,m) \right]
\B_r(x) dx \right)\\
&=& \bf 0, 
\ese
which further implies  $E
\left\{\int_0^1 B_{rk}(x) C_{1i}(x) dx\right\}= 0$ for all $k$. Plug it into
(\ref{eq:bosq}), and combine with (\ref{eq:T000}),  we obtain
\be\label{eq:T00}
\|\T_{00}\|_\infty 
&=&O_p\{\sqrt{h_b n^{-1}\log(n)}\}.
\ee
Further, 
\be\label{eq:T01}
&&\|\T_{01}\|_\infty \\
&=& \sup_k \bigg|n^{-1}\sumi \int_0^1\left(\left[-\frac{ f'_\epsilon\{Y_i-\B_r(x)\trans\bb_0\}f_U(W_i-x) f^*_X(x)}{\int_0^1 
f_\epsilon\{Y_i- \B_r(x)\trans\bb_0\}f_U(W_i-x) f^*_X(x) 
d\mu(x)}\right.\right.\n\\
&&\left.- P(x, W_i, Y_i, \bb_0)\right]
- \left.\left[-\frac{ f'_\epsilon\{Y_i-m(x)\}f_U(W_i-x) f^*_X(x)}{\int_0^1 
f_\epsilon\{Y_i- m(x)\}f_U(W_i-x) f^*_X(x) 
d\mu(x)}\right.\right.\n\\
&&\left.\left.- P(x, W_i, Y_i, m)\right]\right)B_{rk}(x) d\mu(x)\bigg|\nonumber\\
&=& \sup_k  \bigg|n^{-1}\sumi  \frac{\partial S_m(Y_i, W_i, m)}{\partial m}(B_{rk},
\B_{r}\trans\bb - m)\bigg| \{1 + o_p(1)\}\nonumber\\
&=& O_p(1)\sup_k \left\{\int_0^1 B_{rk}(x)
  dx\right\} \left\{\sup_{x\in [0, 1]} |\B_{r}(x)\trans\bb - m(x)|\right\}  \{1 + o_p(1)\}\nonumber\\
&=& O_p(h_b^{q+1}), \n
\ee
The second equality holds by the Taylor expansion with respect to
$\B_r(\cdot)\trans\bb$. The third equality holds by Condition
\ref{ass:2deriv}. The last equality holds by Condition \ref{ass:mdis}
and 
the fact that the support of $B_{rk}$ is the interval $(t_{k-r}, t_k)$. 
Combining (\ref{eq:T00}) and (\ref{eq:T01}) we have $\T_0 = \T_{00}
\{1 + o_p(1)\}$ by Conditions \ref{ass:Bknots} and \ref{ass:Bdistance}.
Further, 
\bse
&&E(\T_{00}\trans\T_{00})\\
&=& n^{-1} E\left\{\left(\sum_{l=1}^{d_{\bb}}\int_0^1\left[ -\frac{ f'_\epsilon\{Y_i-m(x)\}f_U(W_i-x) f^*_X(x)}{\int_0^1 
f_\epsilon\{Y_i- m(x)\}f_U(W_i-x) f^*_X(x) 
d\mu(x)}\right.\right.\right.\n\\
&&\left.\left.\left.- P(x, W_i, Y_i,
m)\right] B_{rl}(x)dx\right)^2\right\}\\
&\leq& n^{-1}  G_1 \sum_{l=1}^{d_\beta}\left\{\int_0^1 B_{rl}(x)dx\right\}^2\\
&=& O_p(n^{-1} h_b), 
\ese
for some constant $G_1$.  The second
equality holds by Condition \ref{ass:2deriv} and the fact that, 
\bse
&&\sum_{l=1}^{d_{\bb}}\left\{\int_0^1 B_{rl}(x)dx\right\}^2\\
&=&\sum_{l = 1}^{d_{\bb}} D_{1l} (t_l - t_{l - r})^2\\
&\leq& \sup_{l} |t_l - t_{l - r}| D_1\\
&=& O_p(h_b), 
\ese
for some finite constant $D_{1l}$ and $D_1$. The second equality holds 
because the support of $B_{rl}$ is the interval $(t_{l-r}, t_l)$. The
last equality holds because $D_{1l}$ are bounded above since
$B_{rl}(x) <1$ for
any $x$.
Therefore, 
\be\label{eq:T0} \|\T_0\|_2  = O_p(n^{-1/2}h_b^{1/2}).
\ee
Further  for arbitrary vector $\u$ with $\|\u\|_2 = 1$, we can write
$\T_1 (\bb^*)$ as 
\bse
|\u\trans \T_{1}(\bb^*)\u| 
&=& \bigg|n^{-1}\sumi \frac{\partial S_m(Y_i, W_i, m^*)}{\partial m^*}\left(\sum_{k
= 1}^{d_{\bb}} u_k B_{rk},  \sum_{k
= 1}^{d_{\bb}} u_k B_{rk}\right)\bigg| \\
&=& O_p(1) \|\sum_{k
= 1}^{d_{\bb}} u_k B_{rk}\|_2^2, 
\ese
where $m^*(\cdot) = \B_r(\cdot)\trans\bb^*$. The last equality holds by Condition \ref{ass:2deriv}.
Further
by using Lemme 1 in the supplementary material,
%\cite{jiang2016}, 
we
have $ g_3 h_b^{1/2}= D_r \|\u'\|_2\leq\|\sum_{k
= 1}^{d_{\bb}} u_k B_{rk}\|_2 \leq \|\u'\|_2 = G_3 h_b^{1/2}$, where $\u' = \{u_k \{(t_k - t_{k- r} )/ r\}^{1/2}, k = 1, \ldots,
d_{\bb}\}\trans$ and $g_3, G_3$ are finite constants.
This implies
\bse
c_9h_b\leq \u\trans\T_{1}(\bb^*)\u\leq C_9 h_b, 
\ese
and 
\be\label{eq:T1inver}
C_9^{-1}h_b^{-1}\leq \u\trans\T_{1}(\bb^*)^{-1}\u\leq c_9^{-1}
h_b^{-1}, 
\ee
in probability. 
Combining with
(\ref{eq:beta}), 
(\ref{eq:T0}), we have 
\bse
\|\wh{\bb} - \bb_0\|_2  \leq \|\T_1(\bb^*)^{-1}\|_2 \|\T_0\|_2 =
O_p\{(nh_b)^{-1/2}\}.
\ese
 By the consistency of $\B_r(x)\trans\bb ^* $ to
$m(x)$, we have 
\bse
&&\T_1(\bb^*) \\
&=&E\left(\frac{\partial[\S^*_{\bb}(W_i, Y_i, \bb)
    -E^*\{\a(X, \bb) \mid Y_i, W_i,
\bb\}]}{\partial \bb\trans}\bigg |_{\B_r(\cdot)\trans\bb =
m(\cdot)}\right)\{1 + o_p(1)\}.
\ese
Therefore, we can write 
\bse 
&&\wh{\bb} - \bb_0\\
&=& -E\left(\frac{\partial[\S^*_{\bb}(W_i, Y_i, \bb) 
    -E^*\{\a(X, \bb) \mid Y_i, W_i,
\bb\}]}{\partial \bb\trans}\bigg |_{\B_r(\cdot)\trans\bb =
m(\cdot)}\right)^{-1}\\
&&\times\T_{00}\{1 + o_p(1)\}. 
\ese
This proves the results.\qed

\begin{figure}[!h]
\caption{B-spline MLE density estimation (left) and deconvolution
  estimation (right) from 200  simulations: The solid
  lines represent the true functions and the 
  dash lines represent the estimated functions and their 90\%
  confidence bands. The first row to third row are the results for
  model II (a)--(c) respectively. Sample size 1000.
}
{\label{fig:den2}}
\begin{center}
\includegraphics[scale = 0.35]{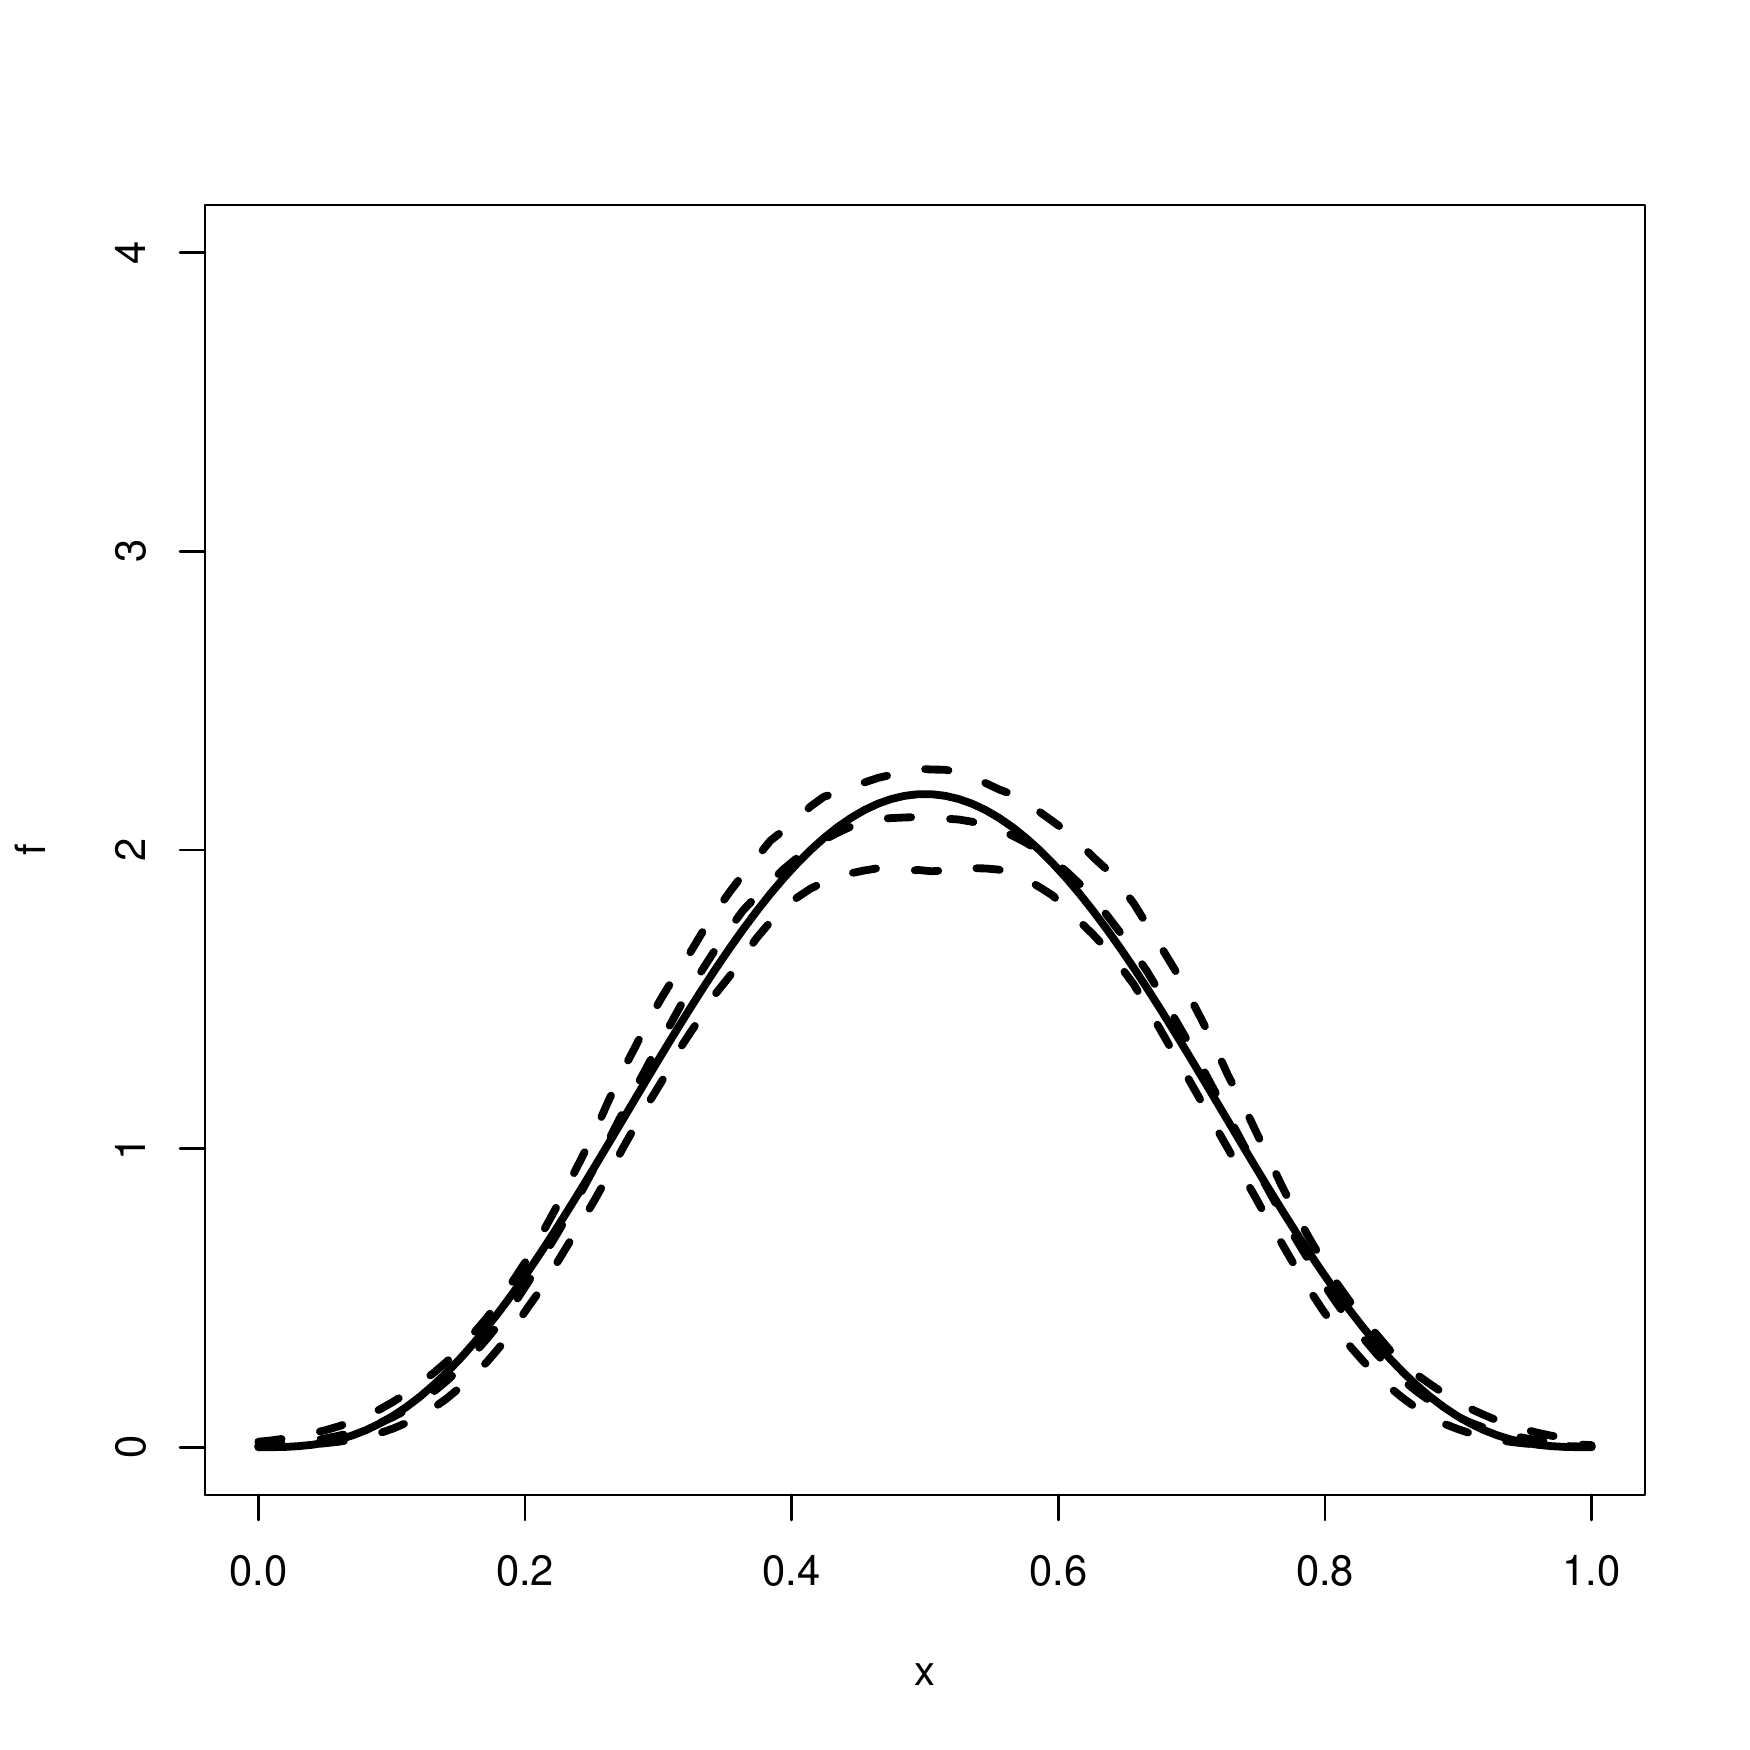}
\includegraphics[scale = 0.35]{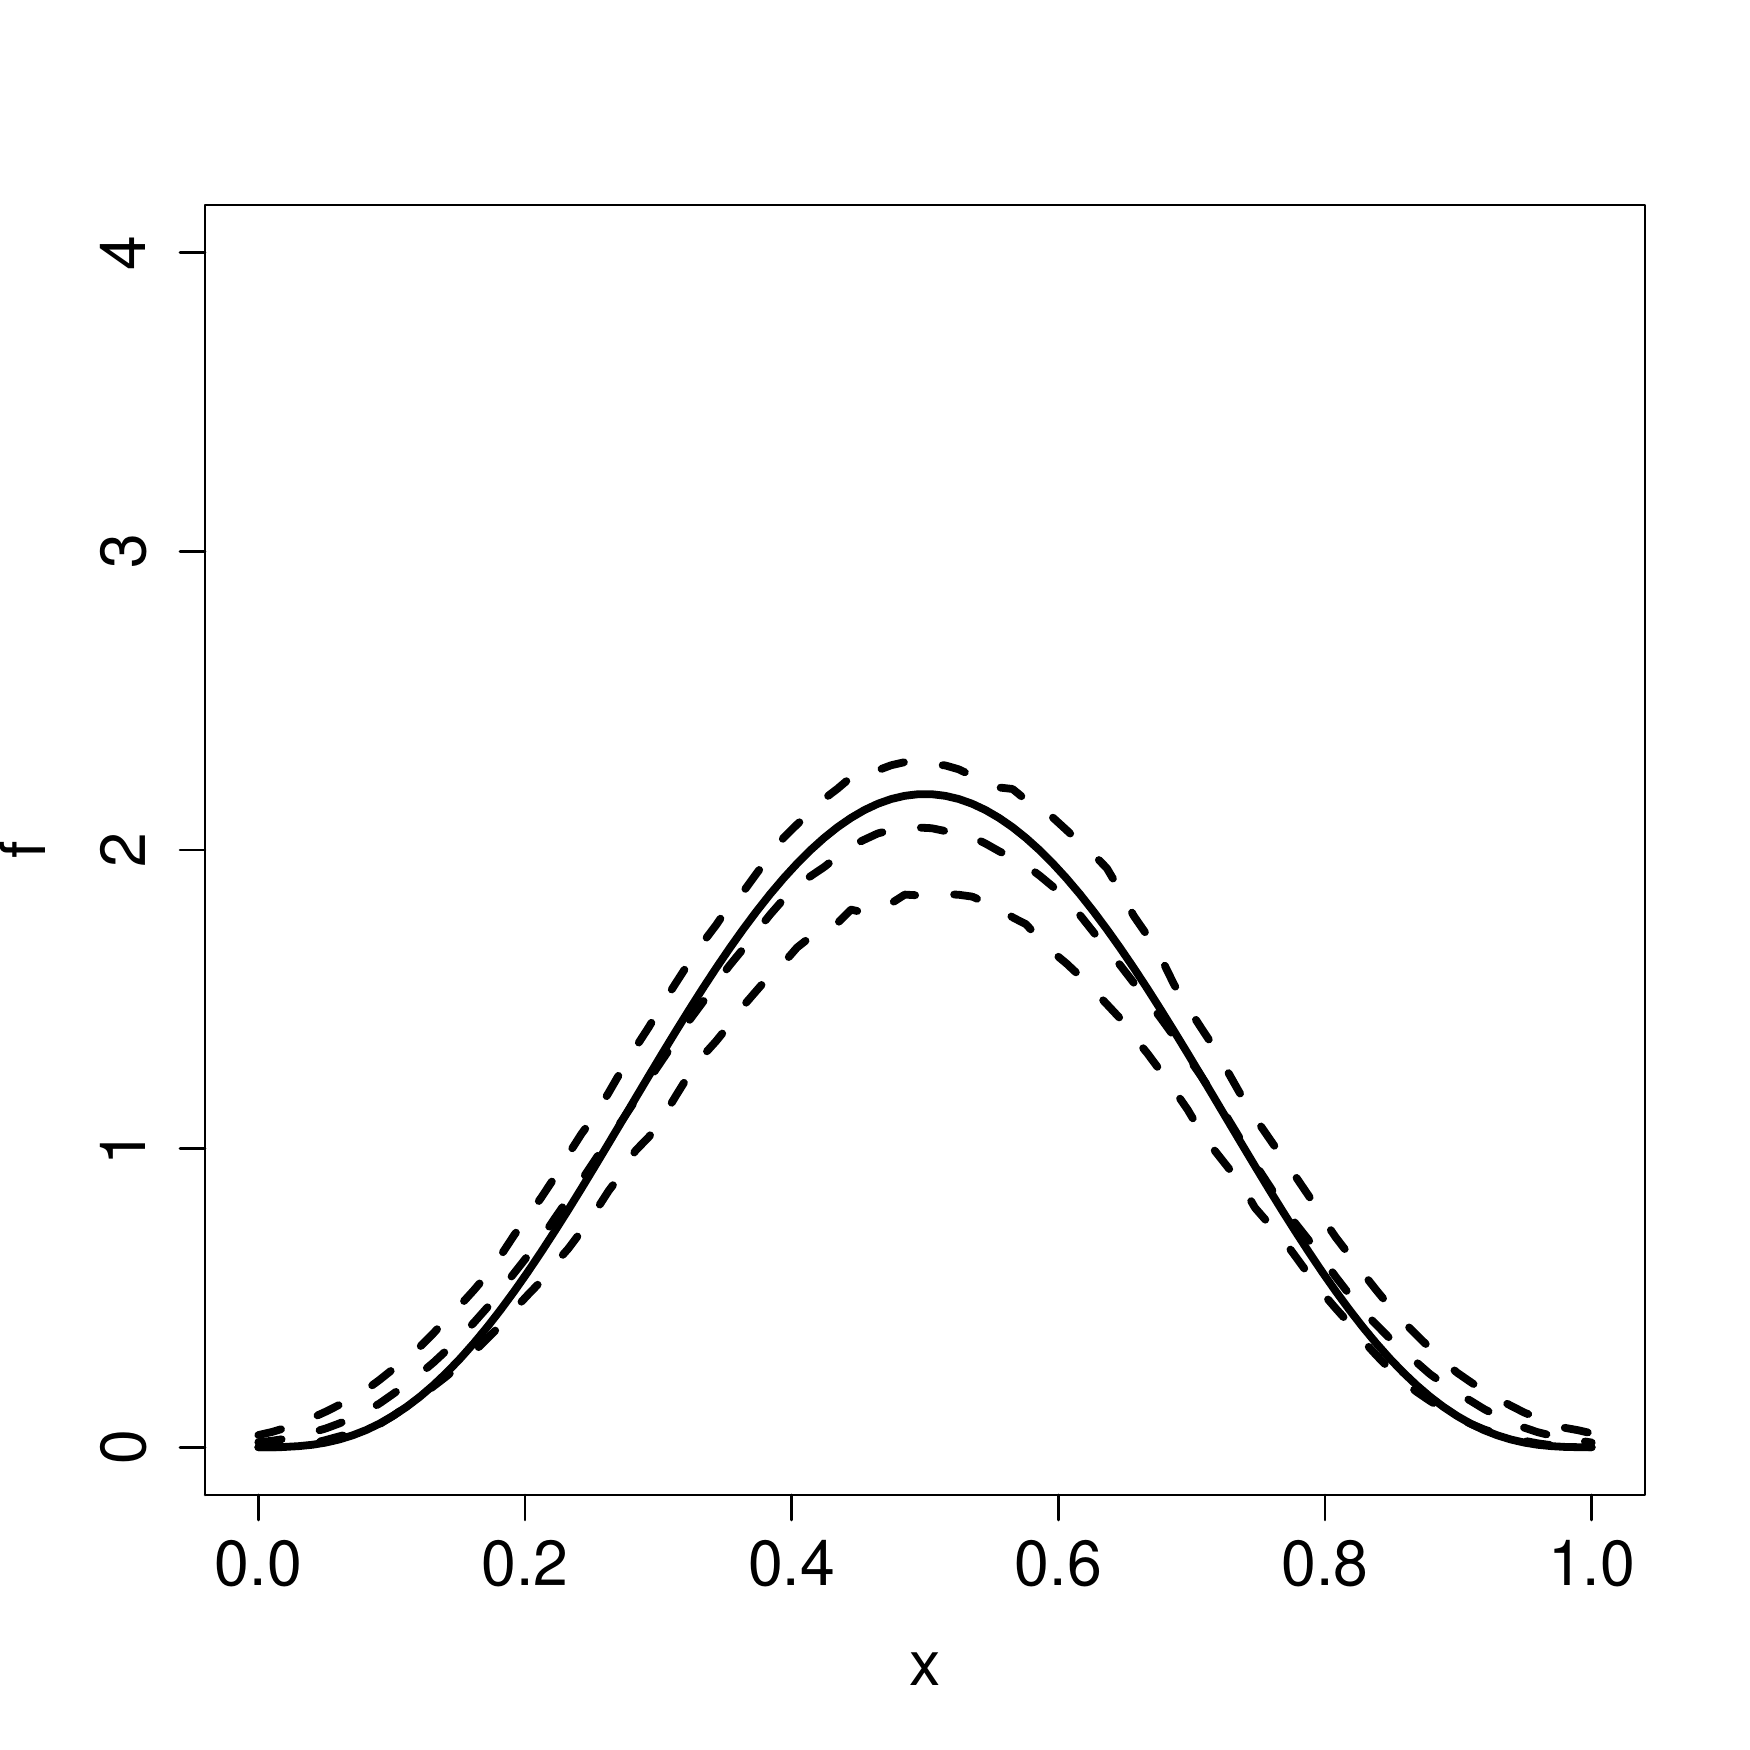}\\
\includegraphics[scale = 0.35]{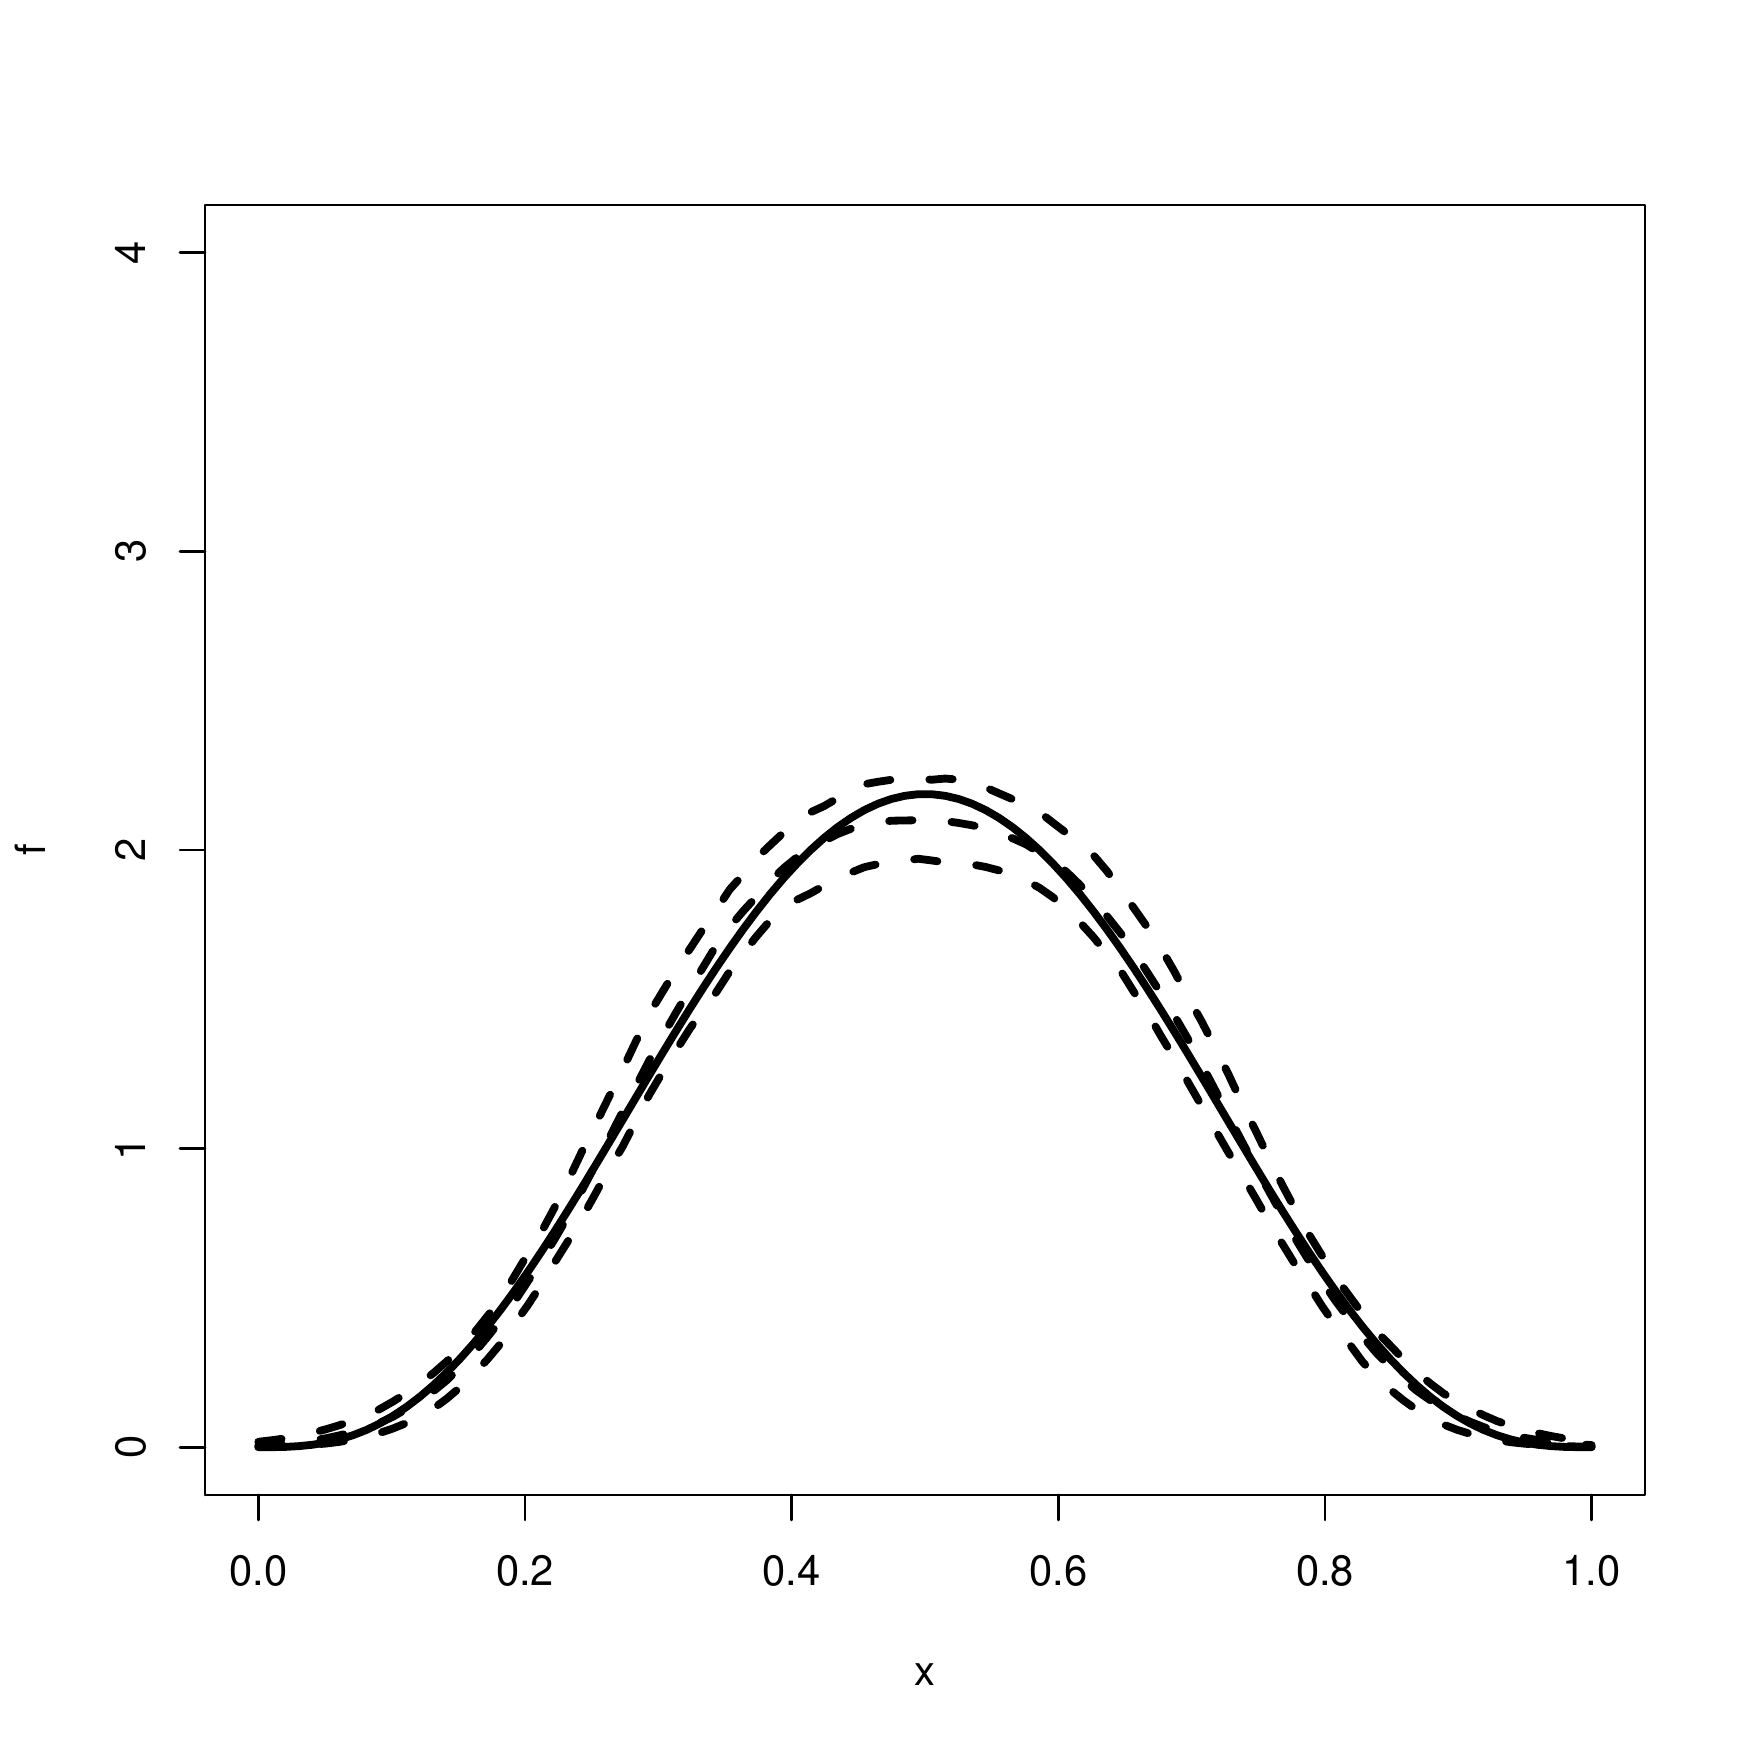}
\includegraphics[scale = 0.35]{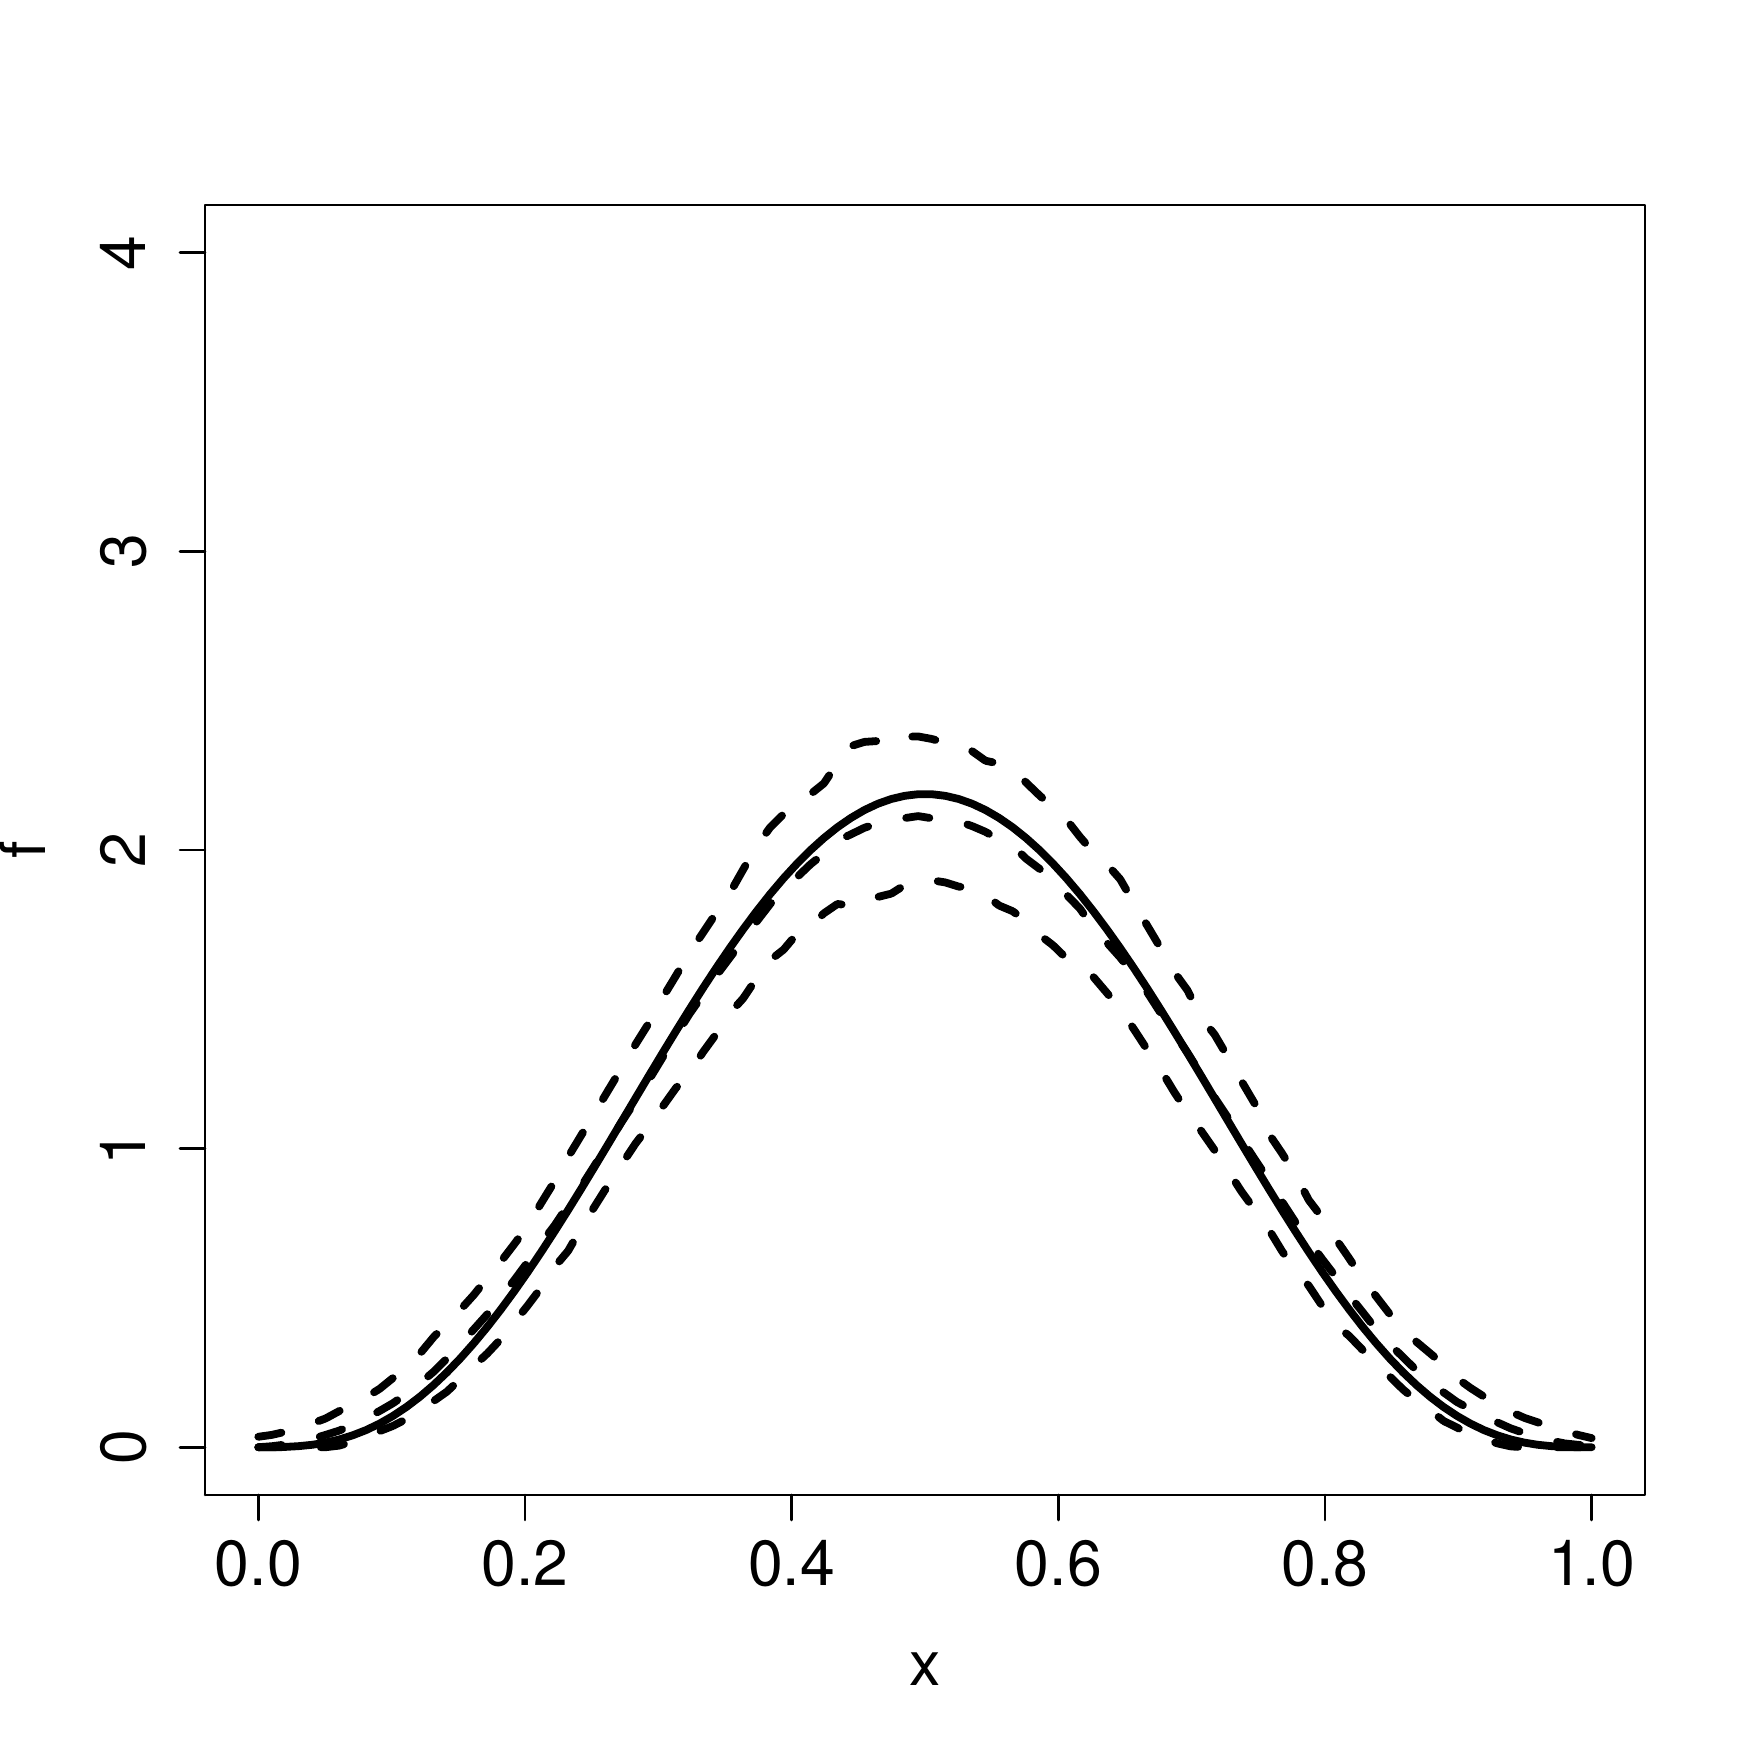}\\
\includegraphics[scale = 0.35]{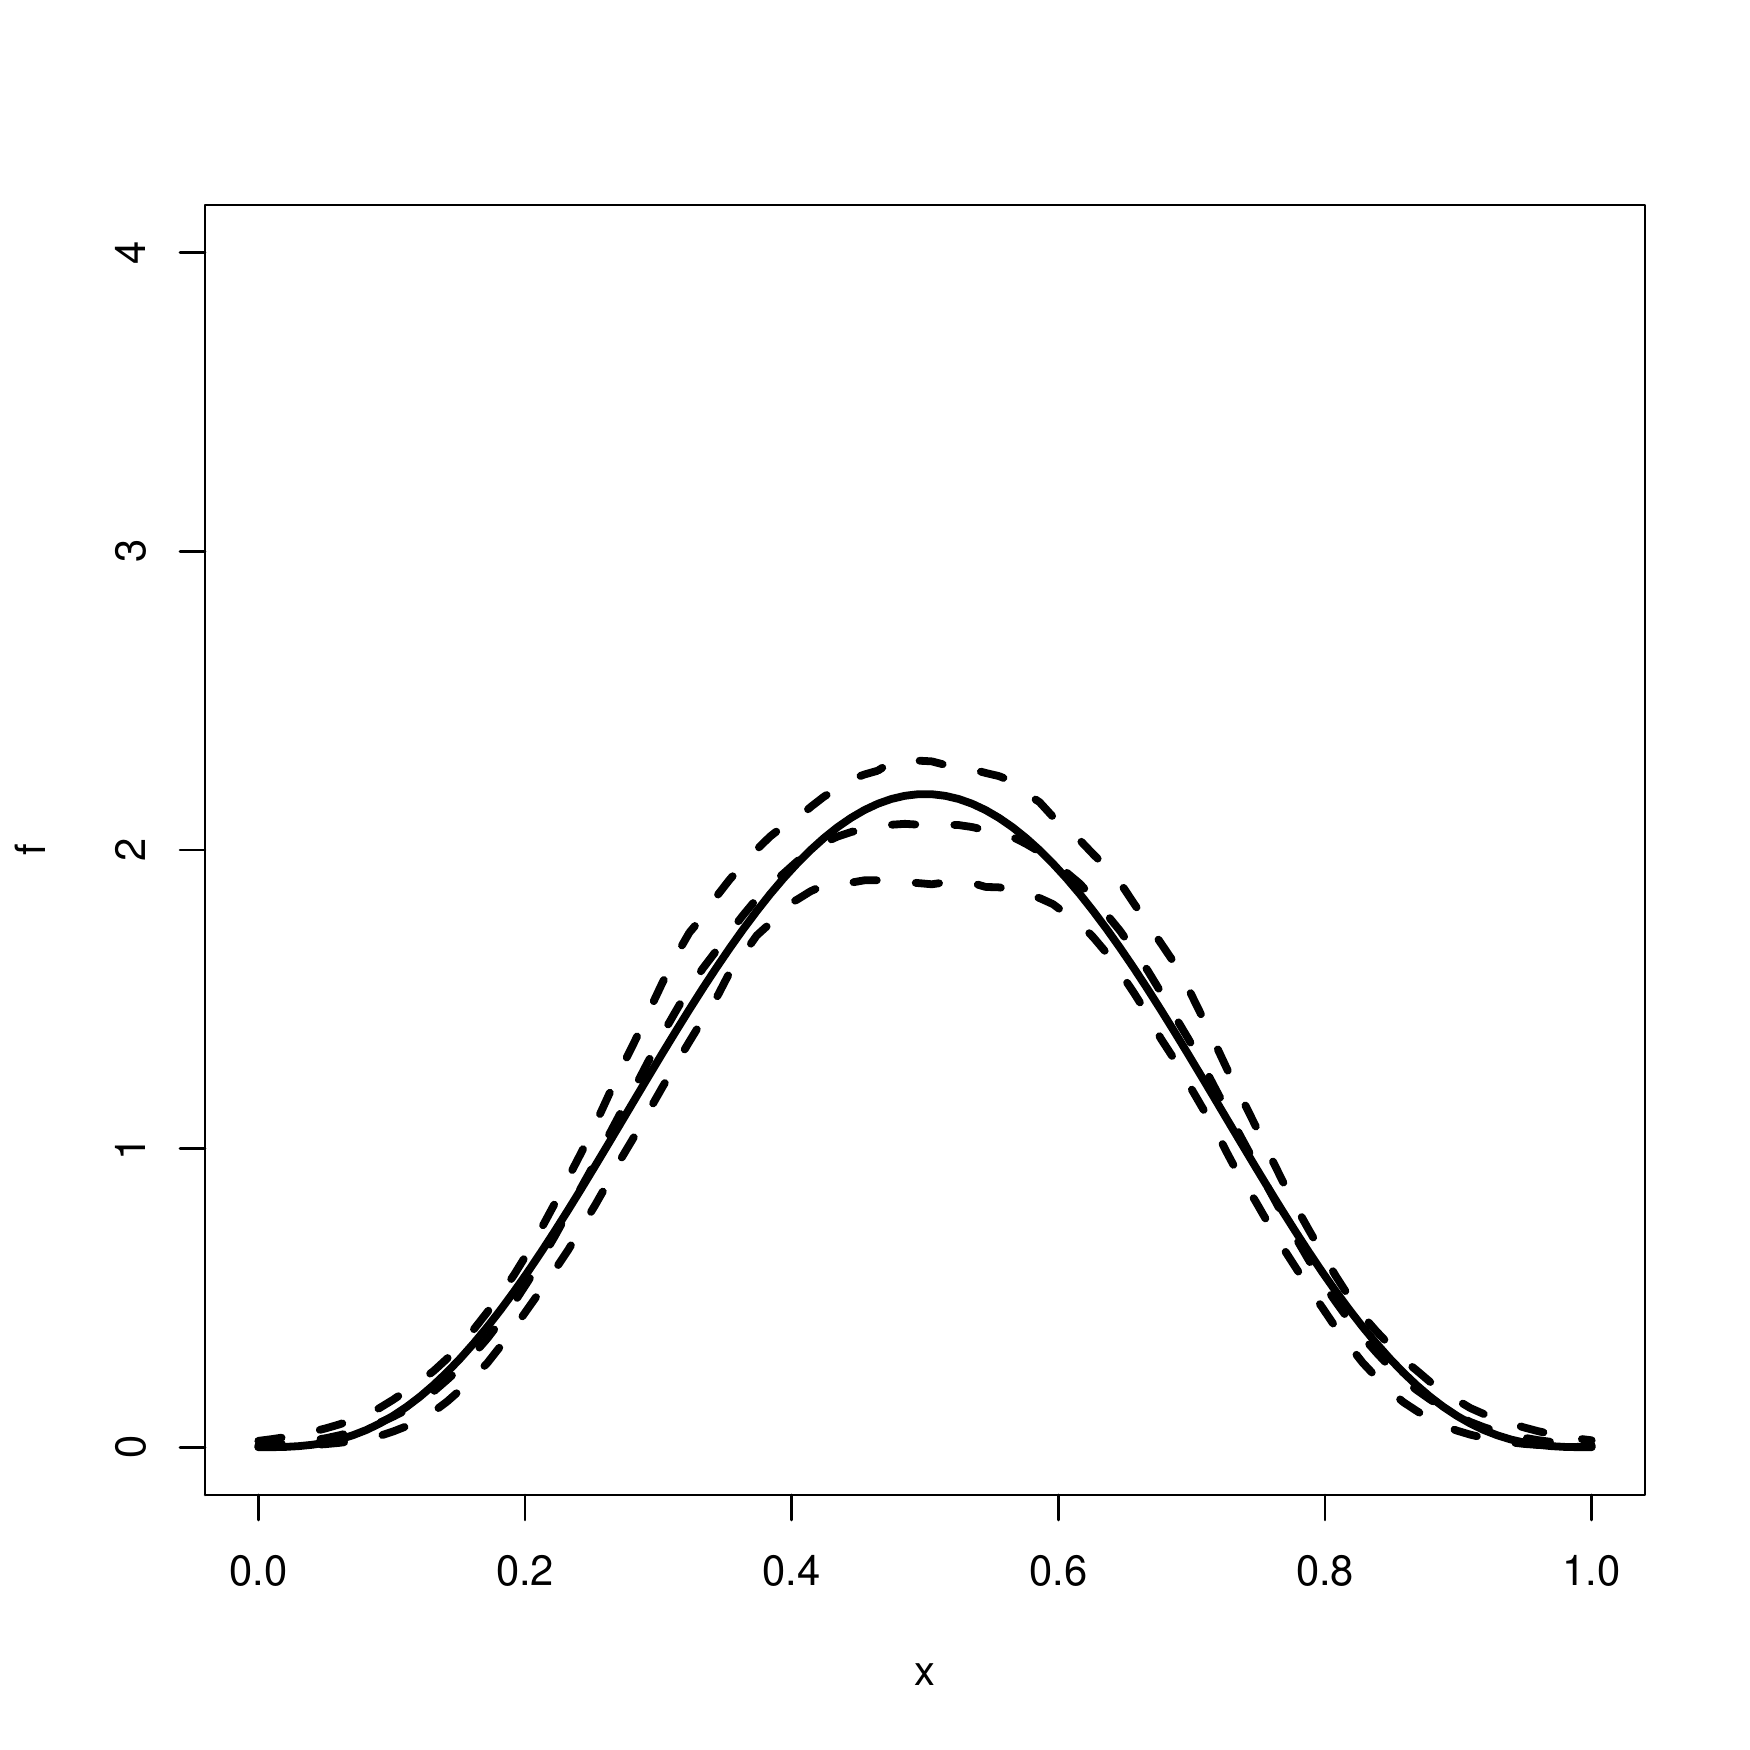}
\includegraphics[scale = 0.35]{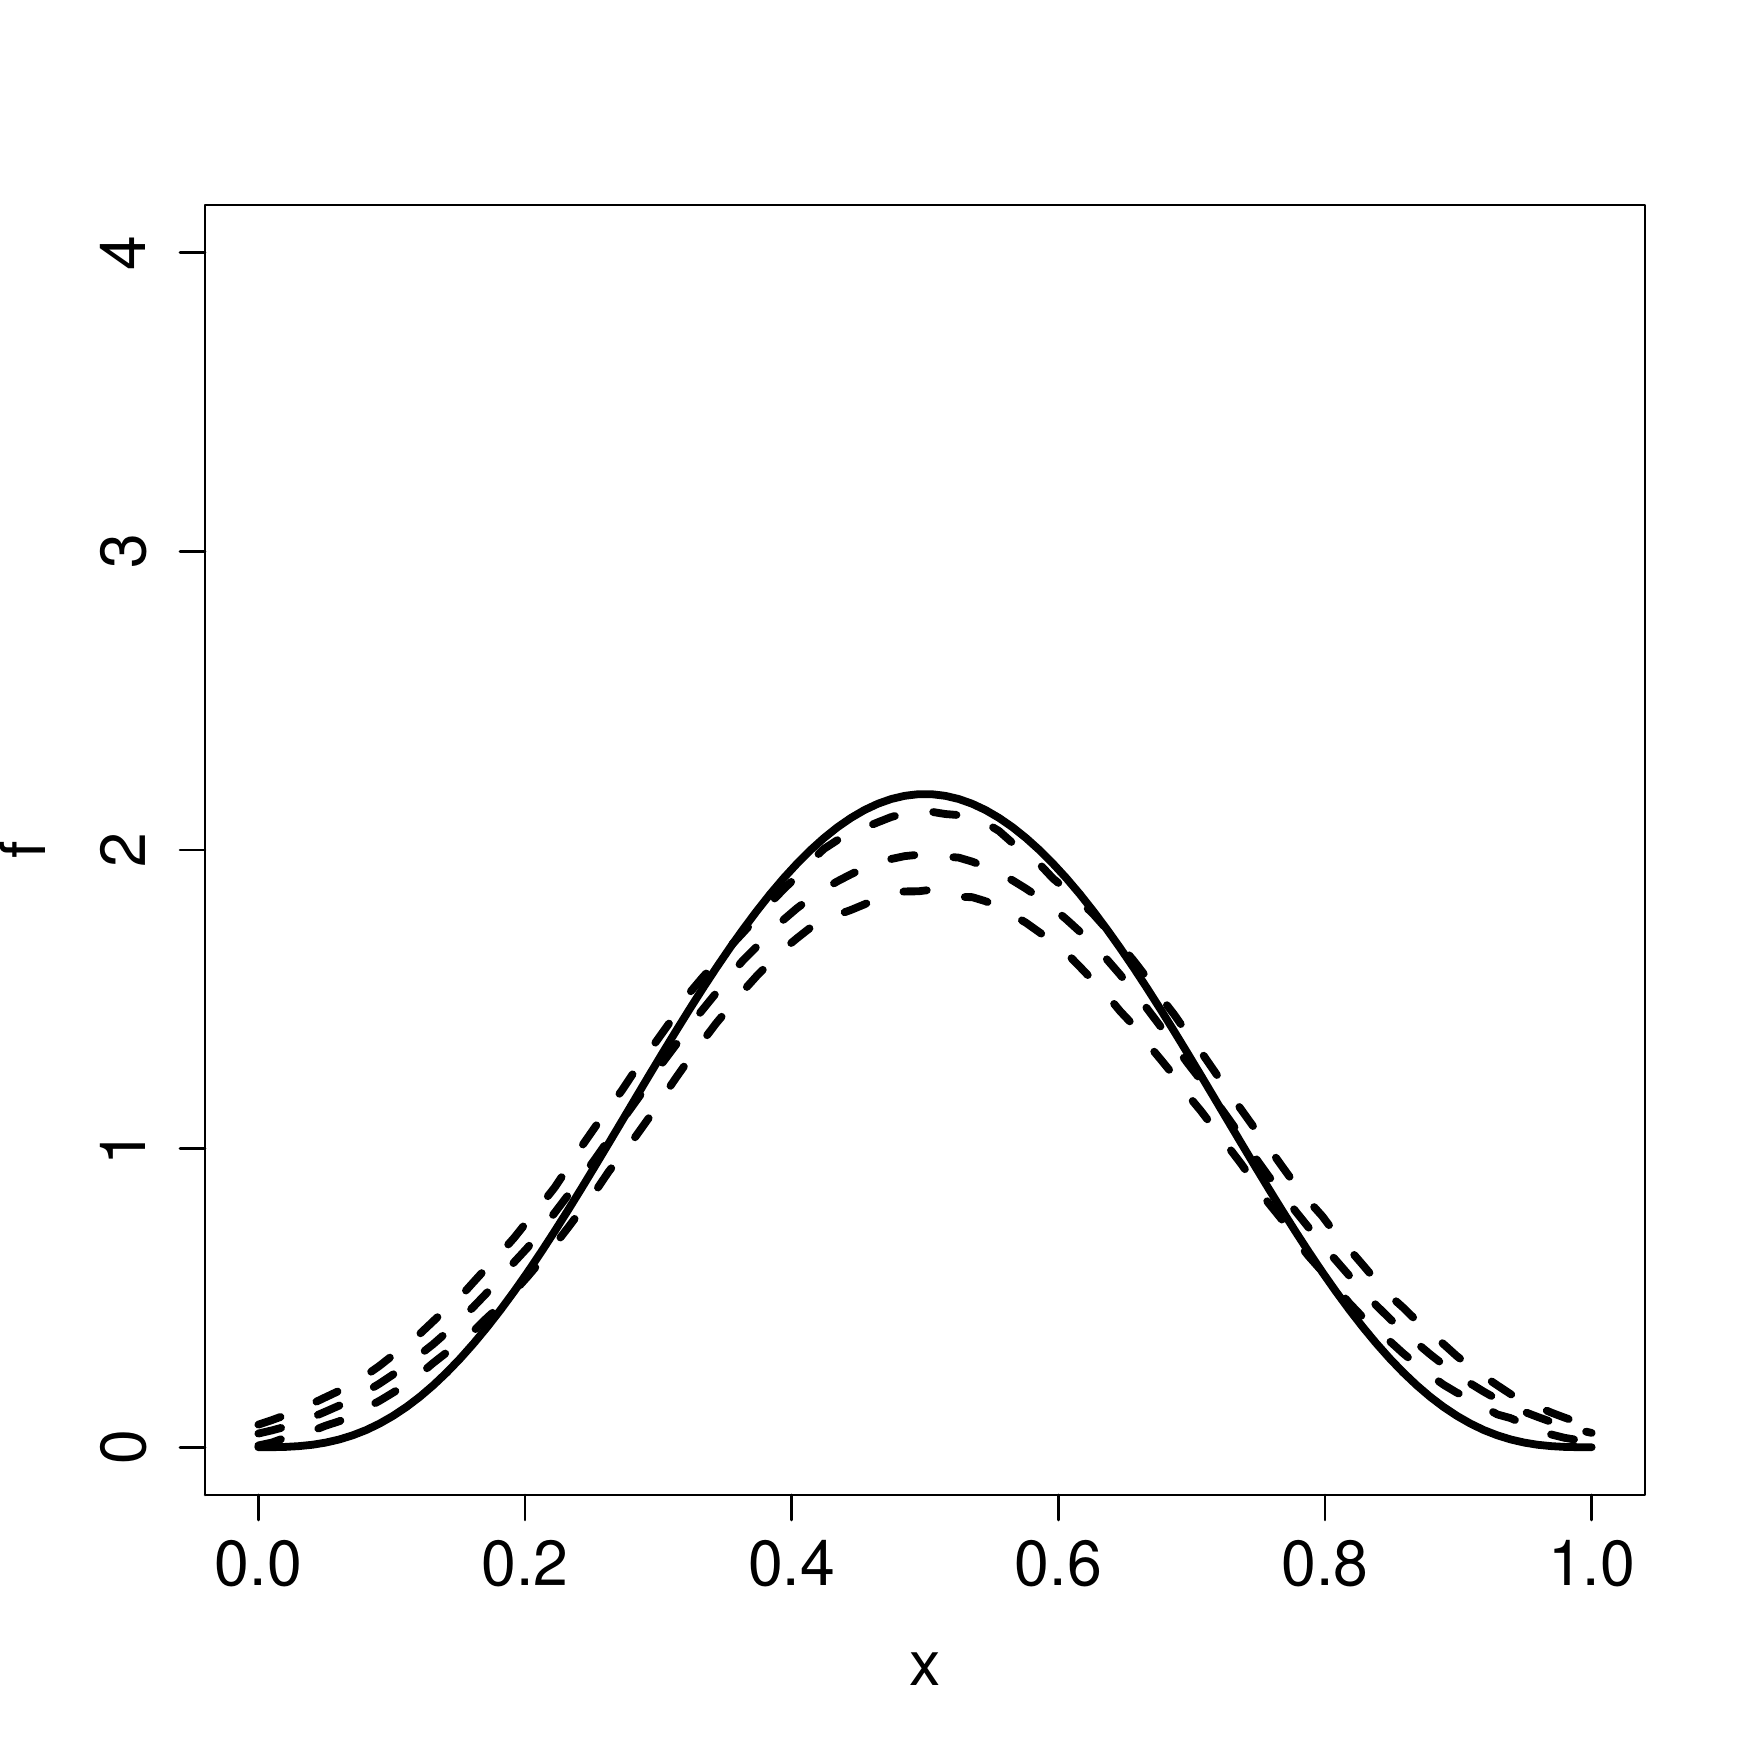}
\end{center}
\end{figure}

\begin{figure}[!h]
\caption{B-spline MLE density estimation (left) and deconvolution
  estimation (right) from 200  simulations: The solid
  lines represent the true functions and the 
  dash lines represent the estimated functions and their 90\%
  confidence bands. The first row to third row are the results for
  model II (a)--(c) respectively. Sample size 2000.
}
{\label{fig:den3}}
\begin{center}
\includegraphics[scale = 0.35]{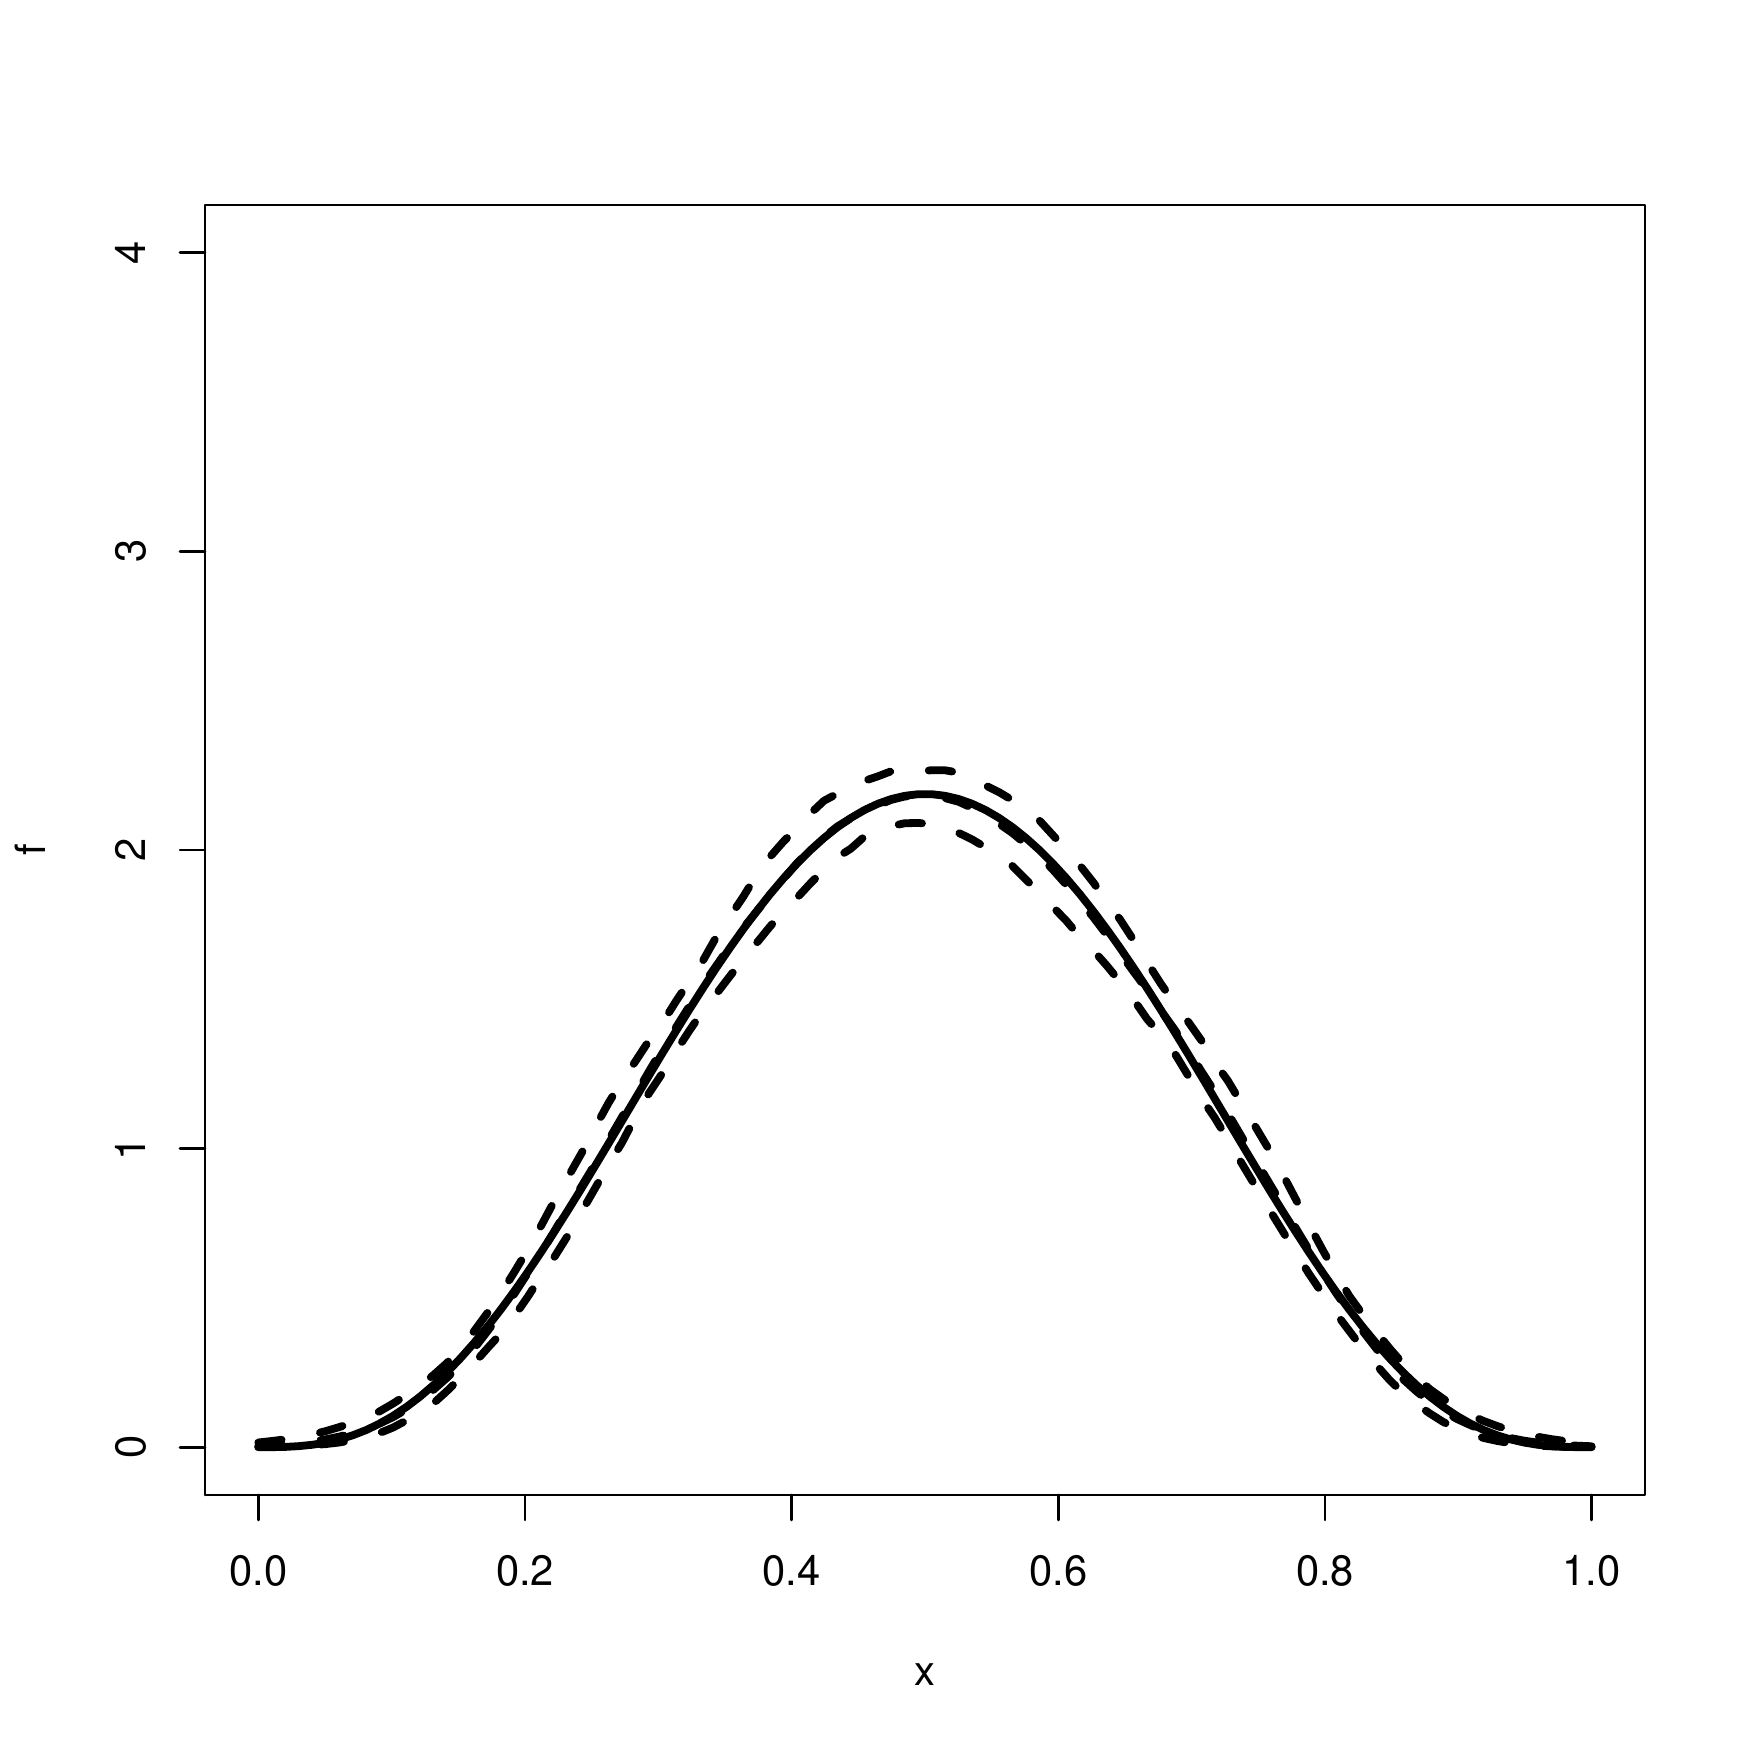}
\includegraphics[scale = 0.35]{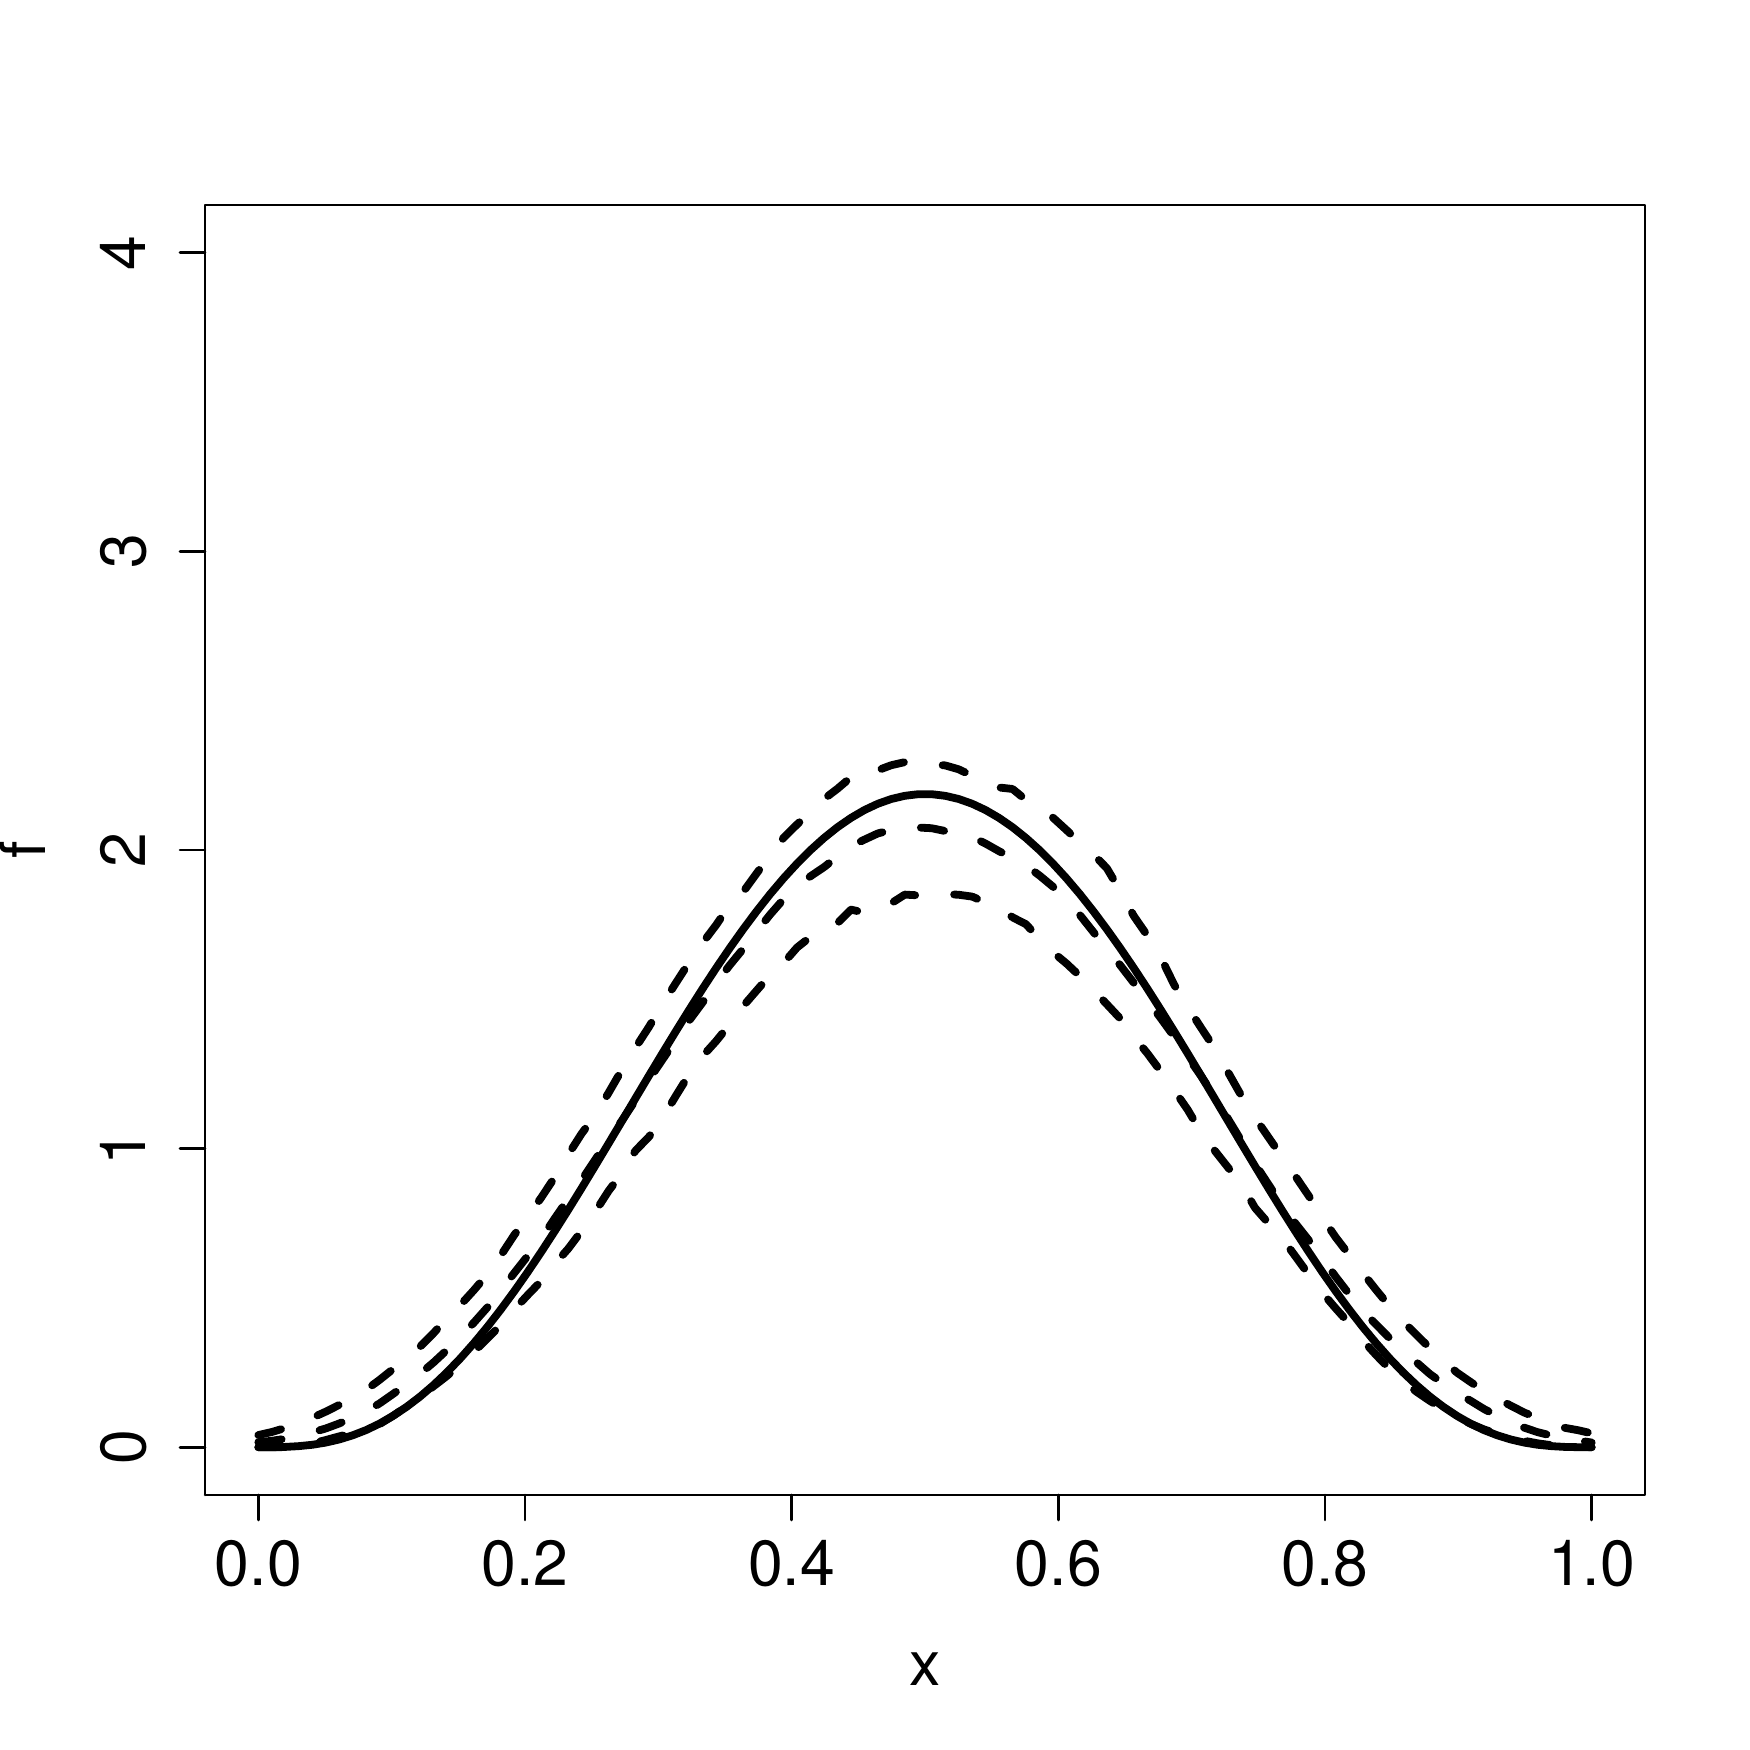}\\
\includegraphics[scale = 0.35]{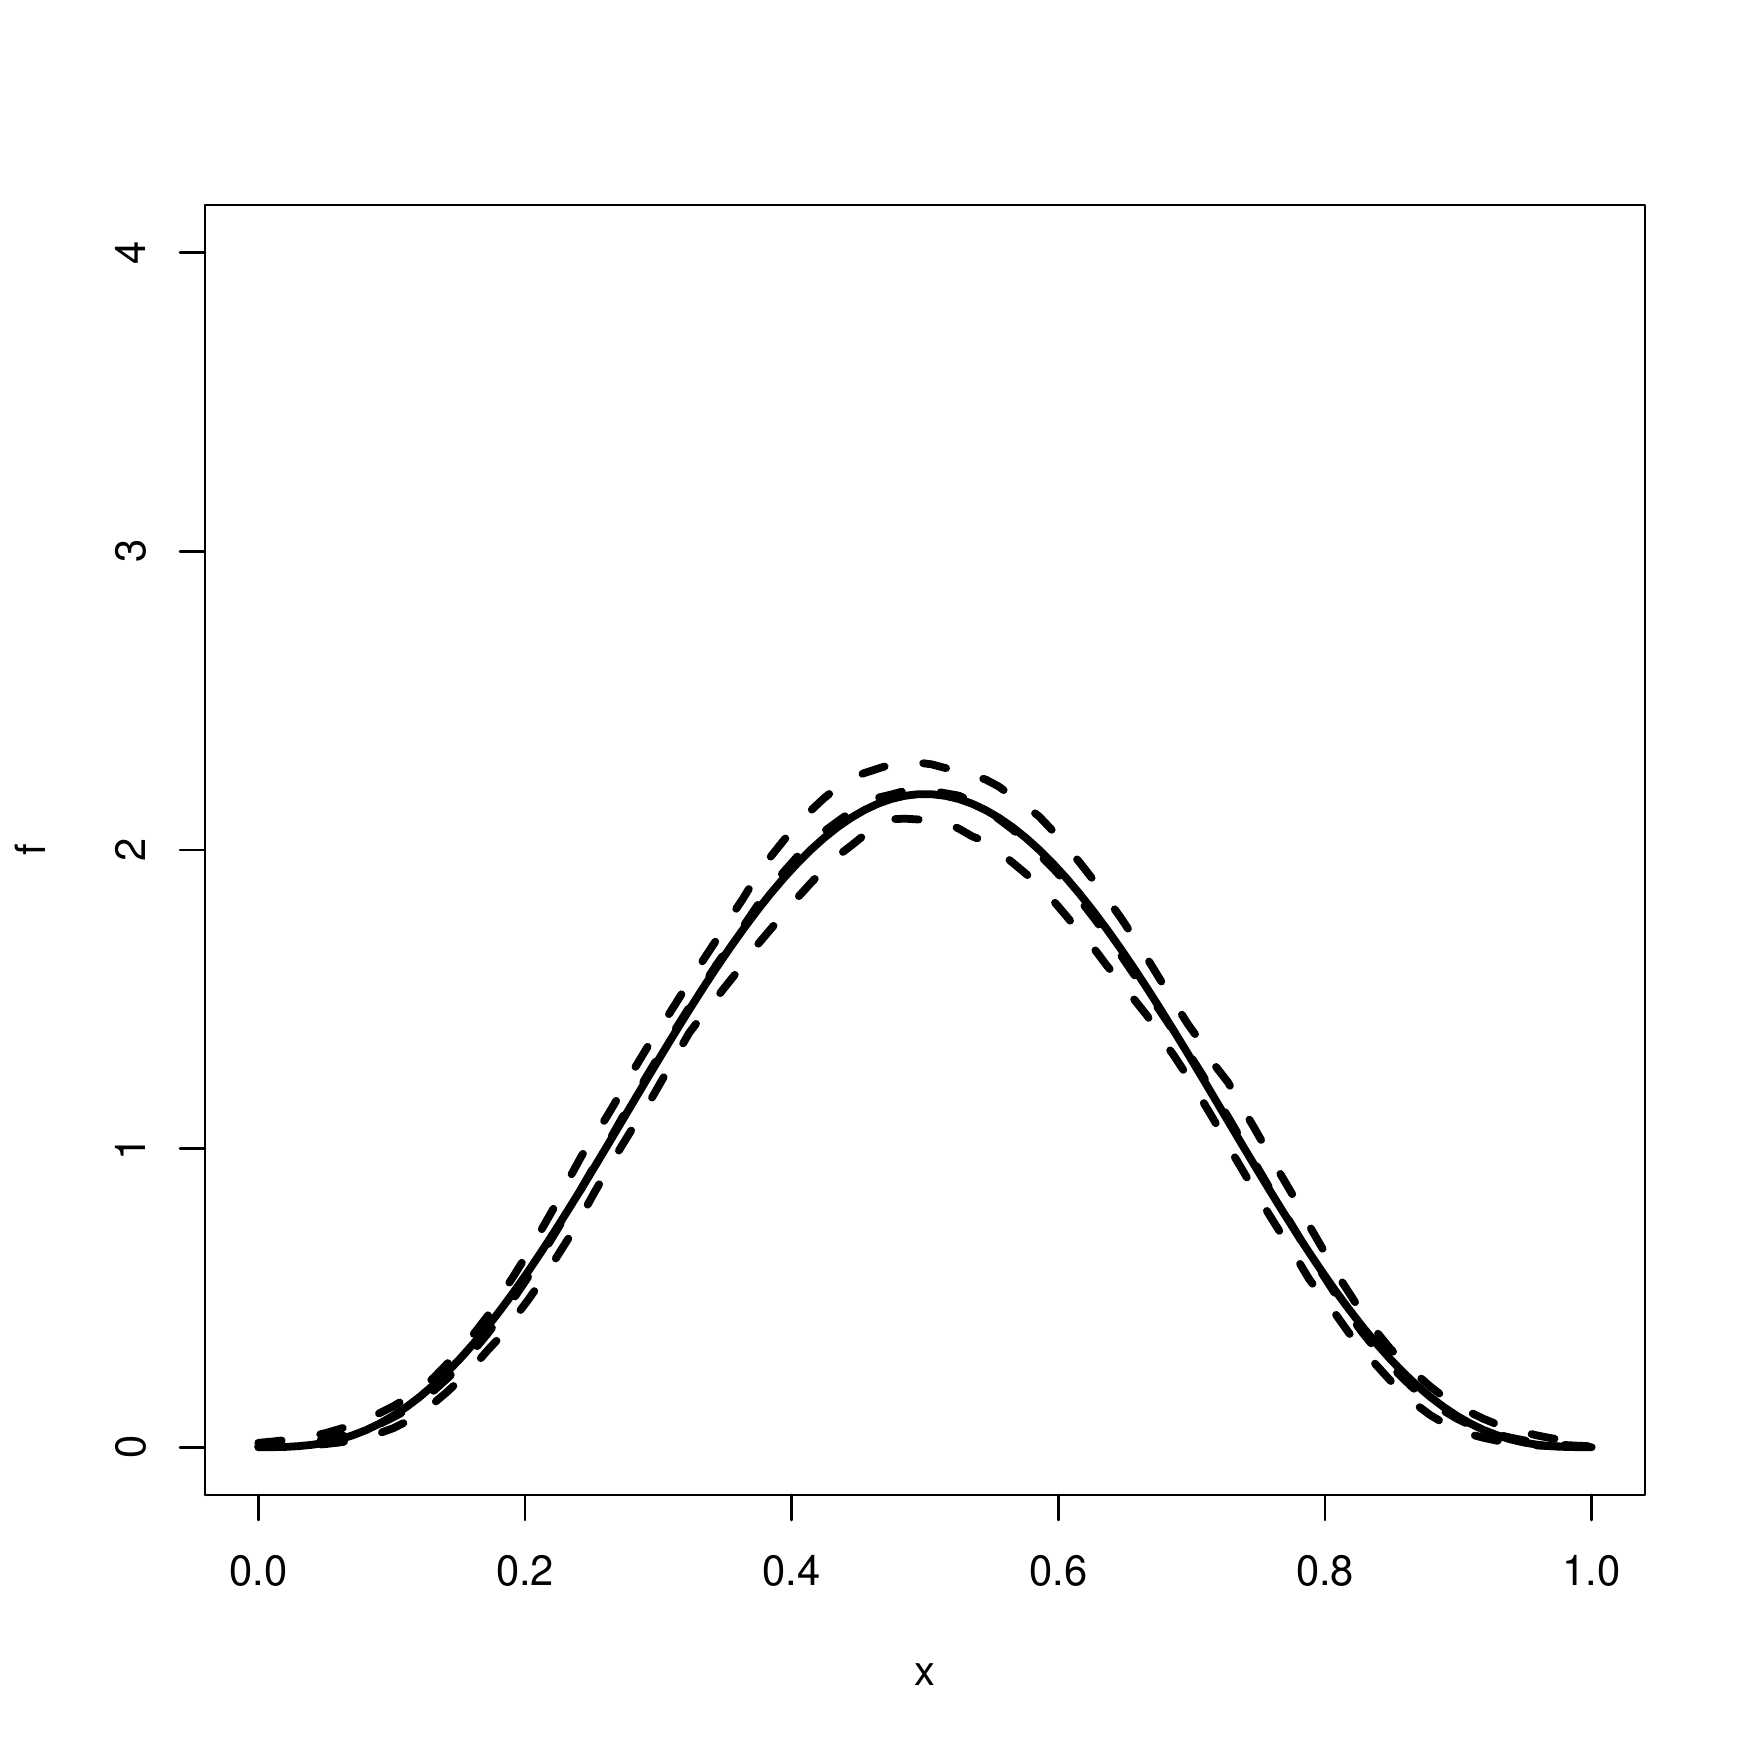}
\includegraphics[scale = 0.35]{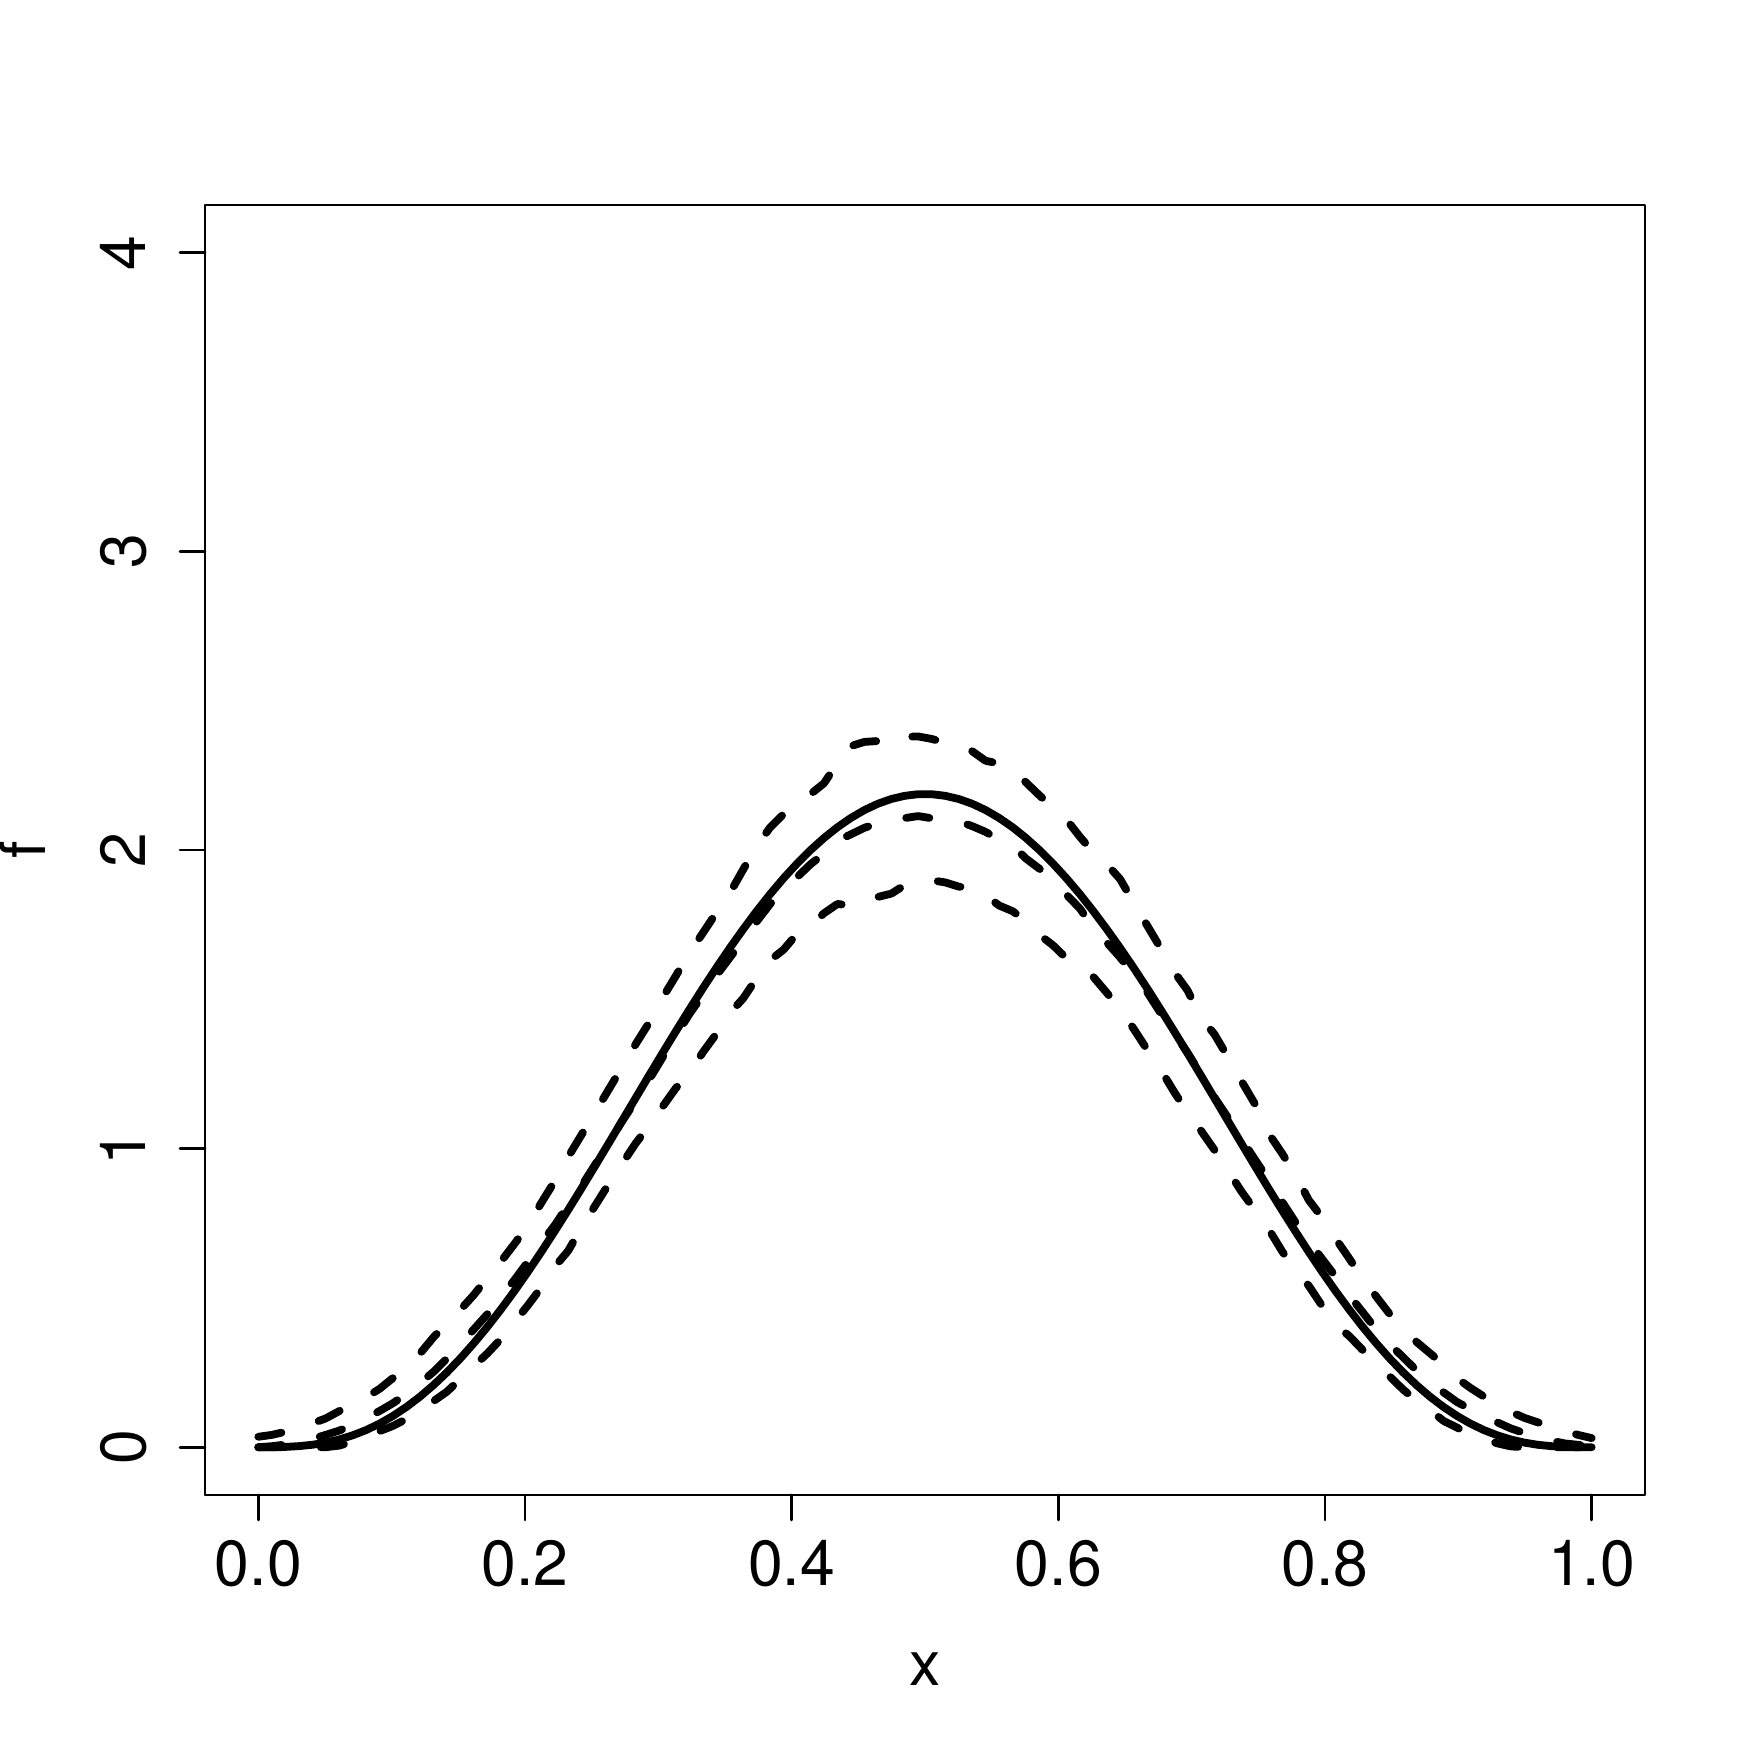}\\
\includegraphics[scale = 0.35]{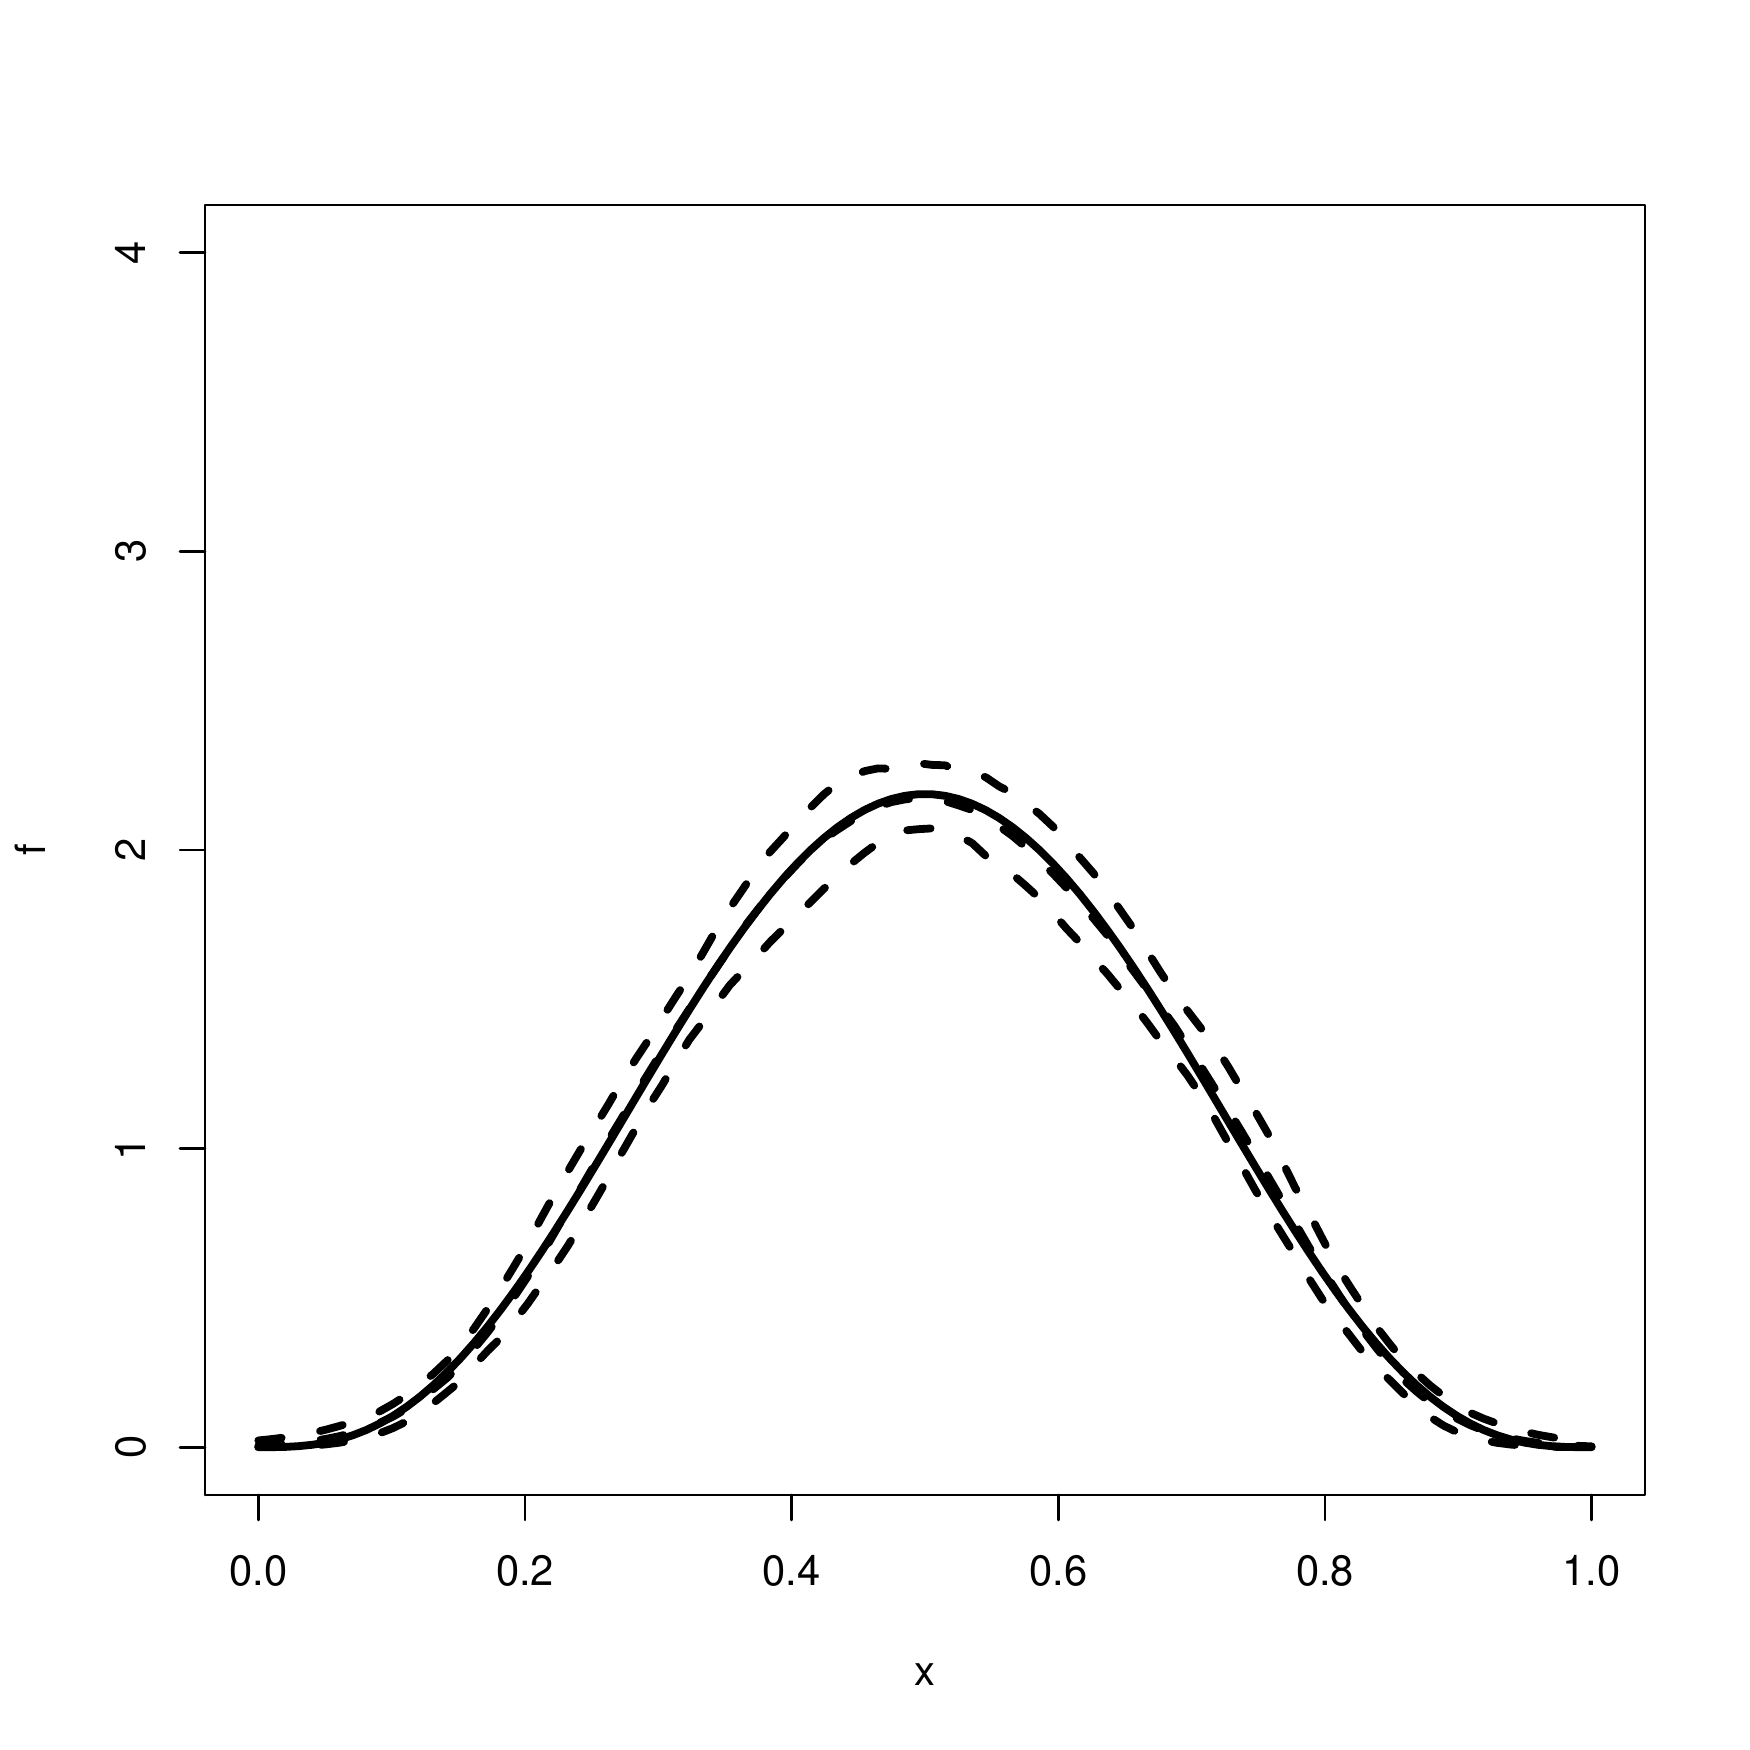}
\includegraphics[scale = 0.35]{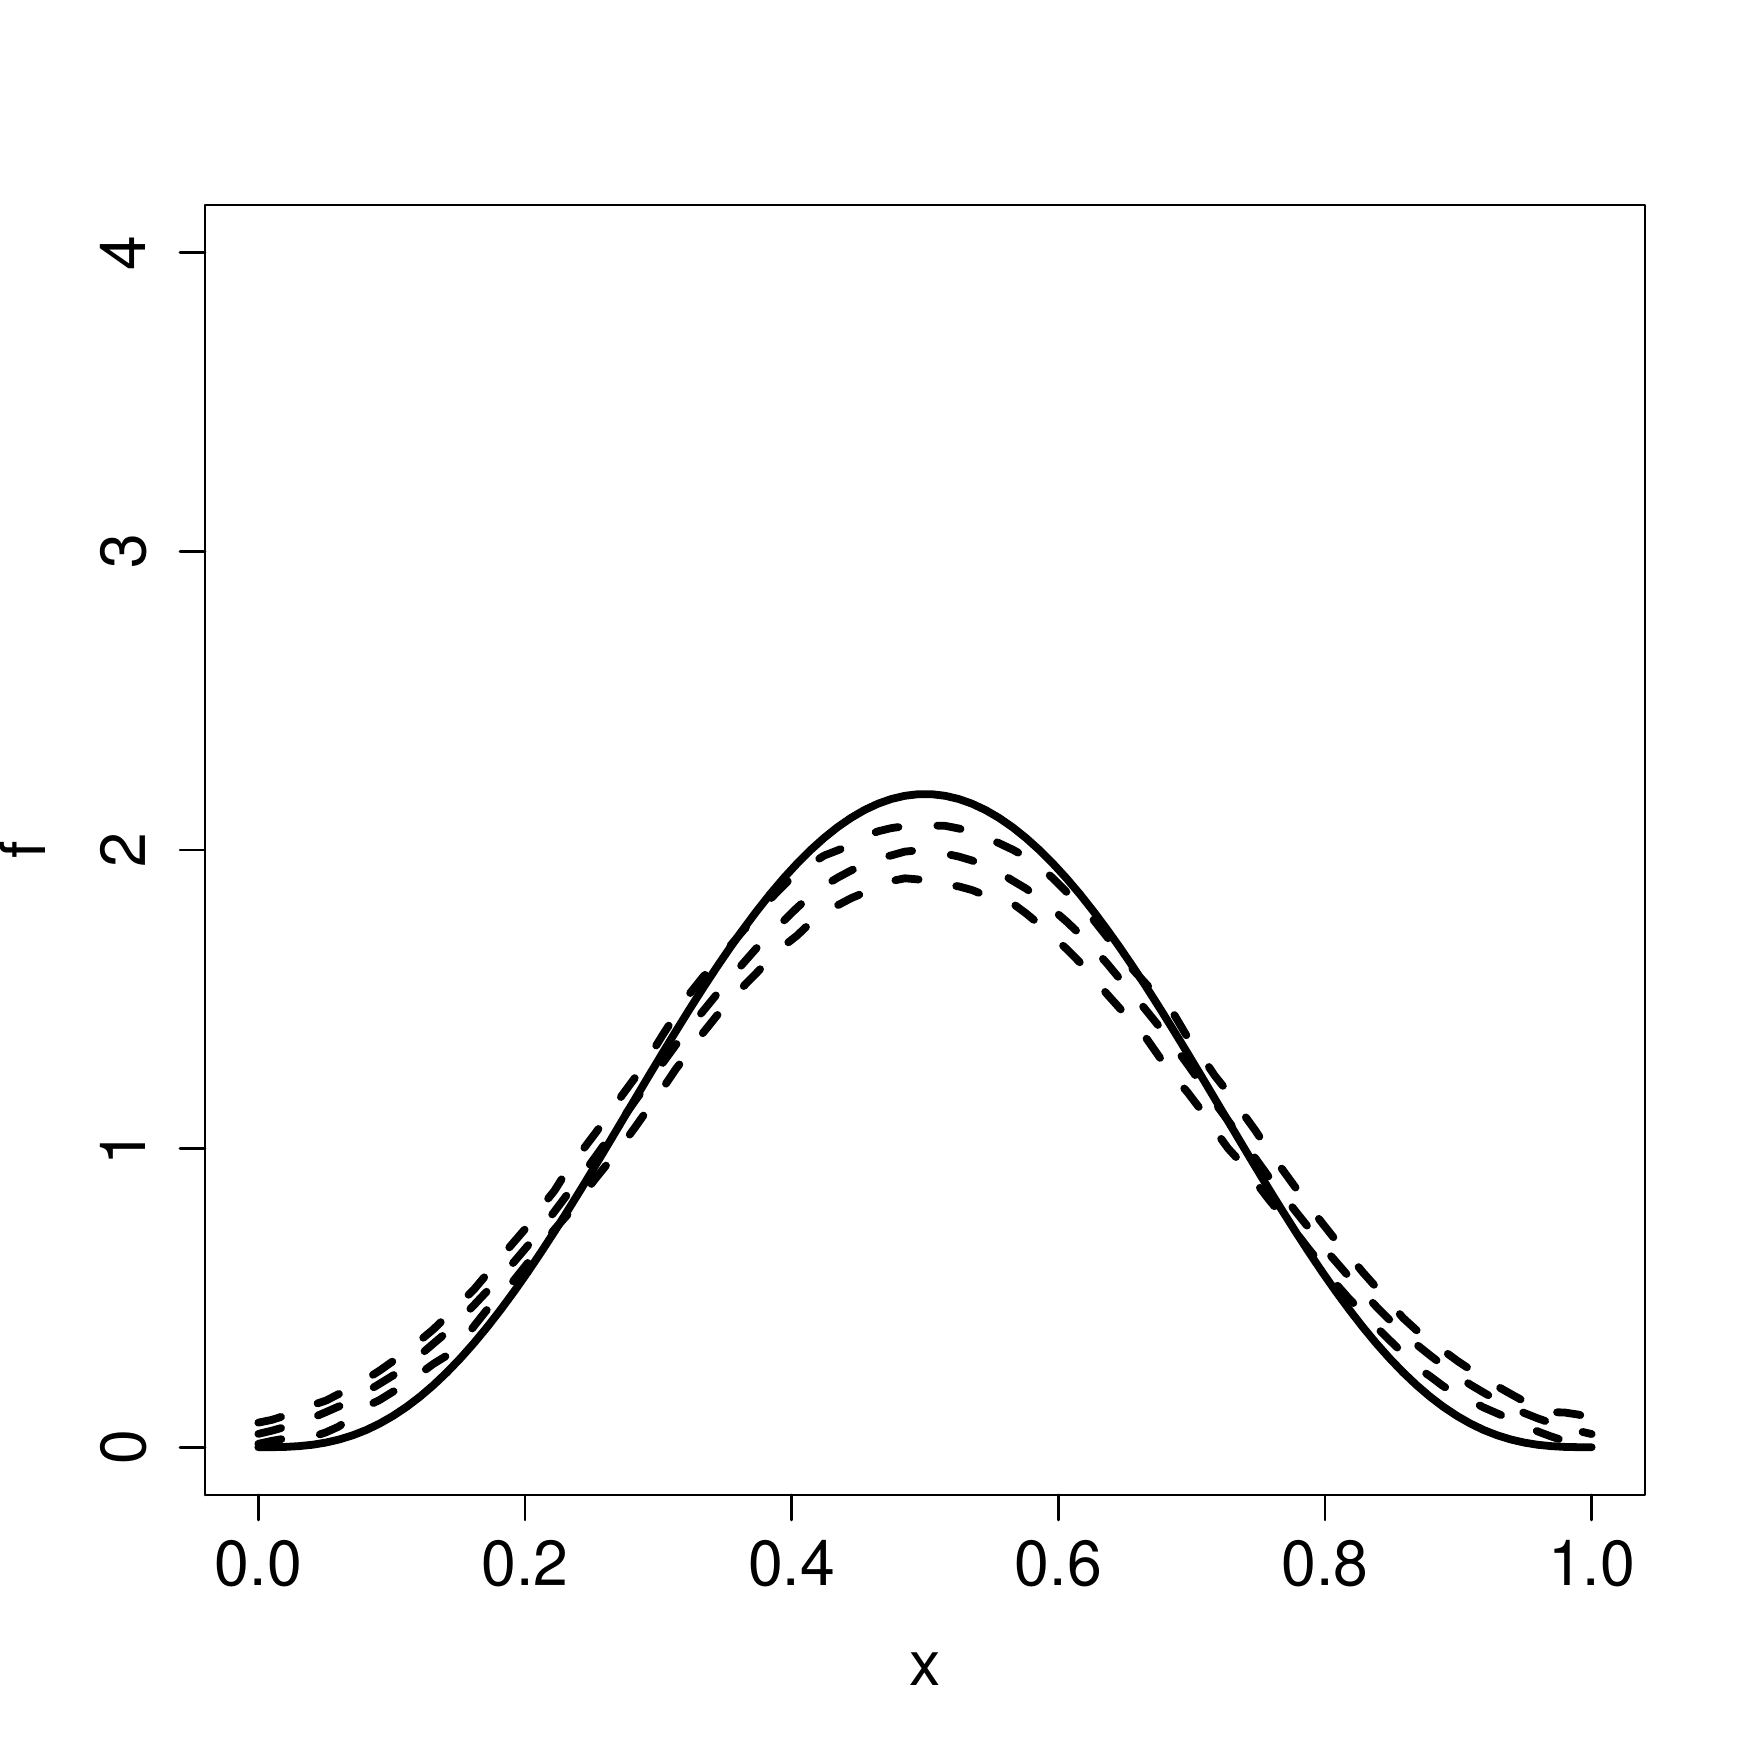}
\end{center}
\end{figure}

\begin{figure}[!h]
\caption{Bspline MLE density estimation (left) and deconvolution 
  estimation (right) from 200  simulations: The solid 
  lines represent the true functions and the 
  dash lines represent the estimated functions and their 90\%
  confidence bands. The first row to third row are the results for 
  model II (a)--(c) respectively. Sample size 200. 
}
{\label{fig:den0}}
\begin{center}
\includegraphics[scale = 0.35]{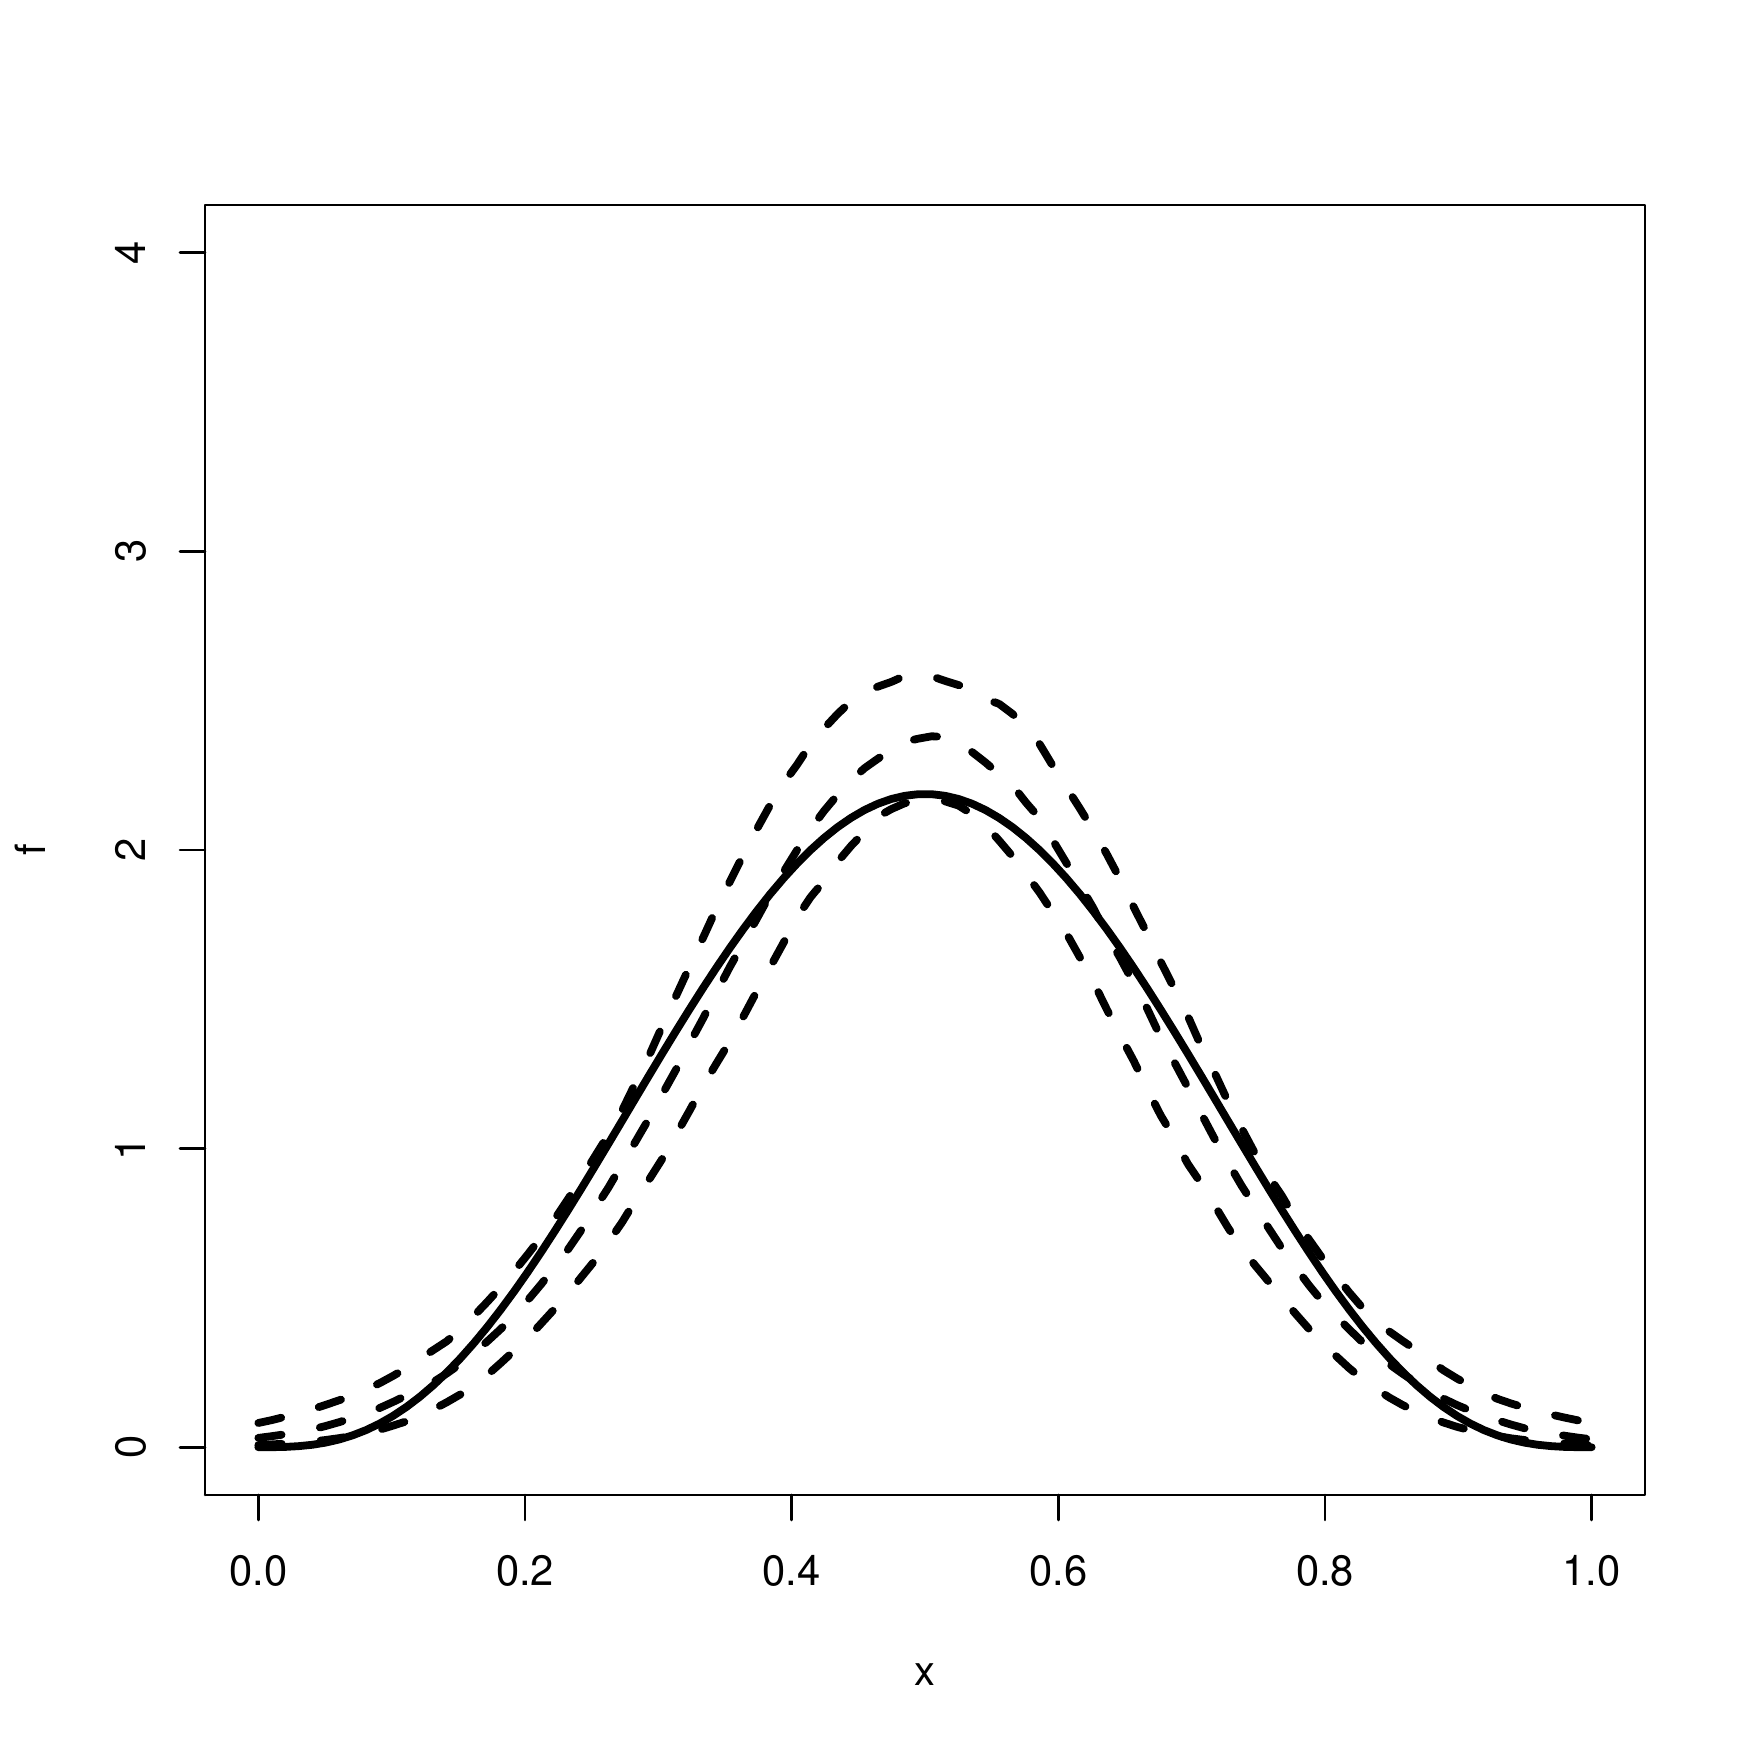}
\includegraphics[scale = 0.35]{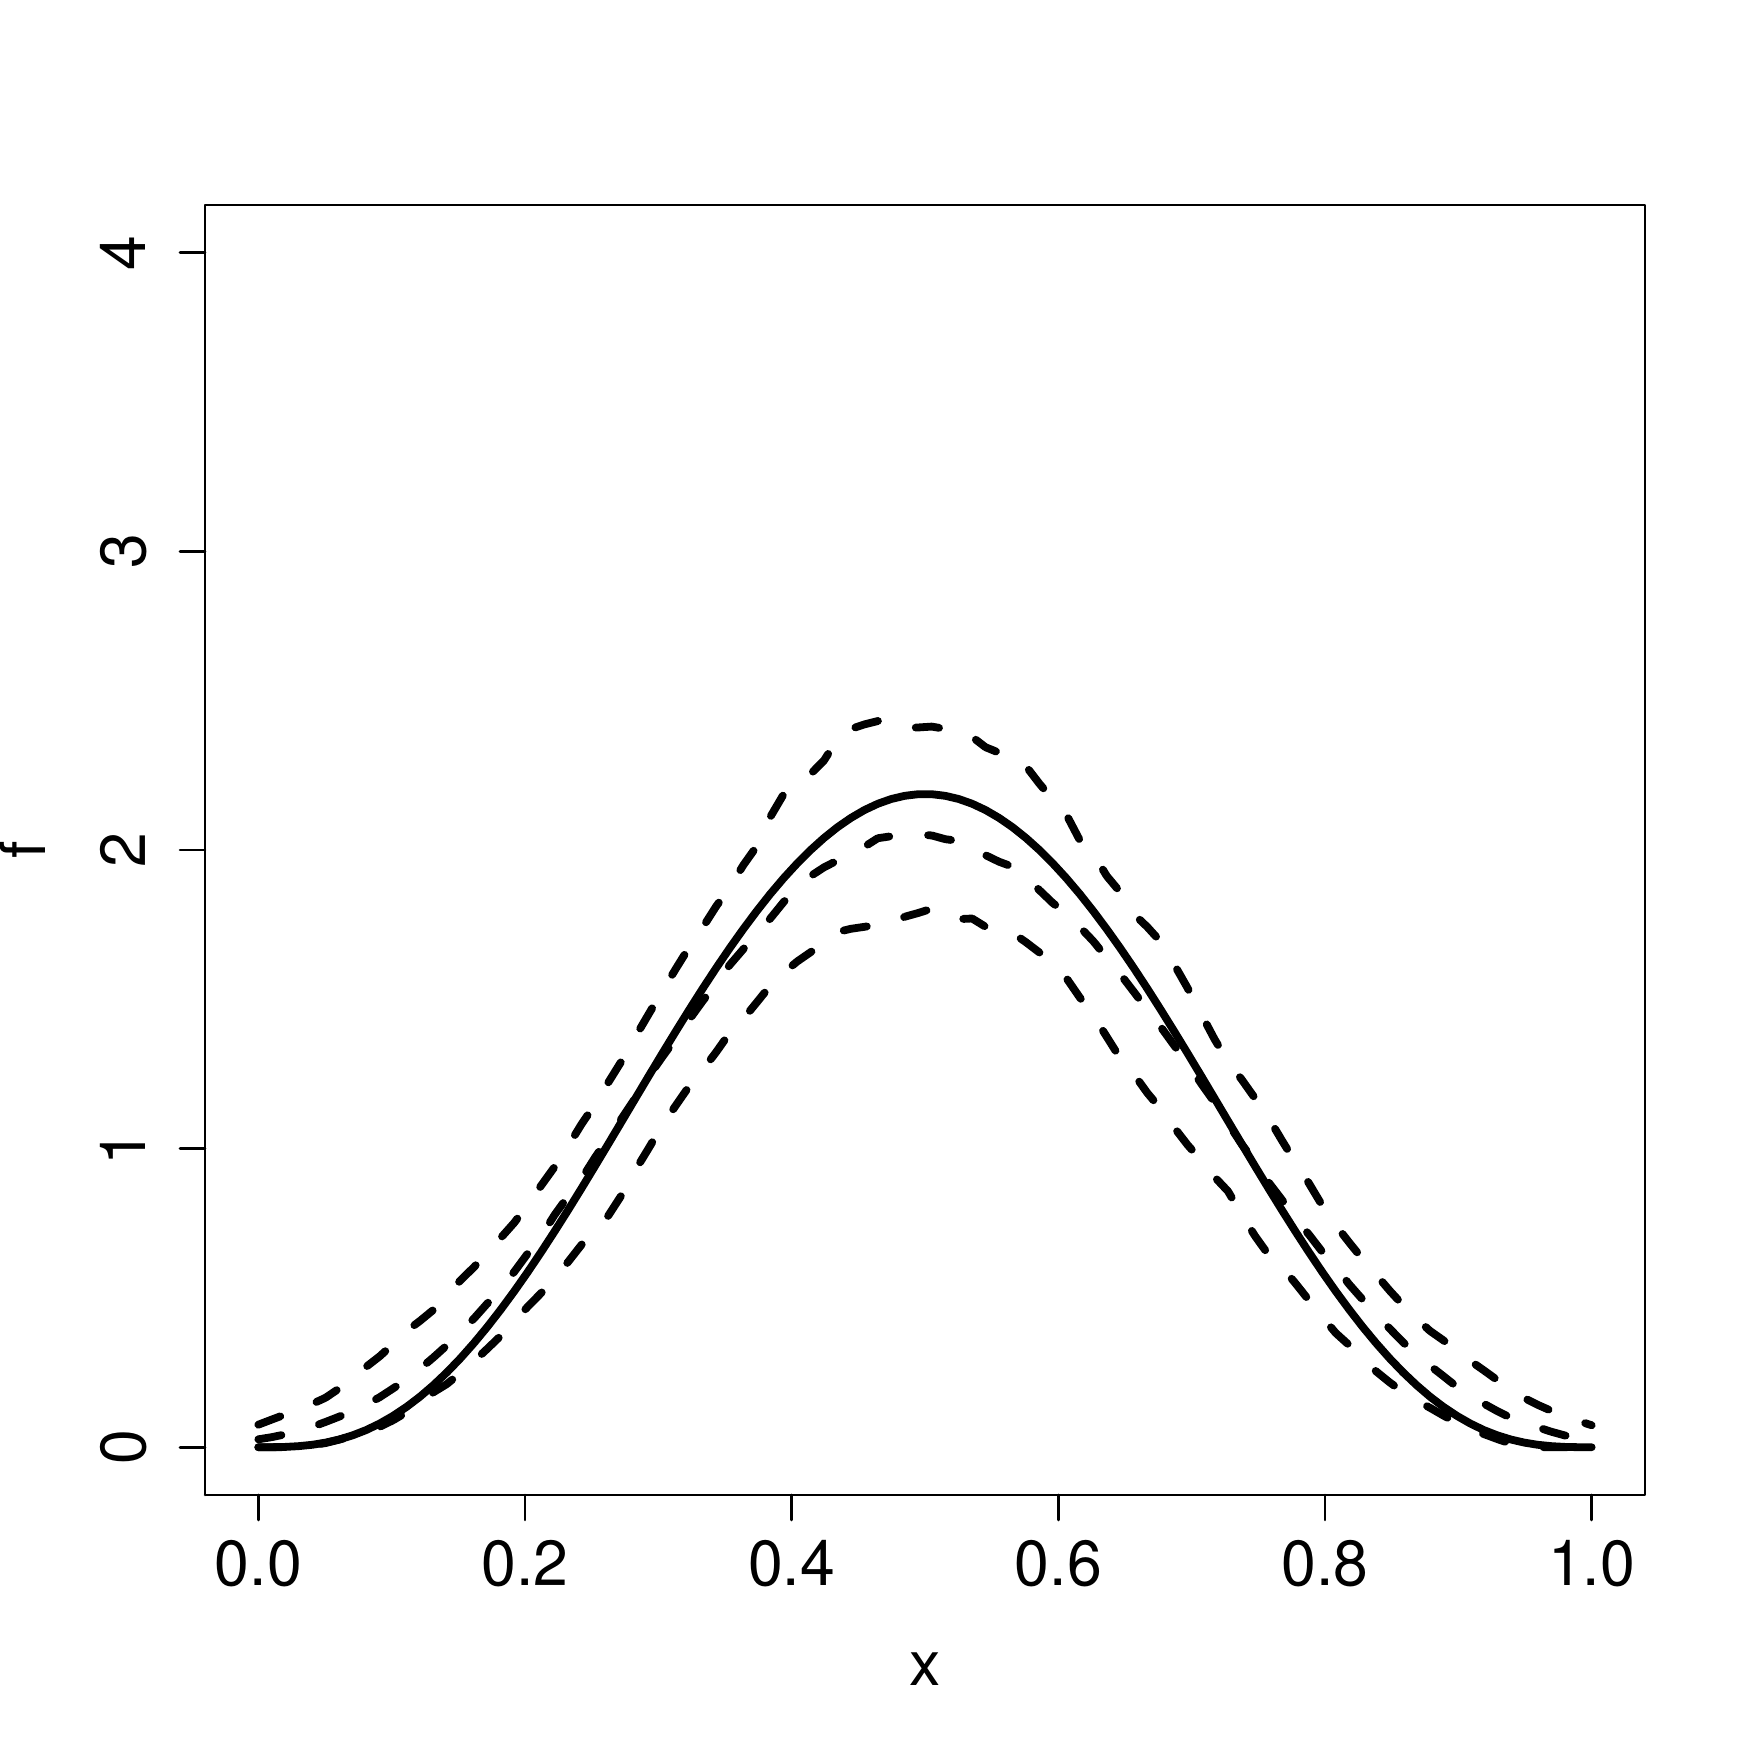}\\
\includegraphics[scale = 0.35]{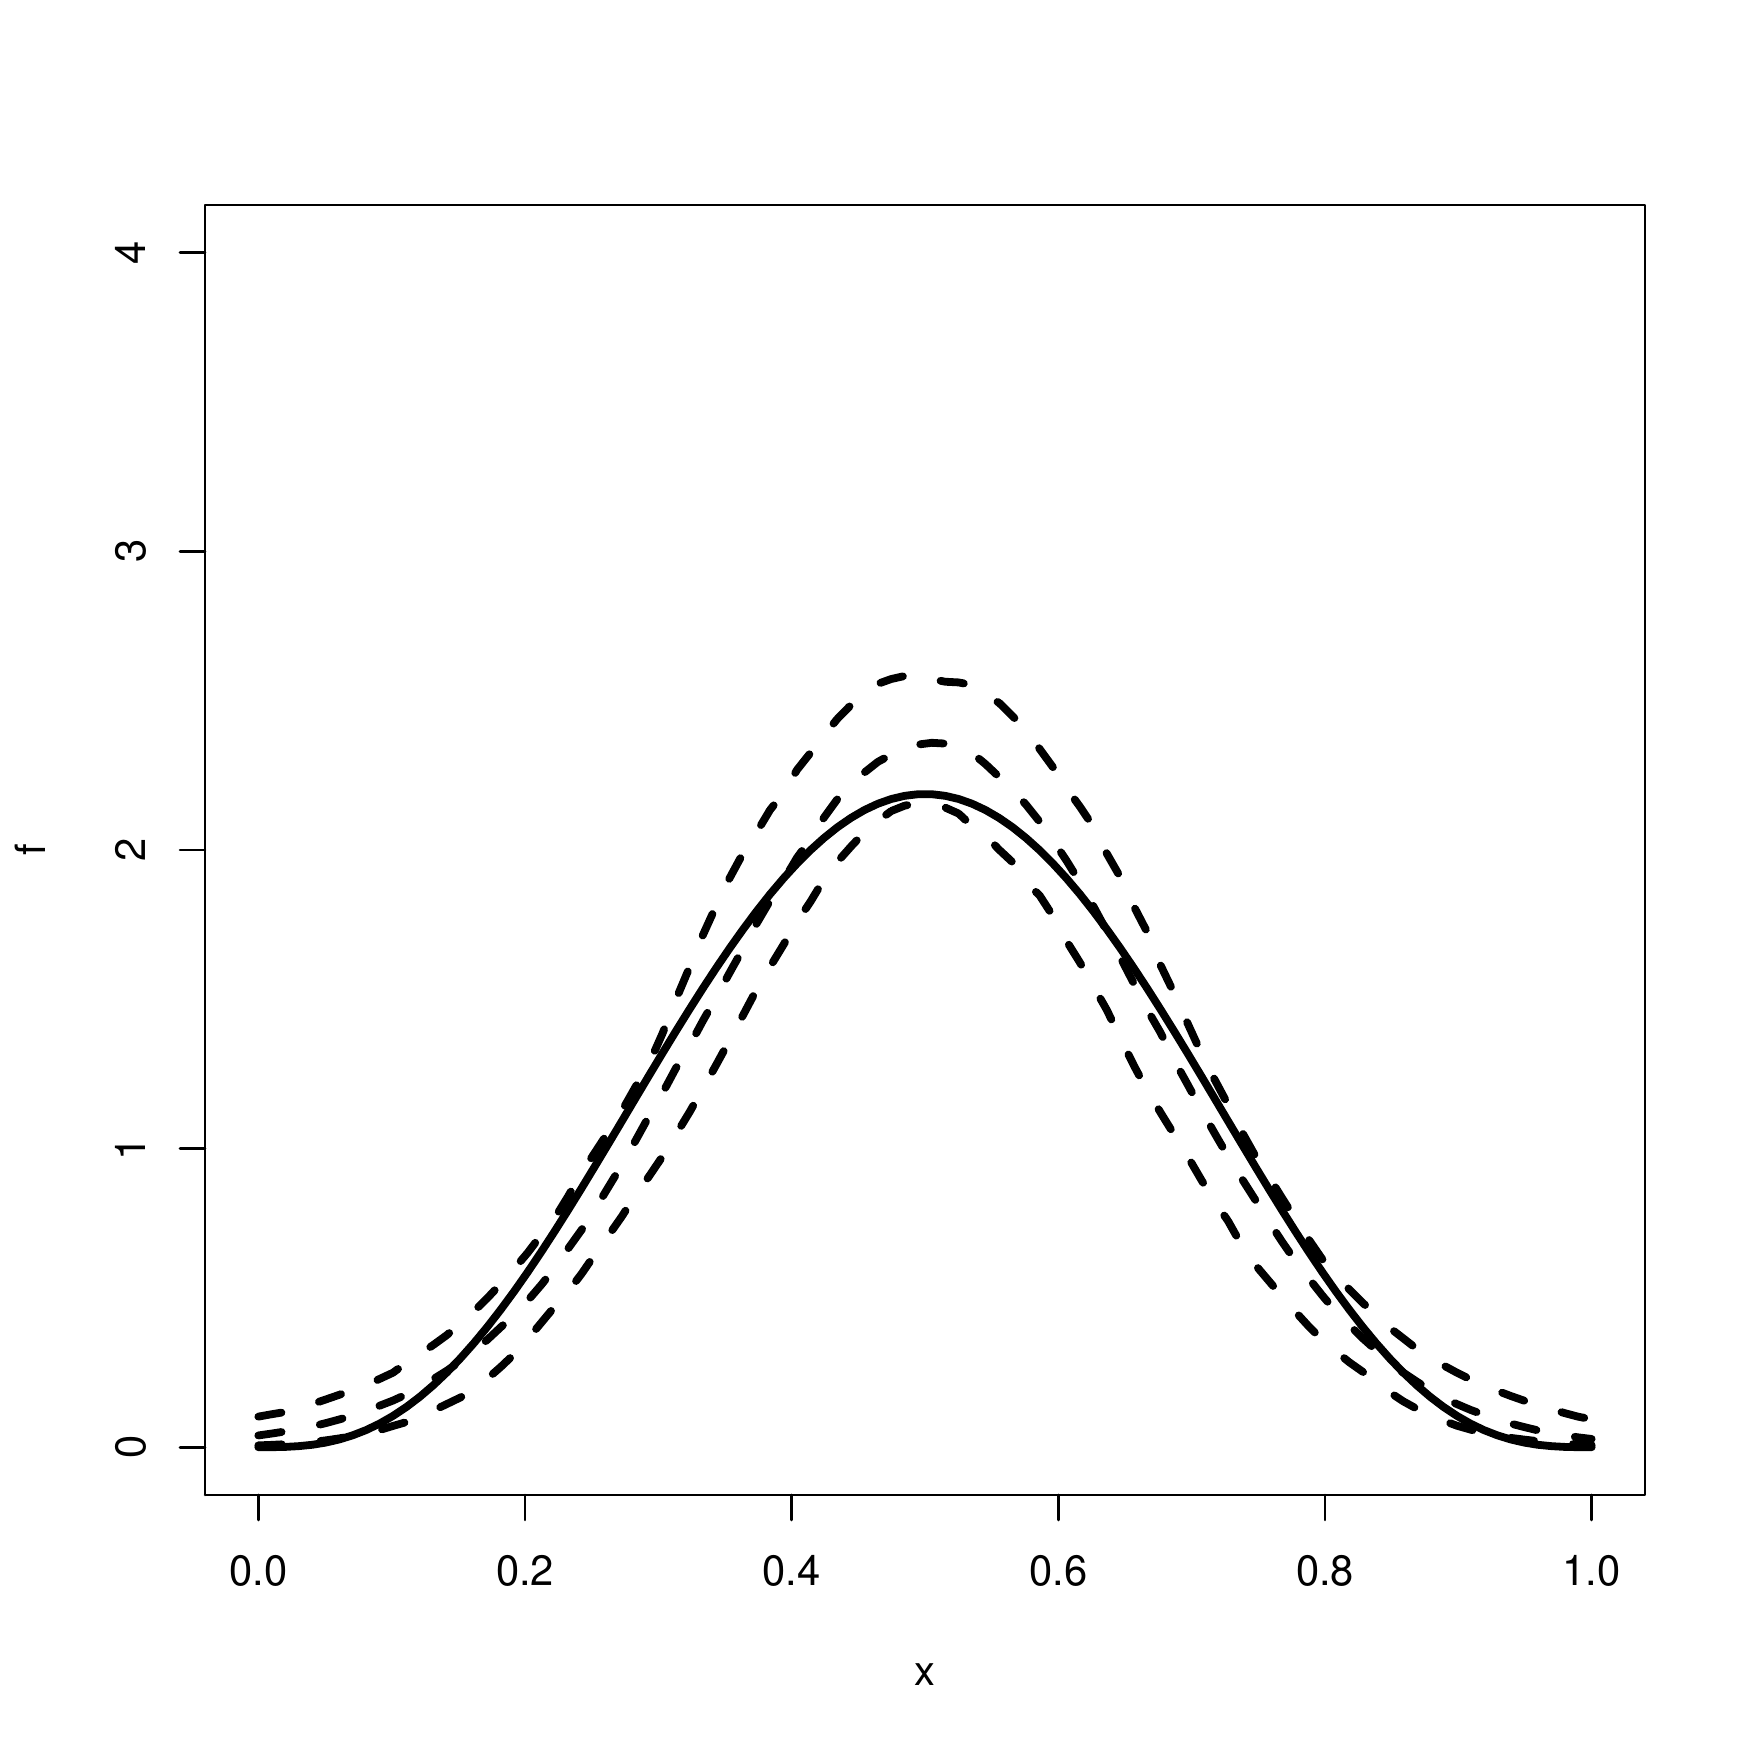}
\includegraphics[scale = 0.35]{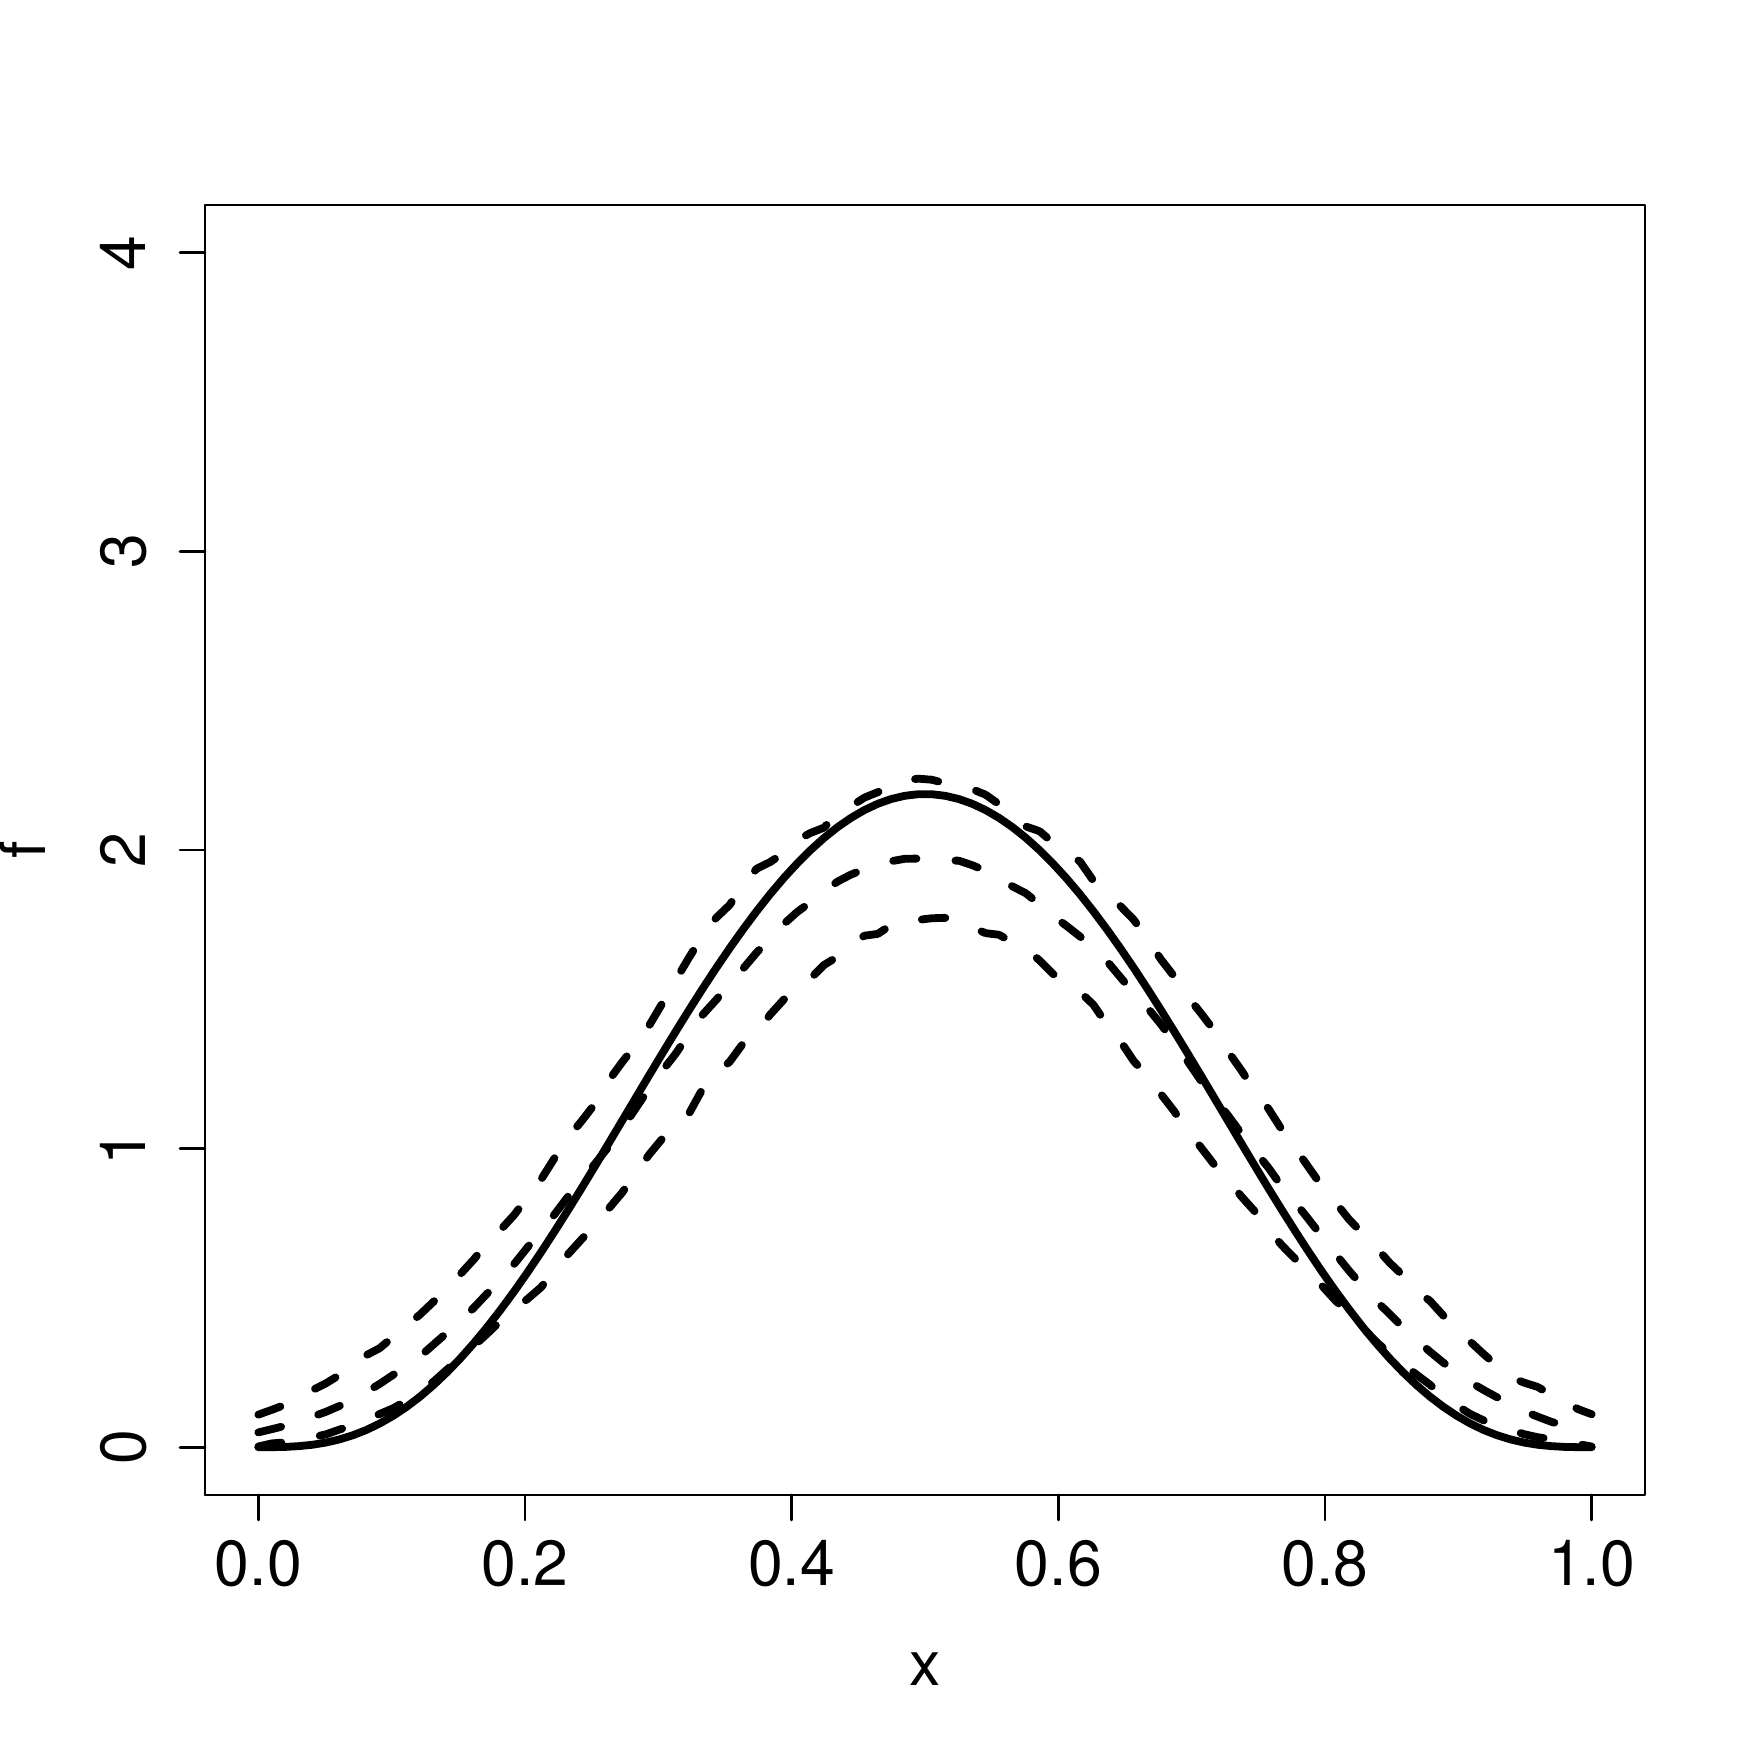}\\
\includegraphics[scale = 0.35]{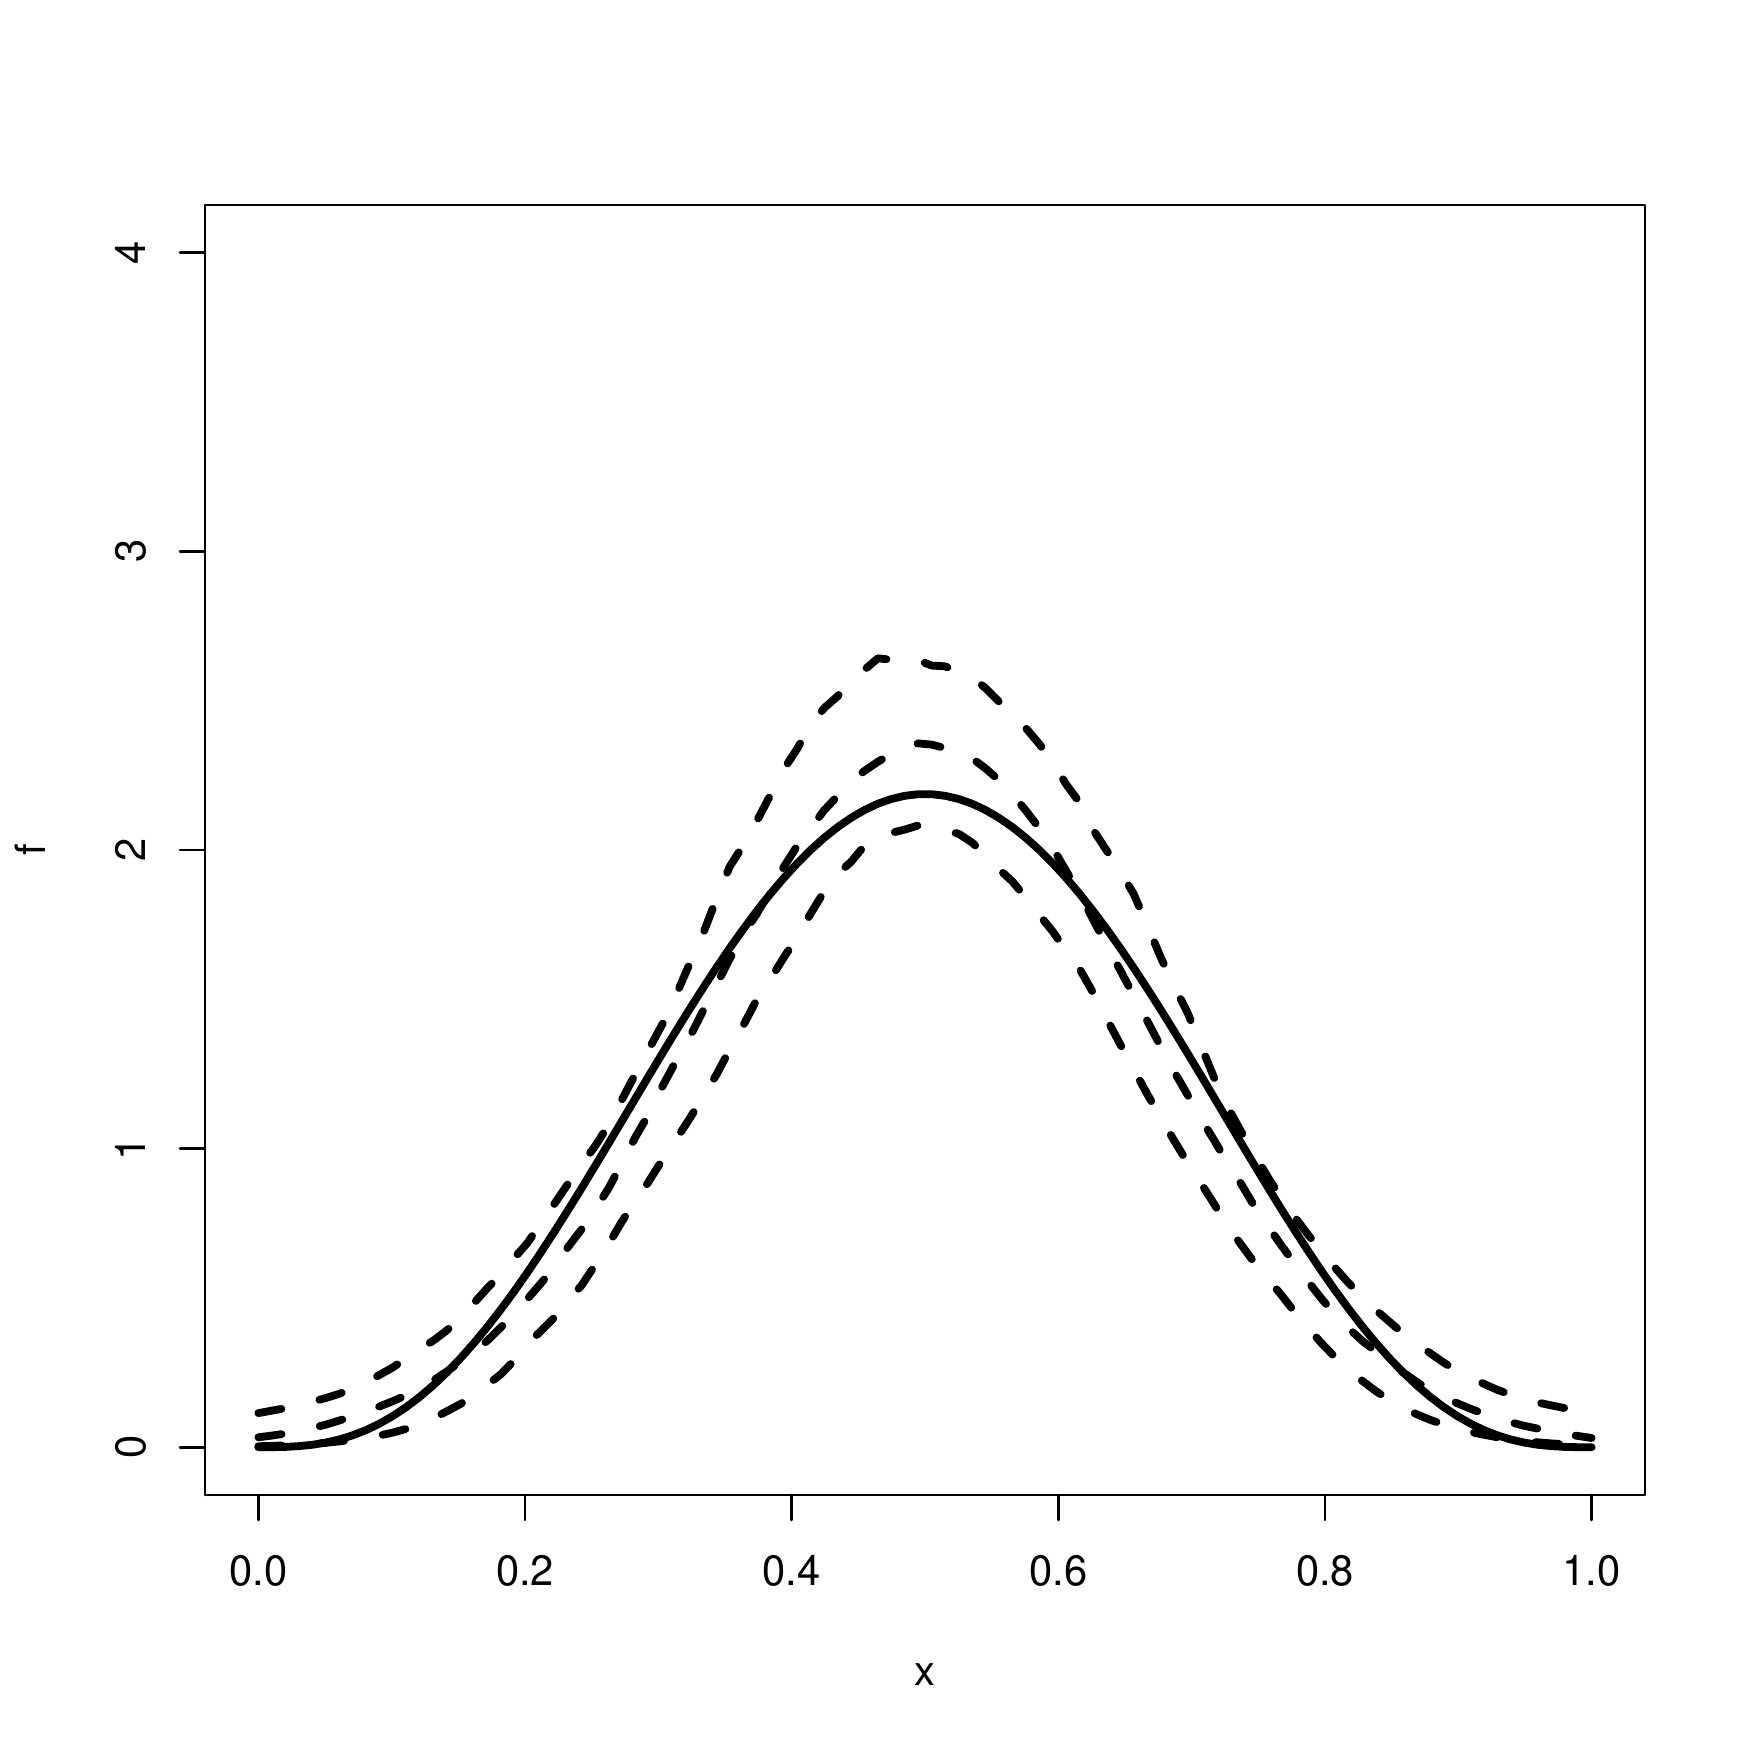}
\includegraphics[scale = 0.35]{figures/den2002.pdf}
\end{center}
\end{figure}

\begin{figure}[!h]
\caption{B-spline semiparametric regression estimation (left) and 
deconvolution estimation (right) 
from 200 
  simulations: The solid lines represent the true functions and the 
  dash lines represent the estimated functions and their 90\%
  confidence bands. The first row to third row are the results for 
  model II (a)--(c), respectively. Sample size 1000.} 
{\label{fig:mean2}}
\begin{center}
\includegraphics[scale = 0.35]{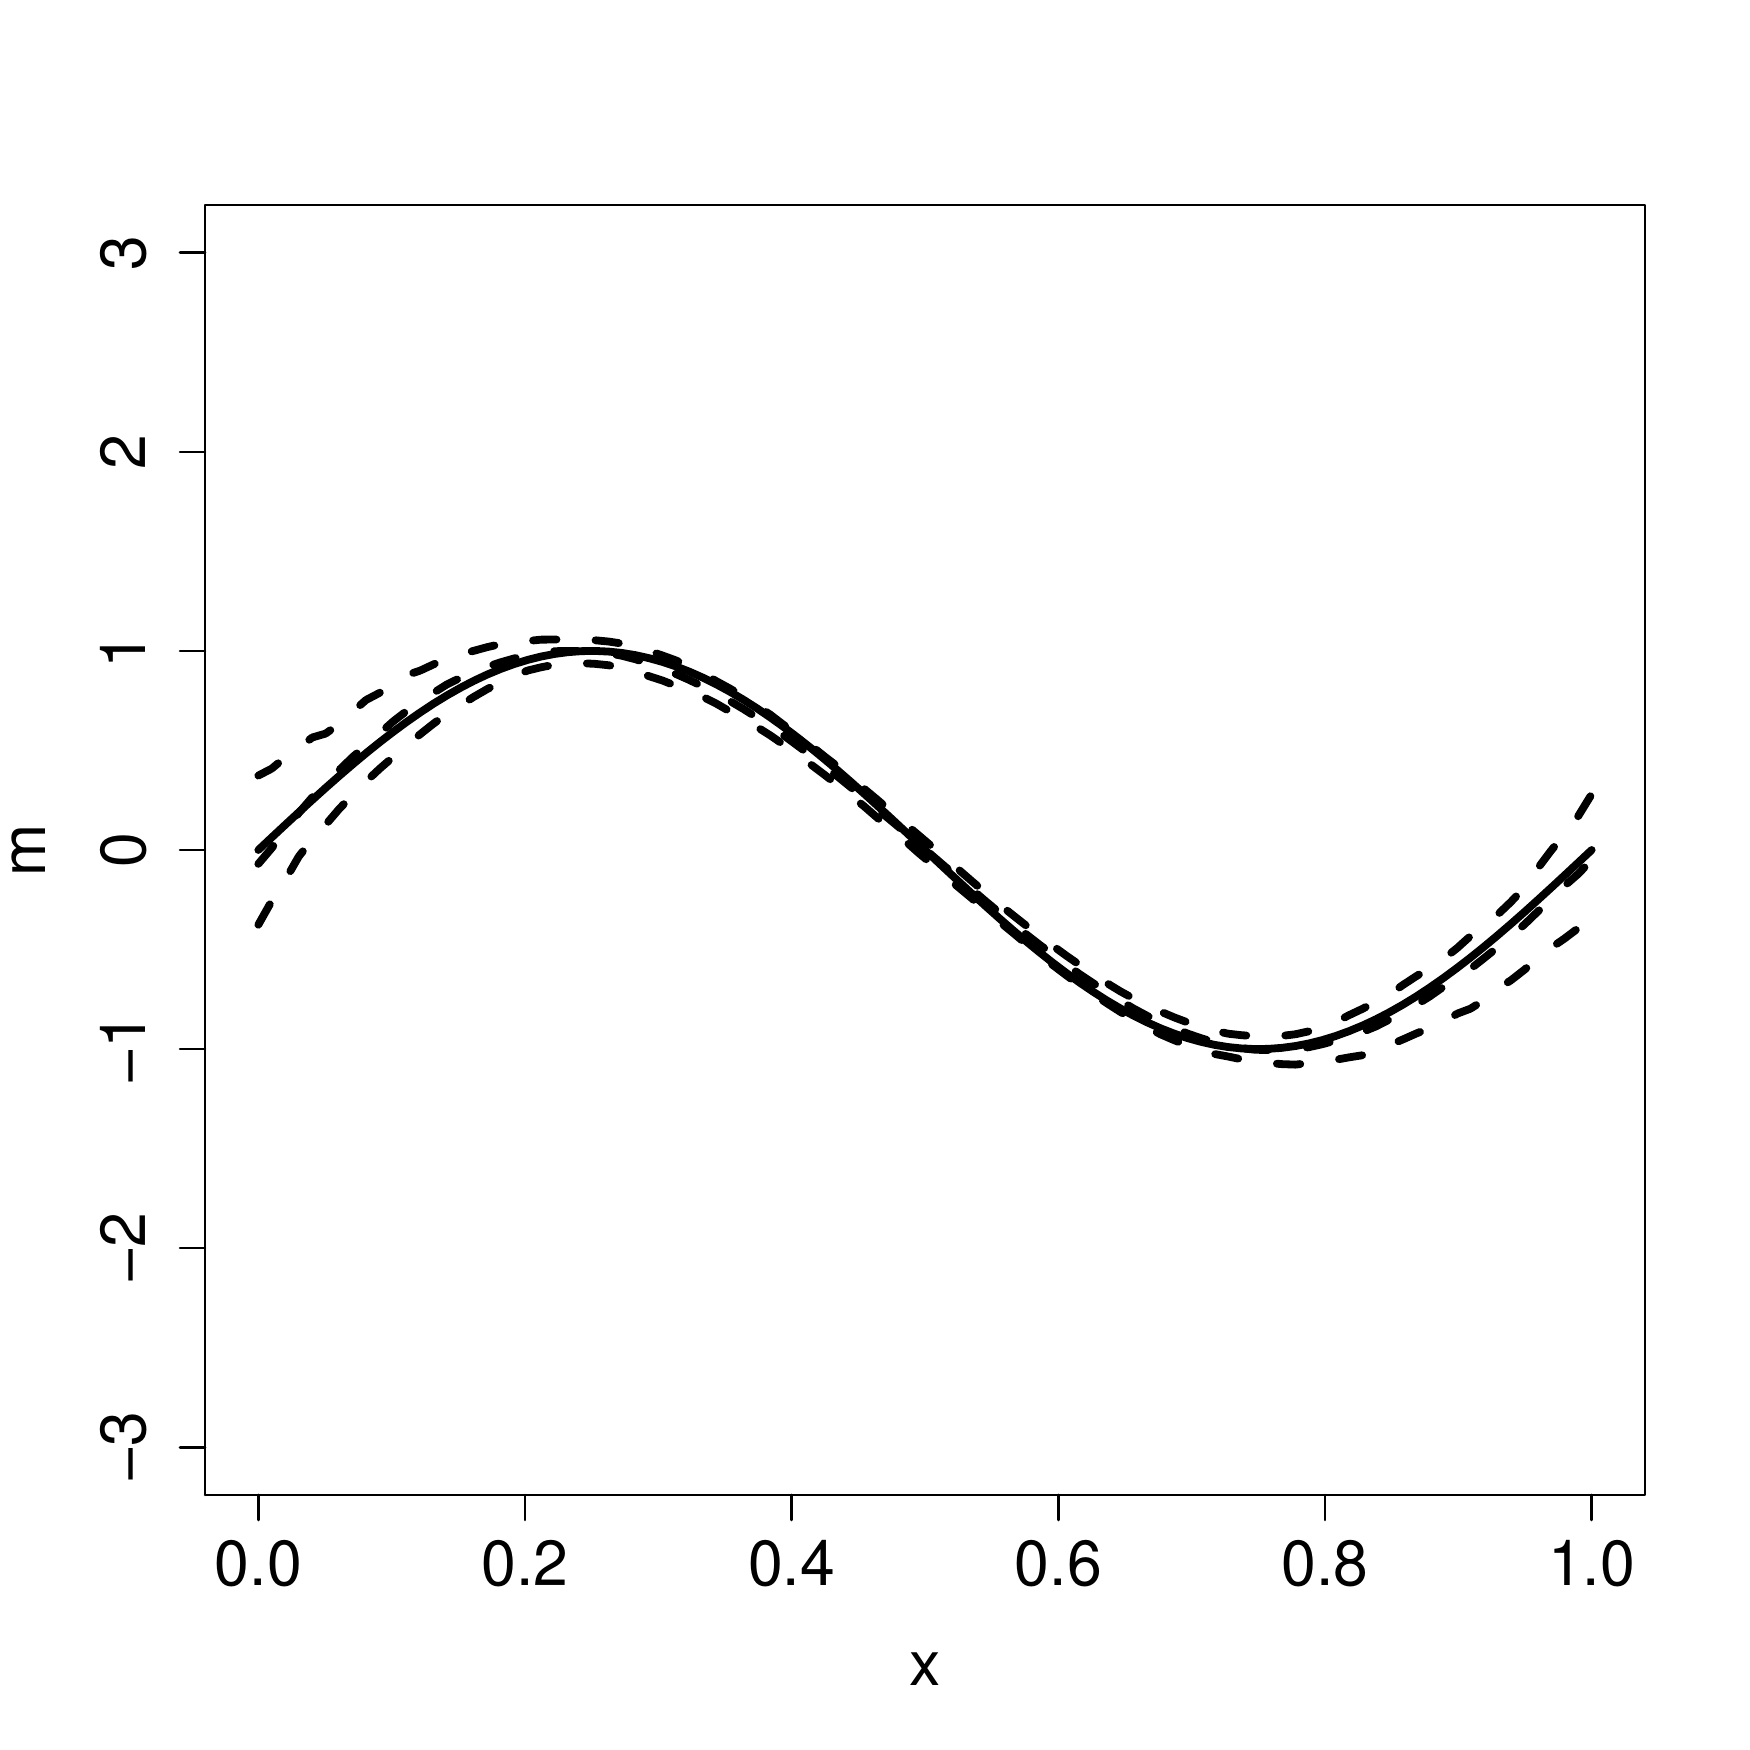}
\includegraphics[scale = 0.35]{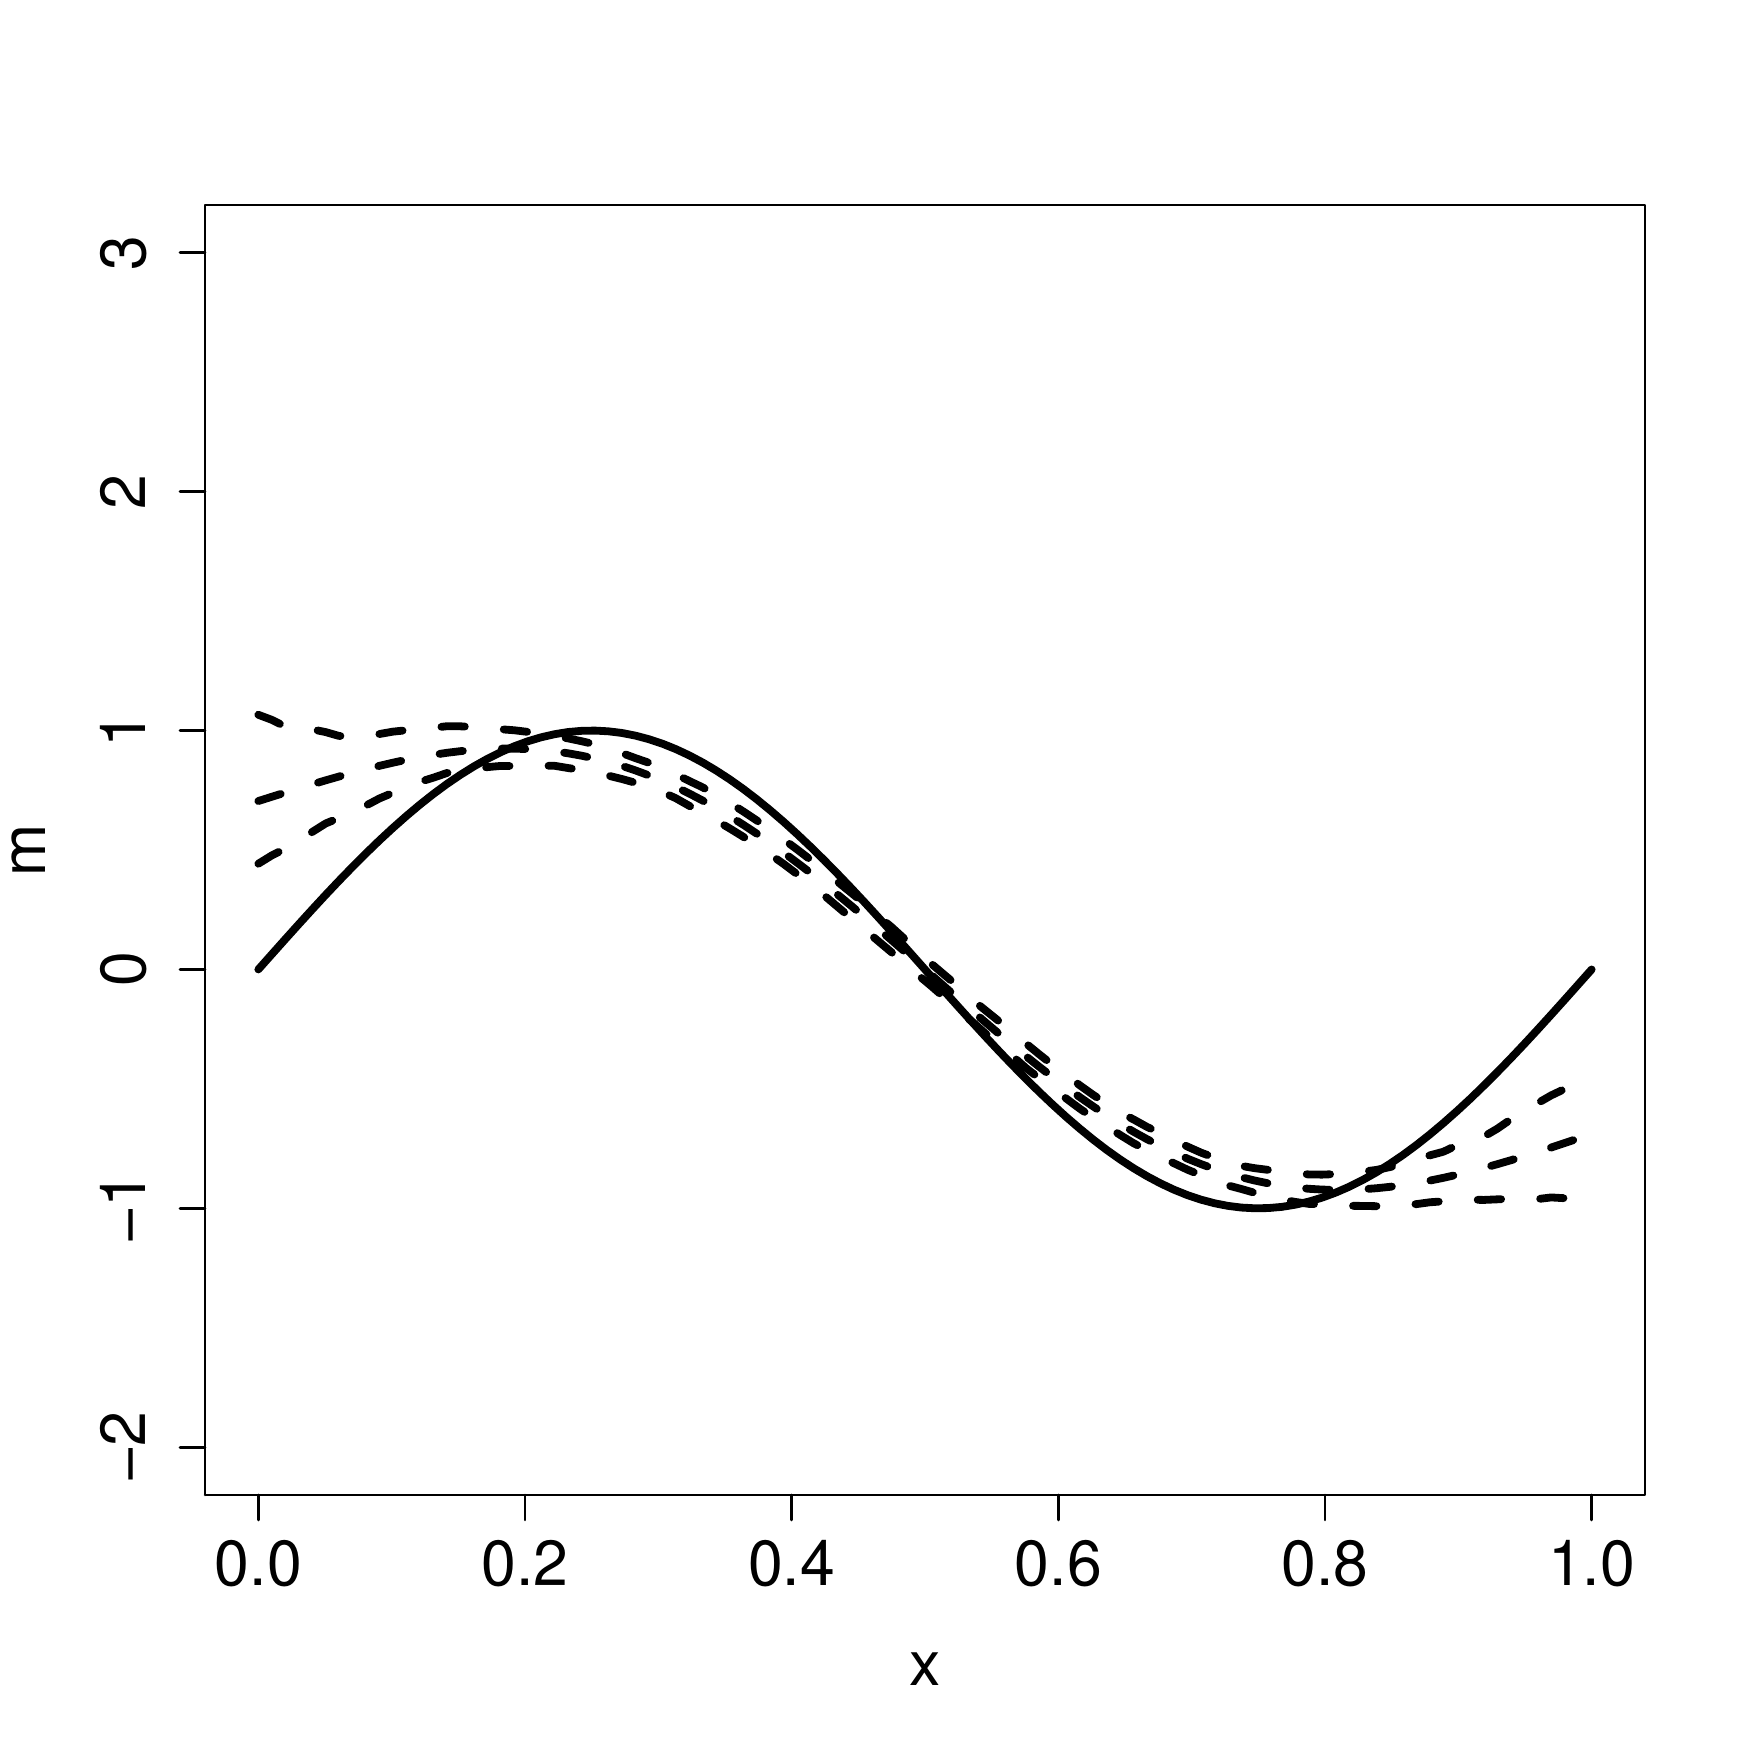}\\
\includegraphics[scale = 0.35]{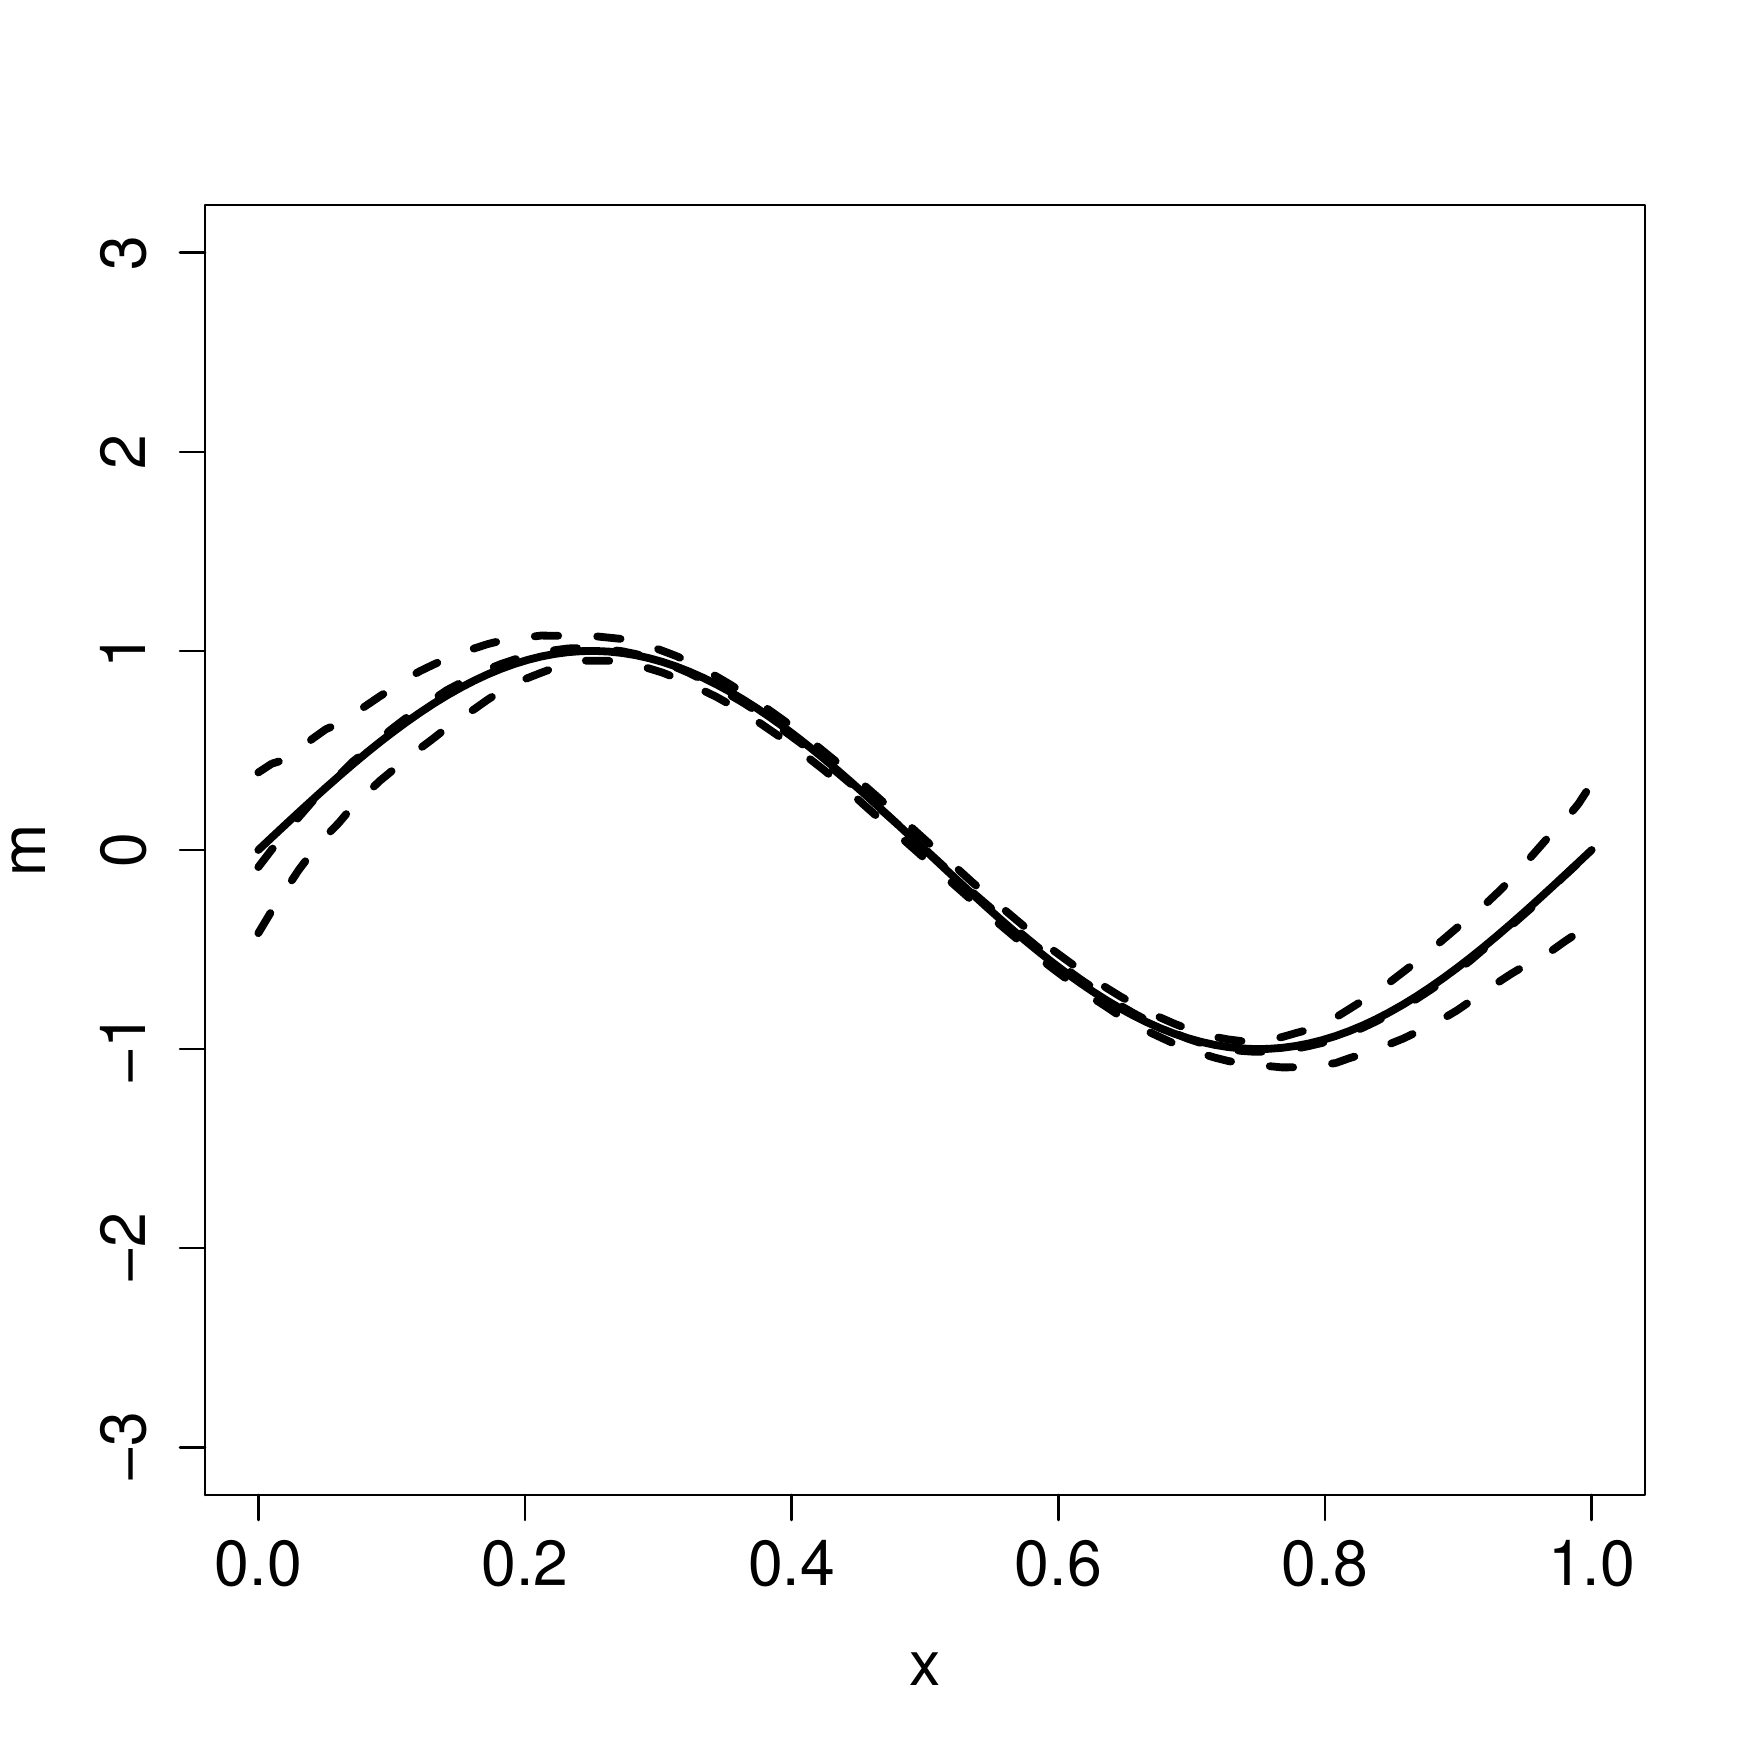}
\includegraphics[scale = 0.35]{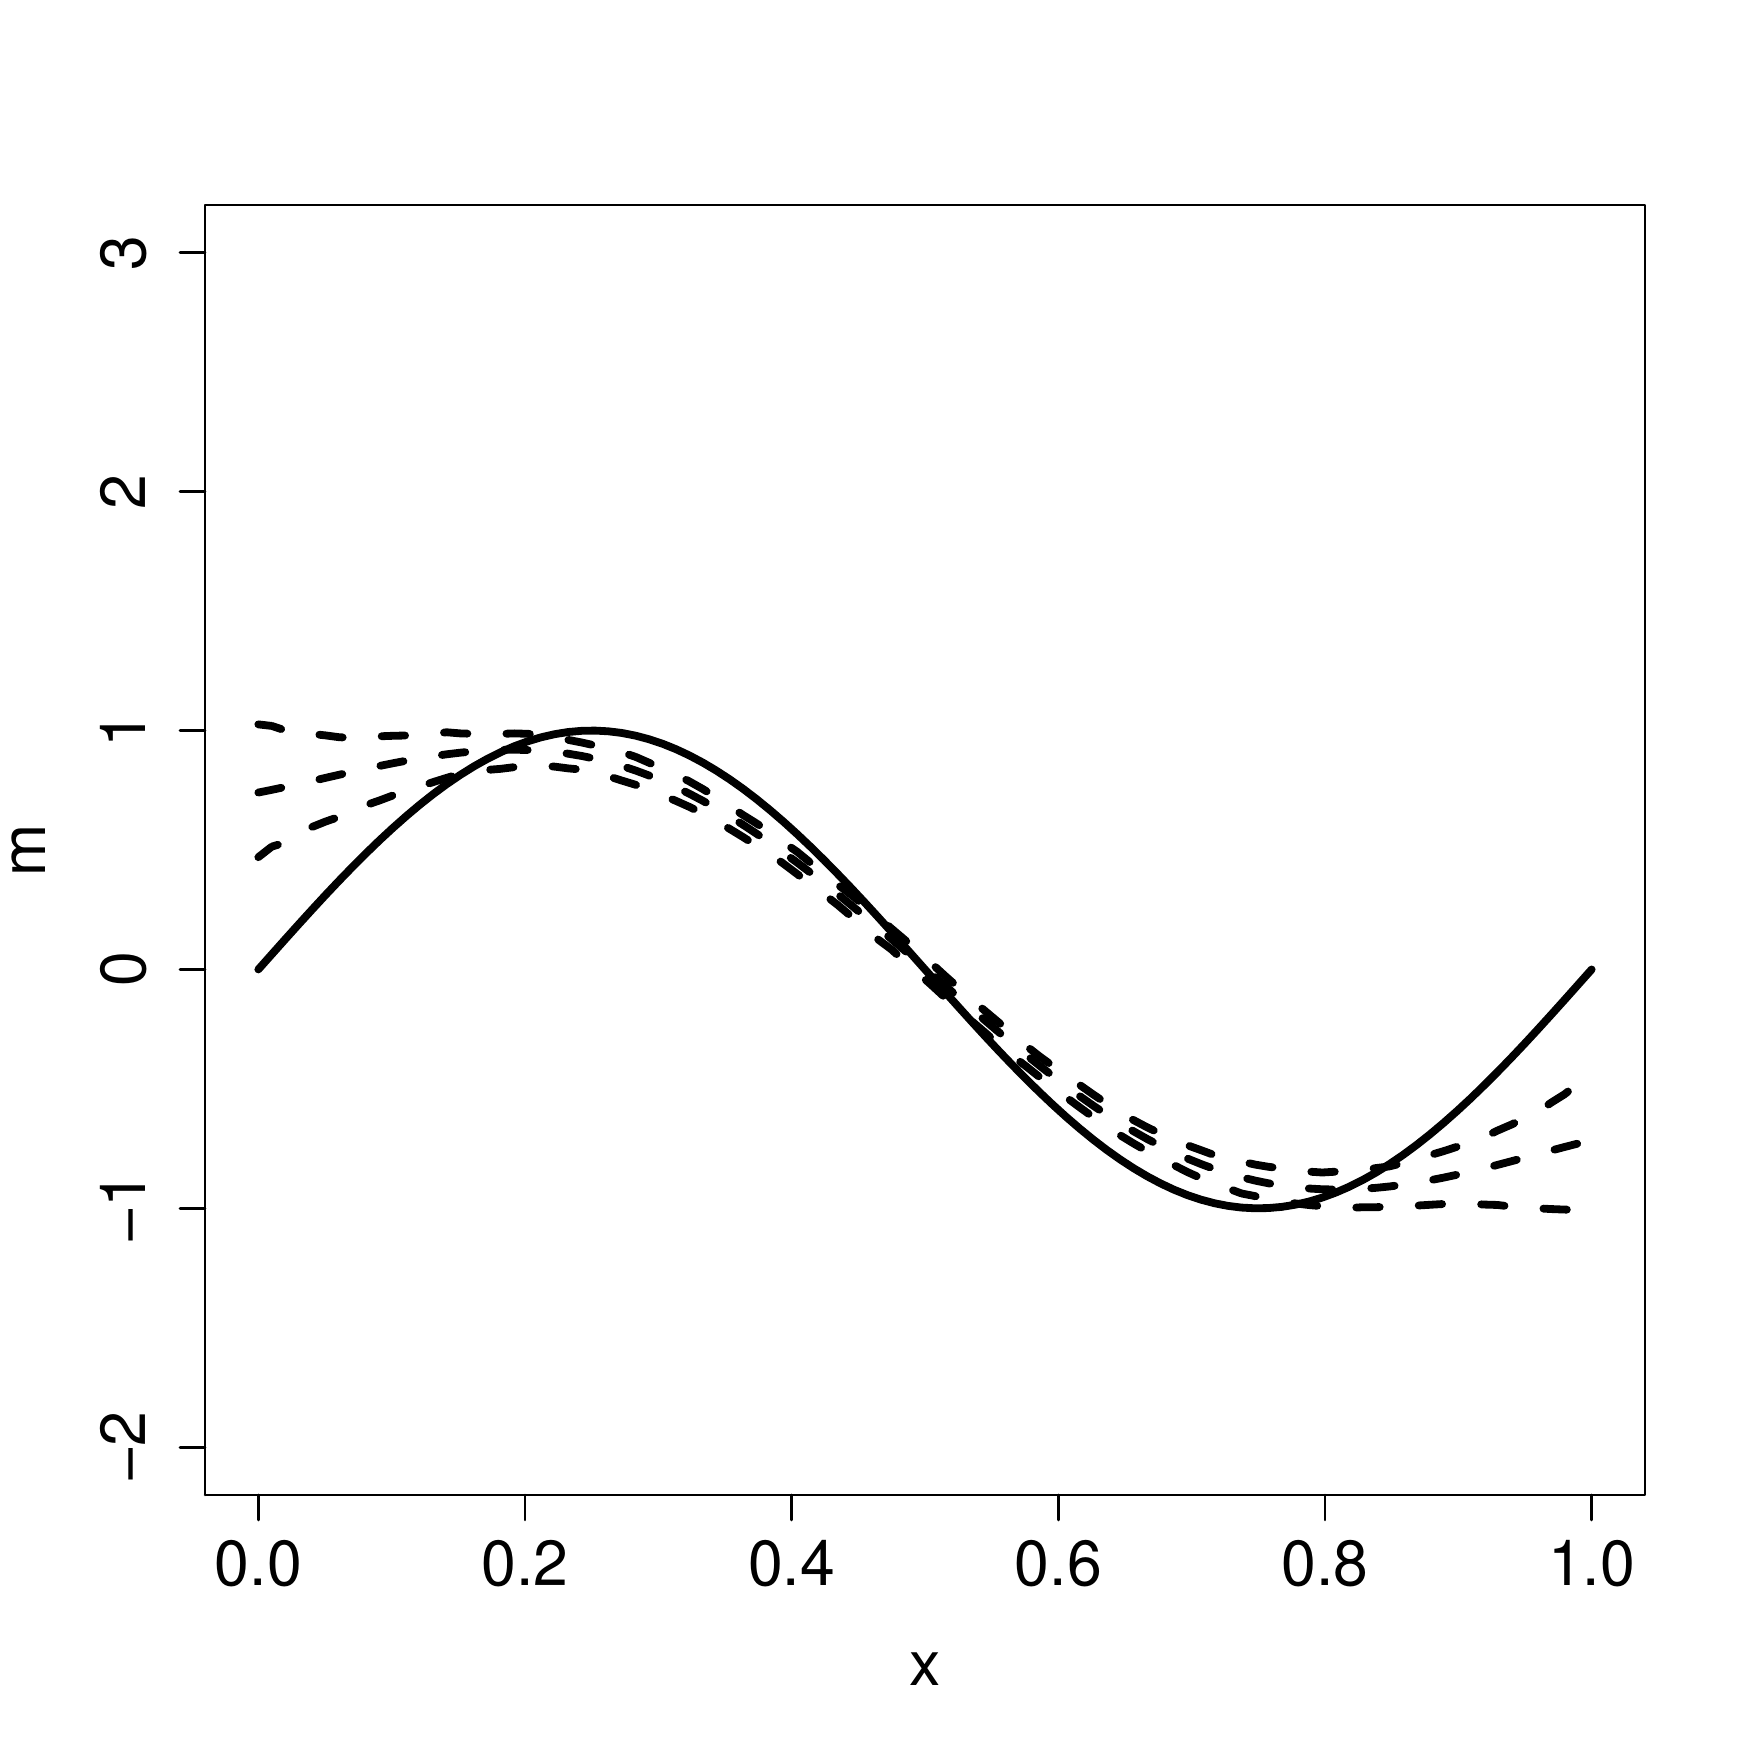}\\
\includegraphics[scale = 0.35]{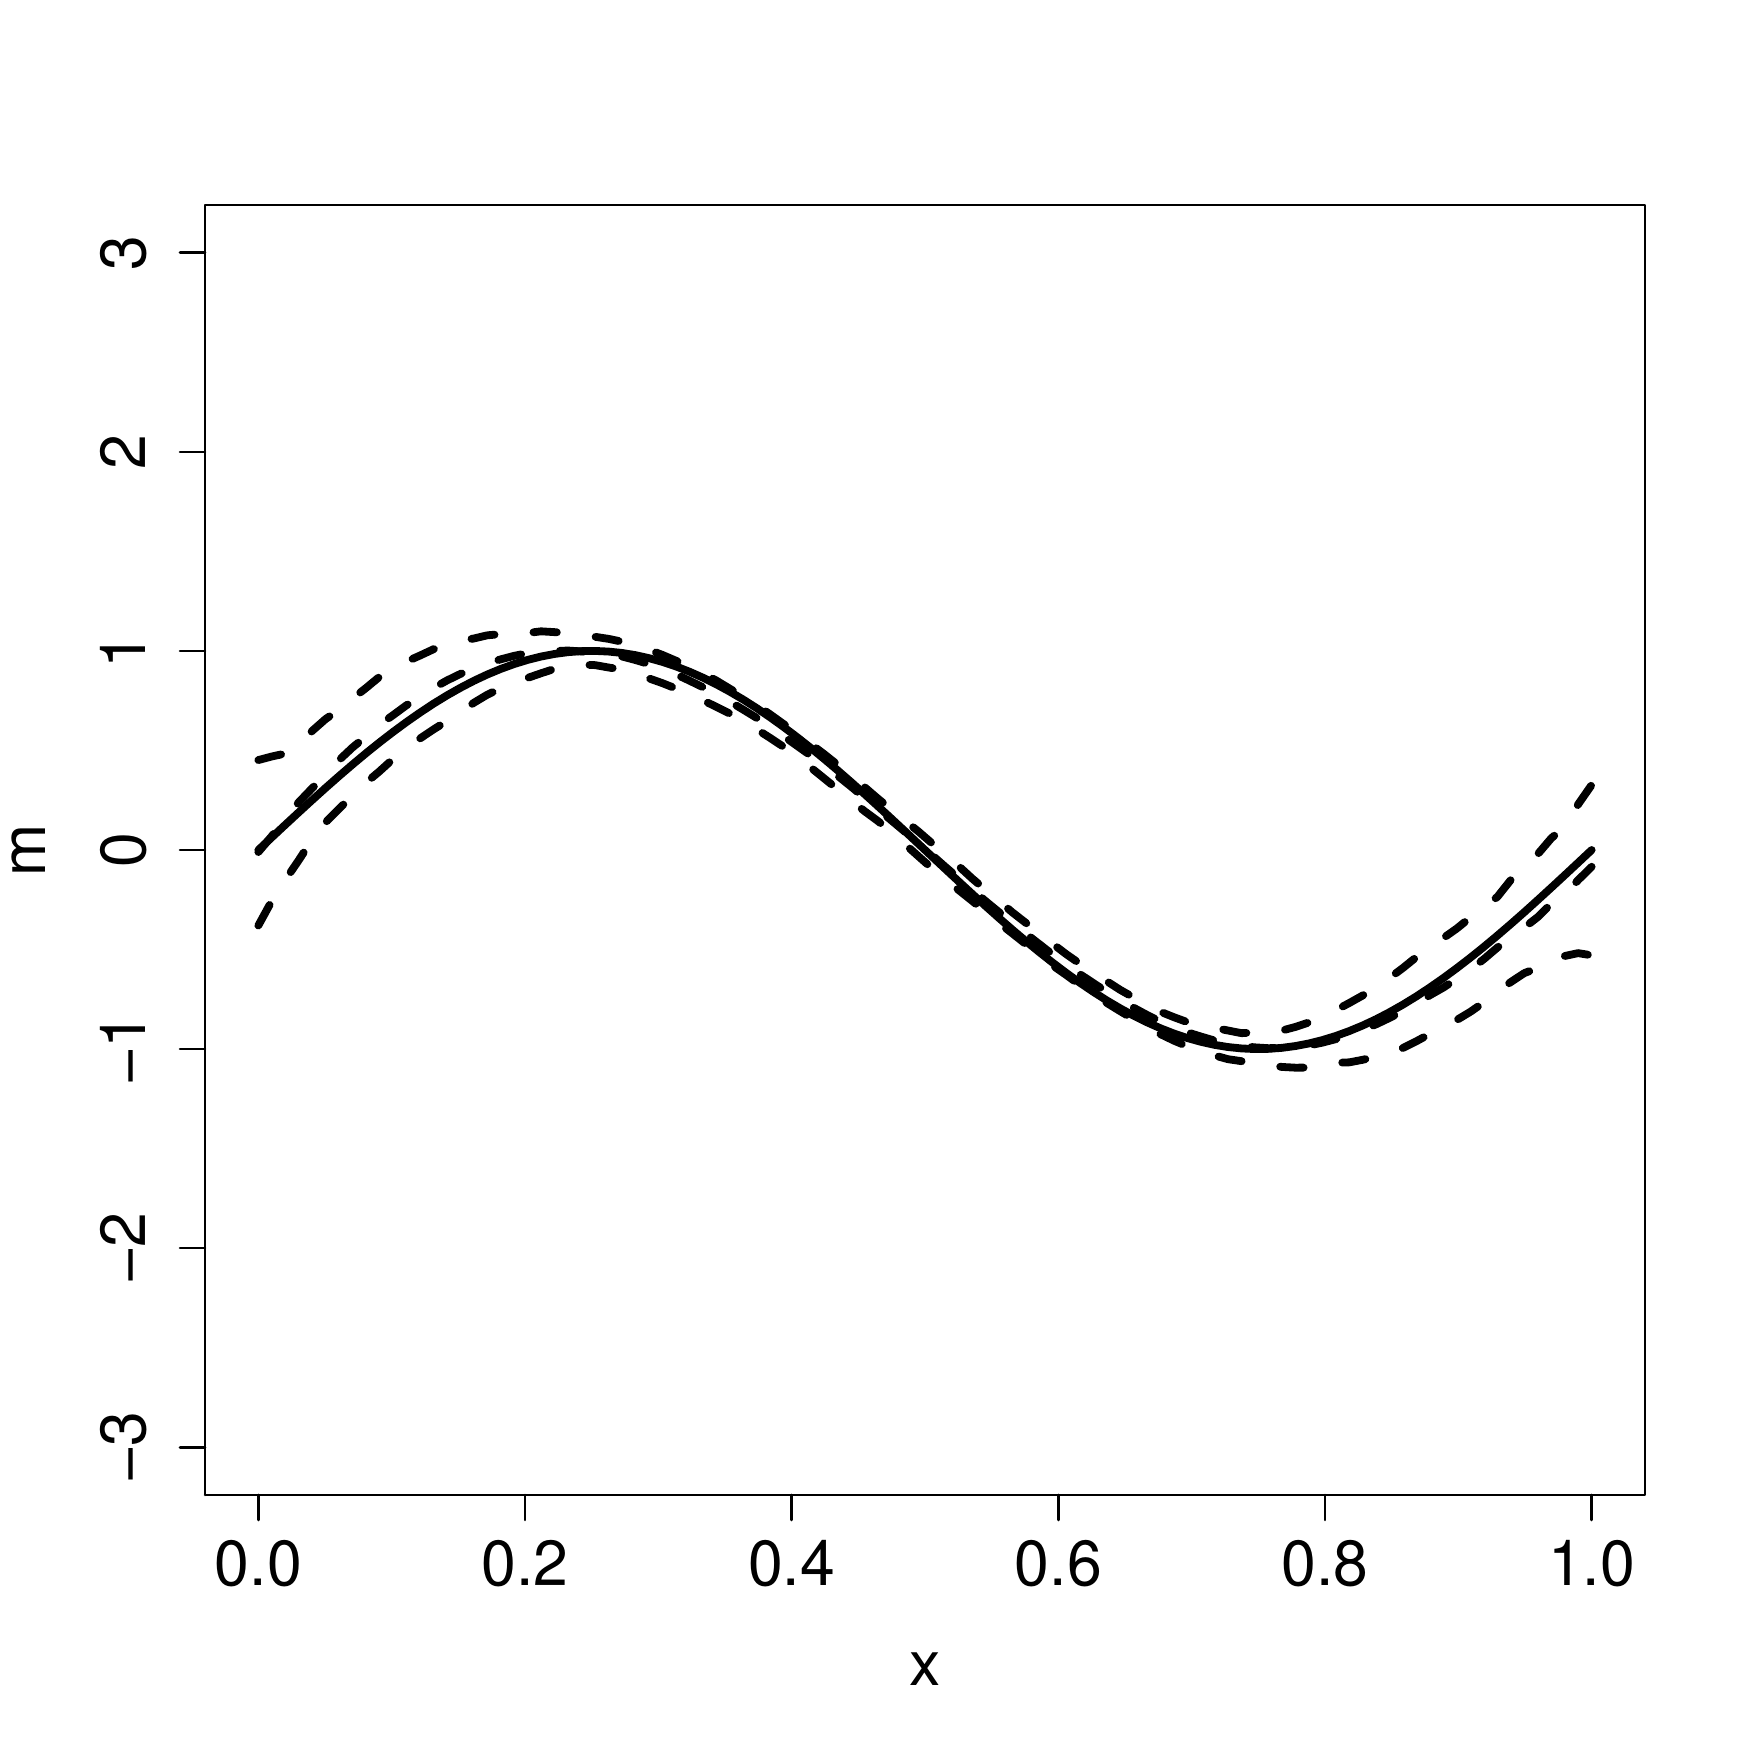}
\includegraphics[scale = 0.35]{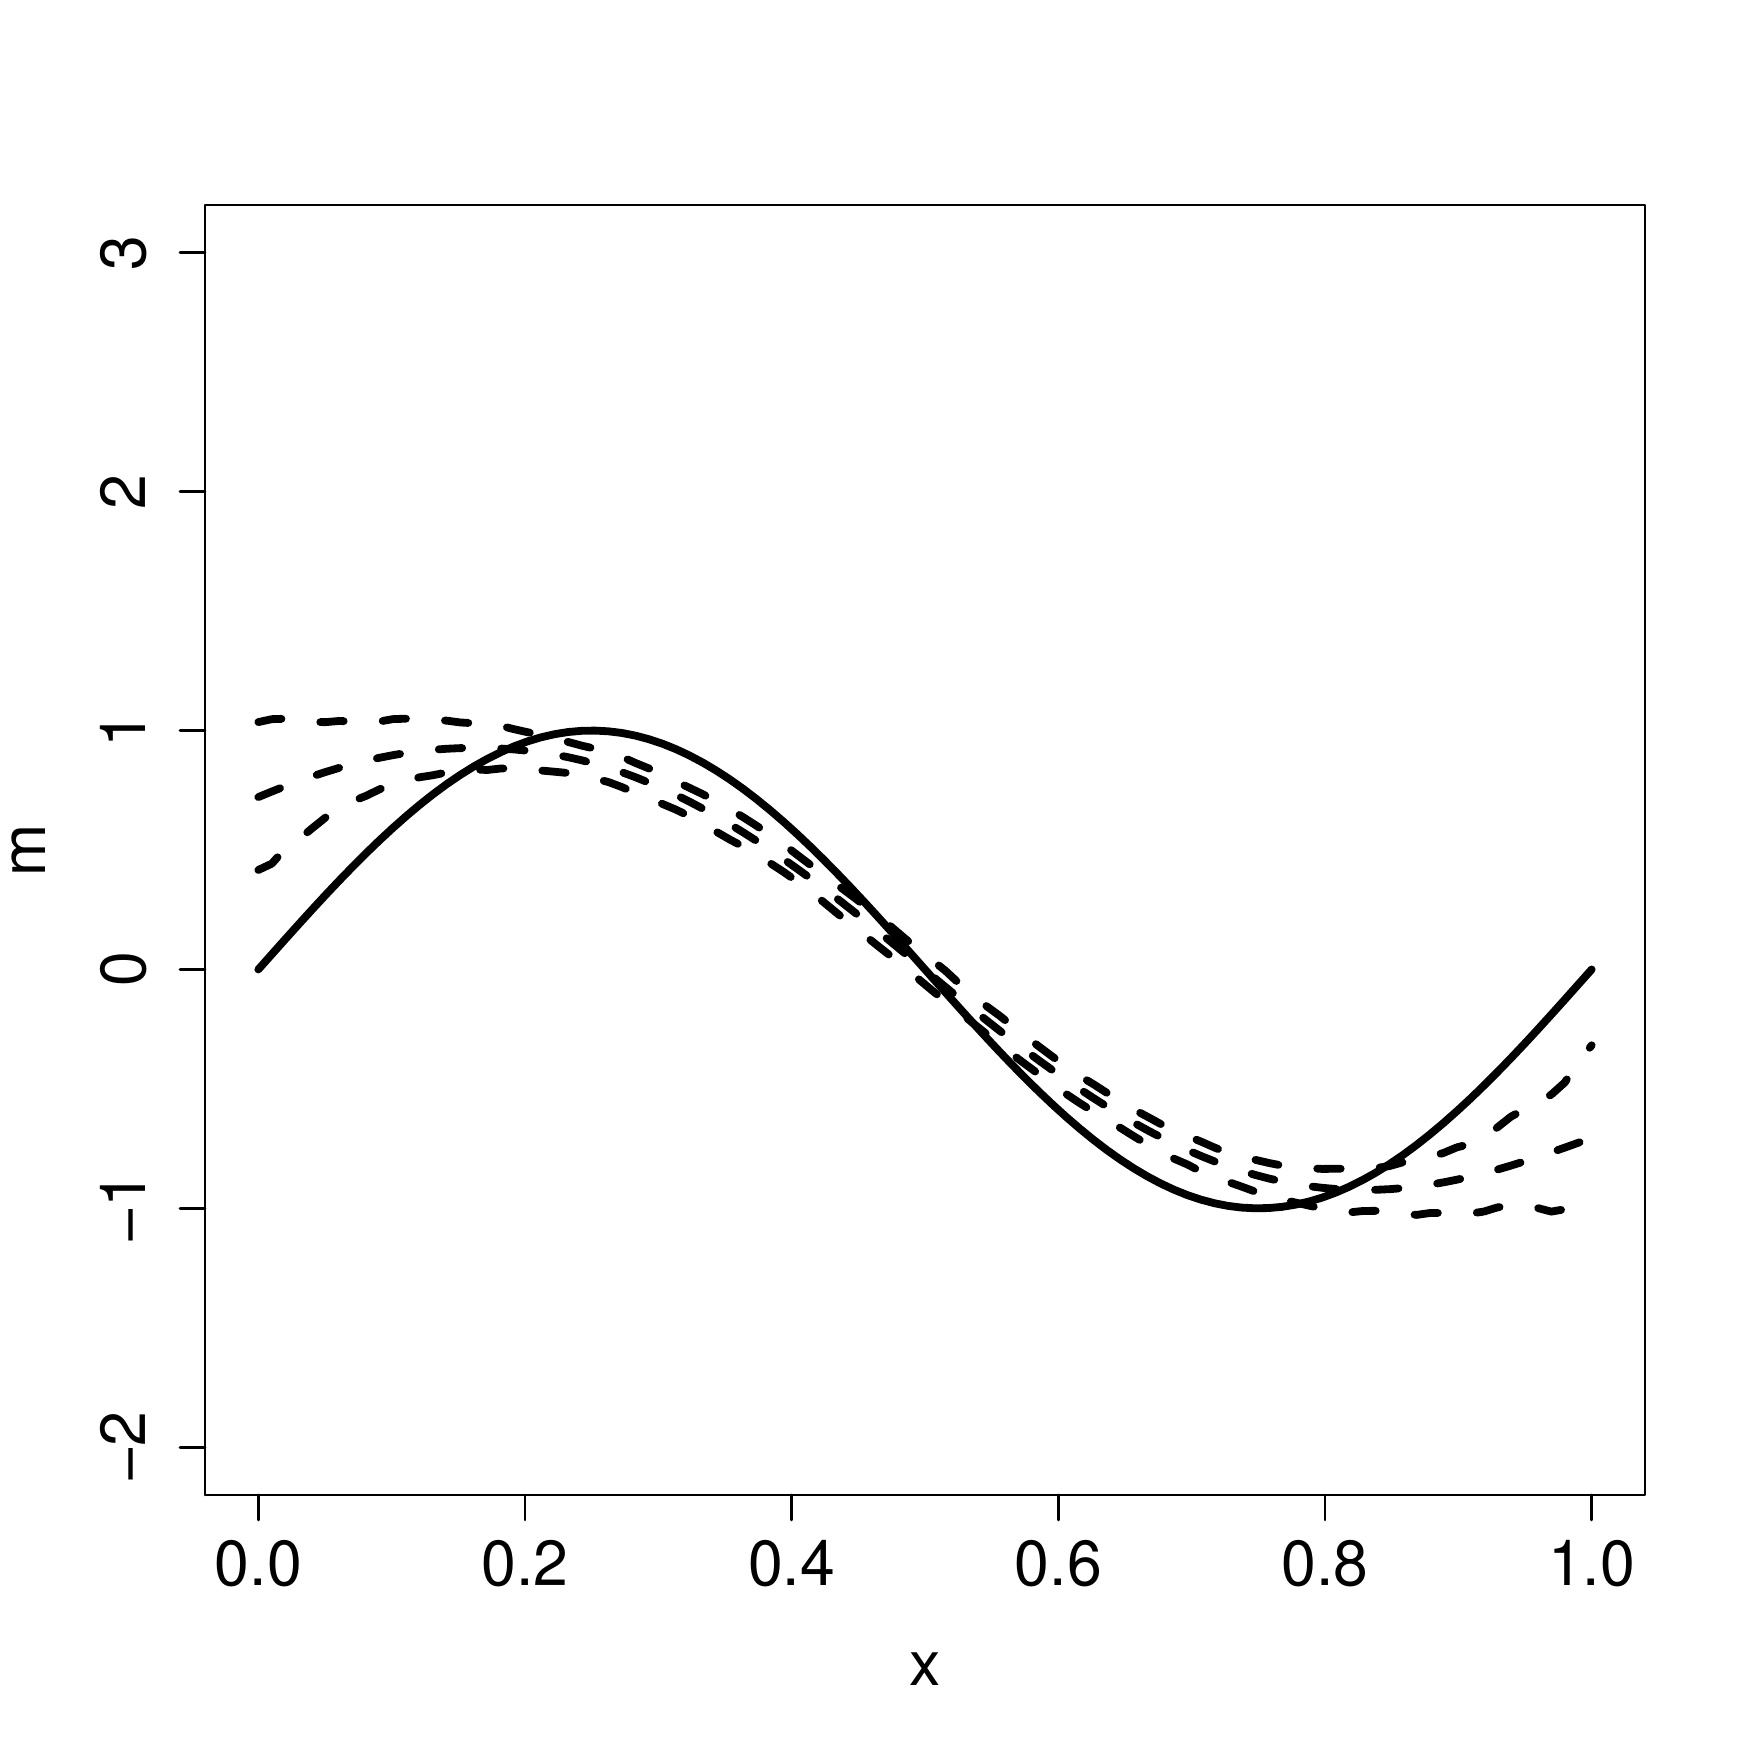}
\end{center}
\end{figure}

\begin{figure}[!h]
\caption{B-spline semiparametric regression estimation (left) and 
deconvolution estimation (right) 
from 200 
  simulations: The solid lines represent the true functions and the 
  dash lines represent the estimated functions and their 90\%
  confidence bands. The first row to third row are the results for 
  model II (a)--(c), respectively. Sample size 2000.} 
{\label{fig:mean3}}
\begin{center}
\includegraphics[scale = 0.35]{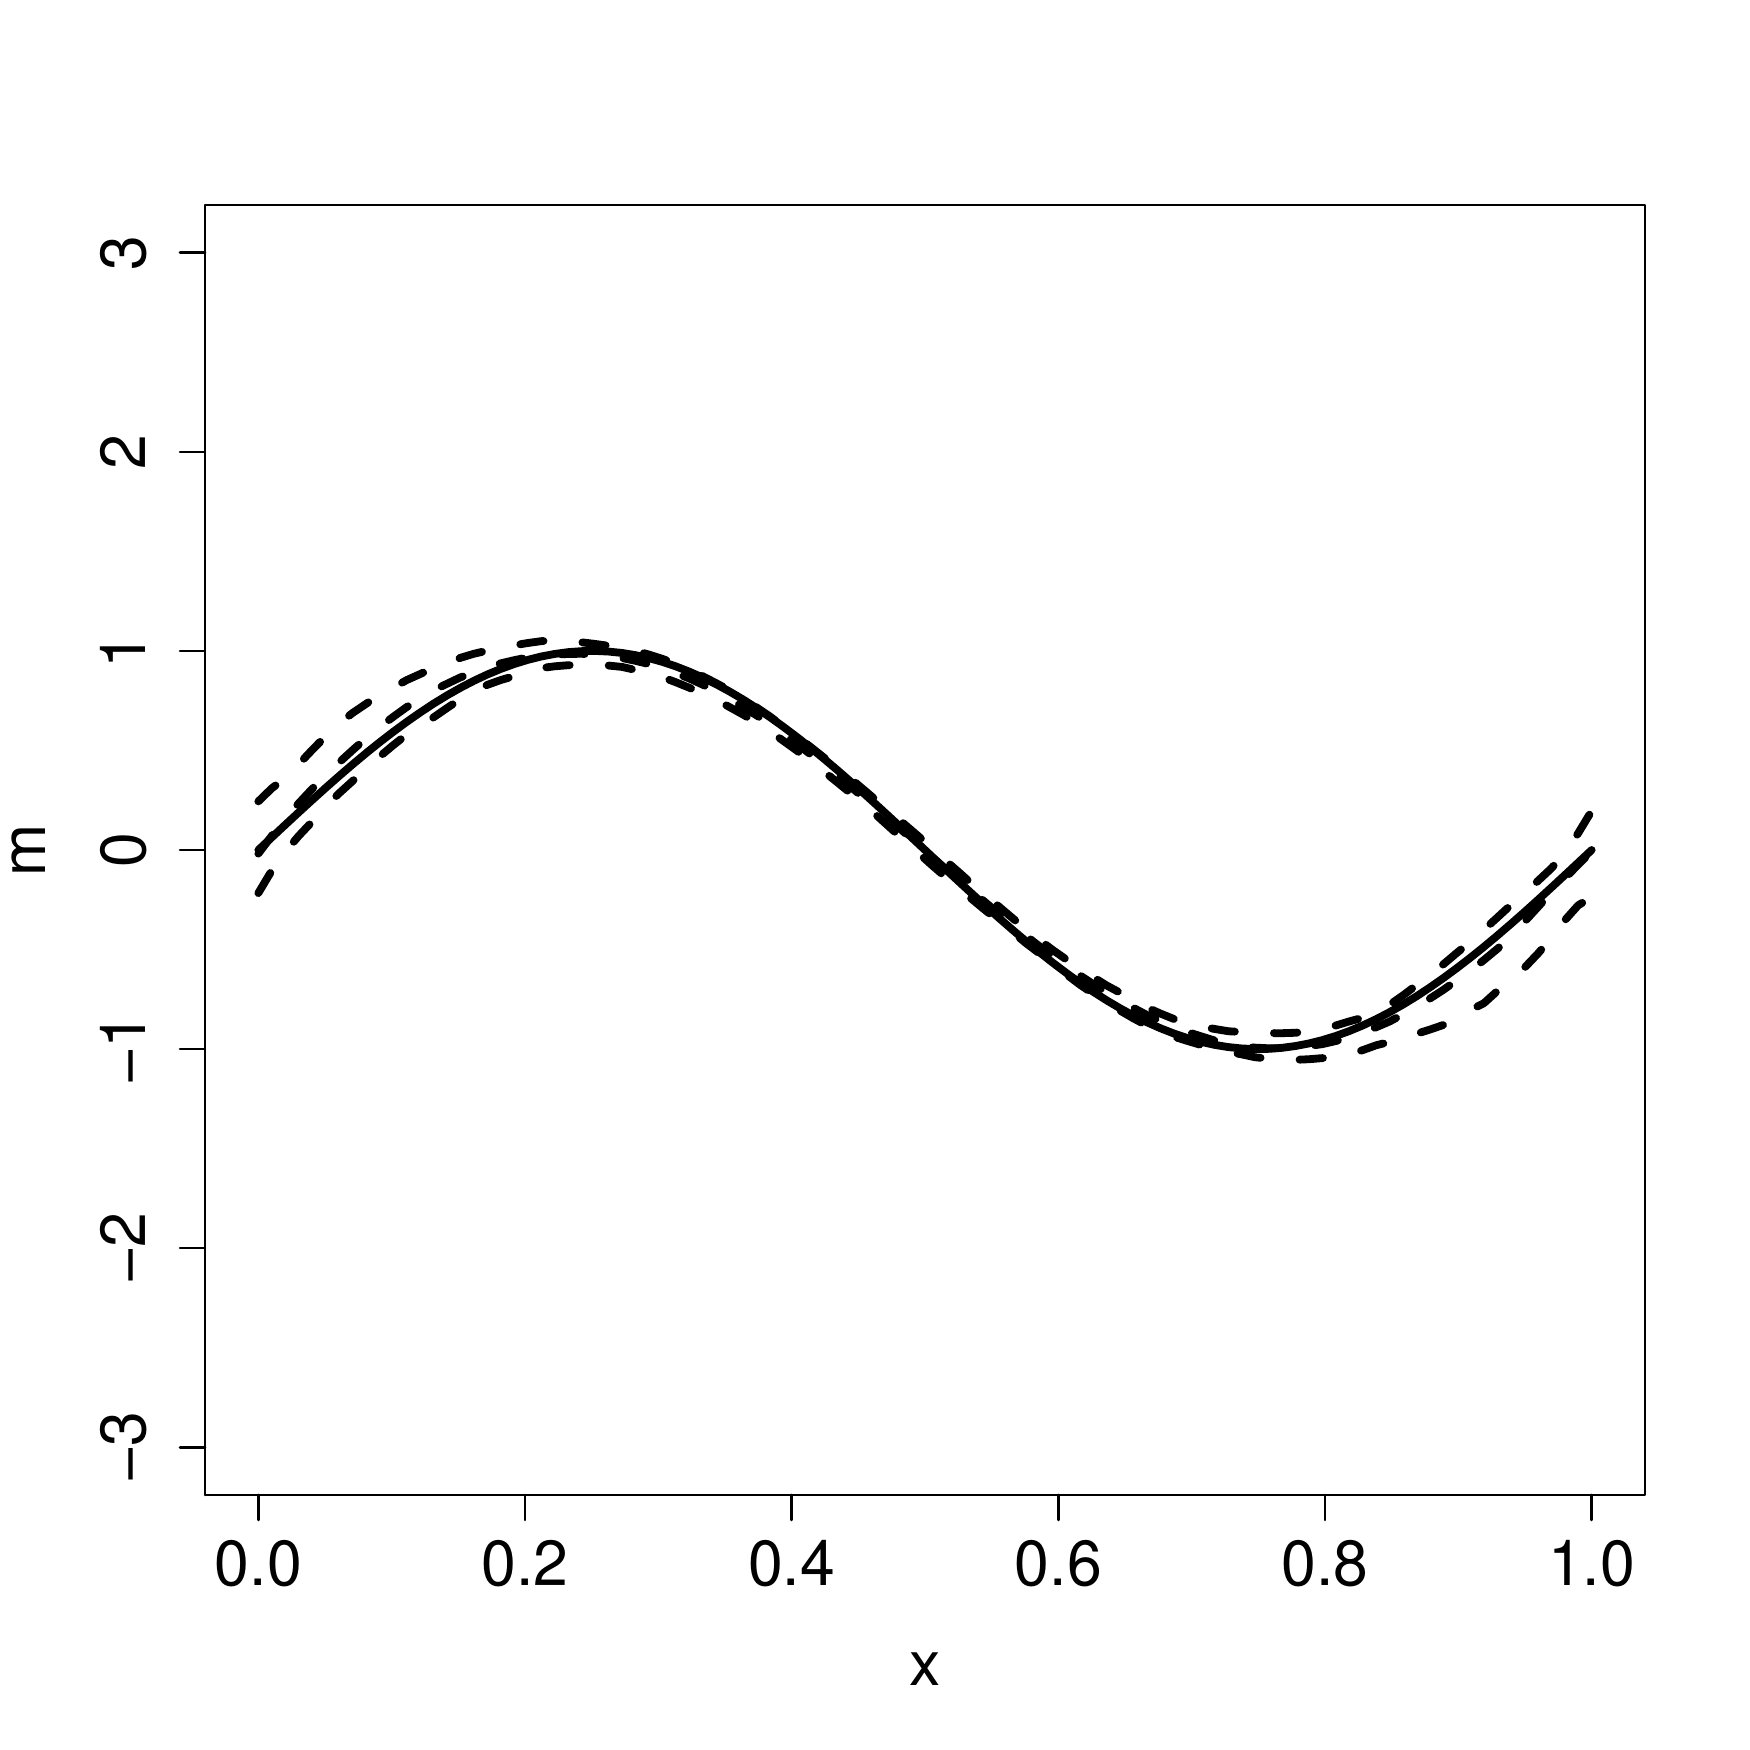}
\includegraphics[scale = 0.35]{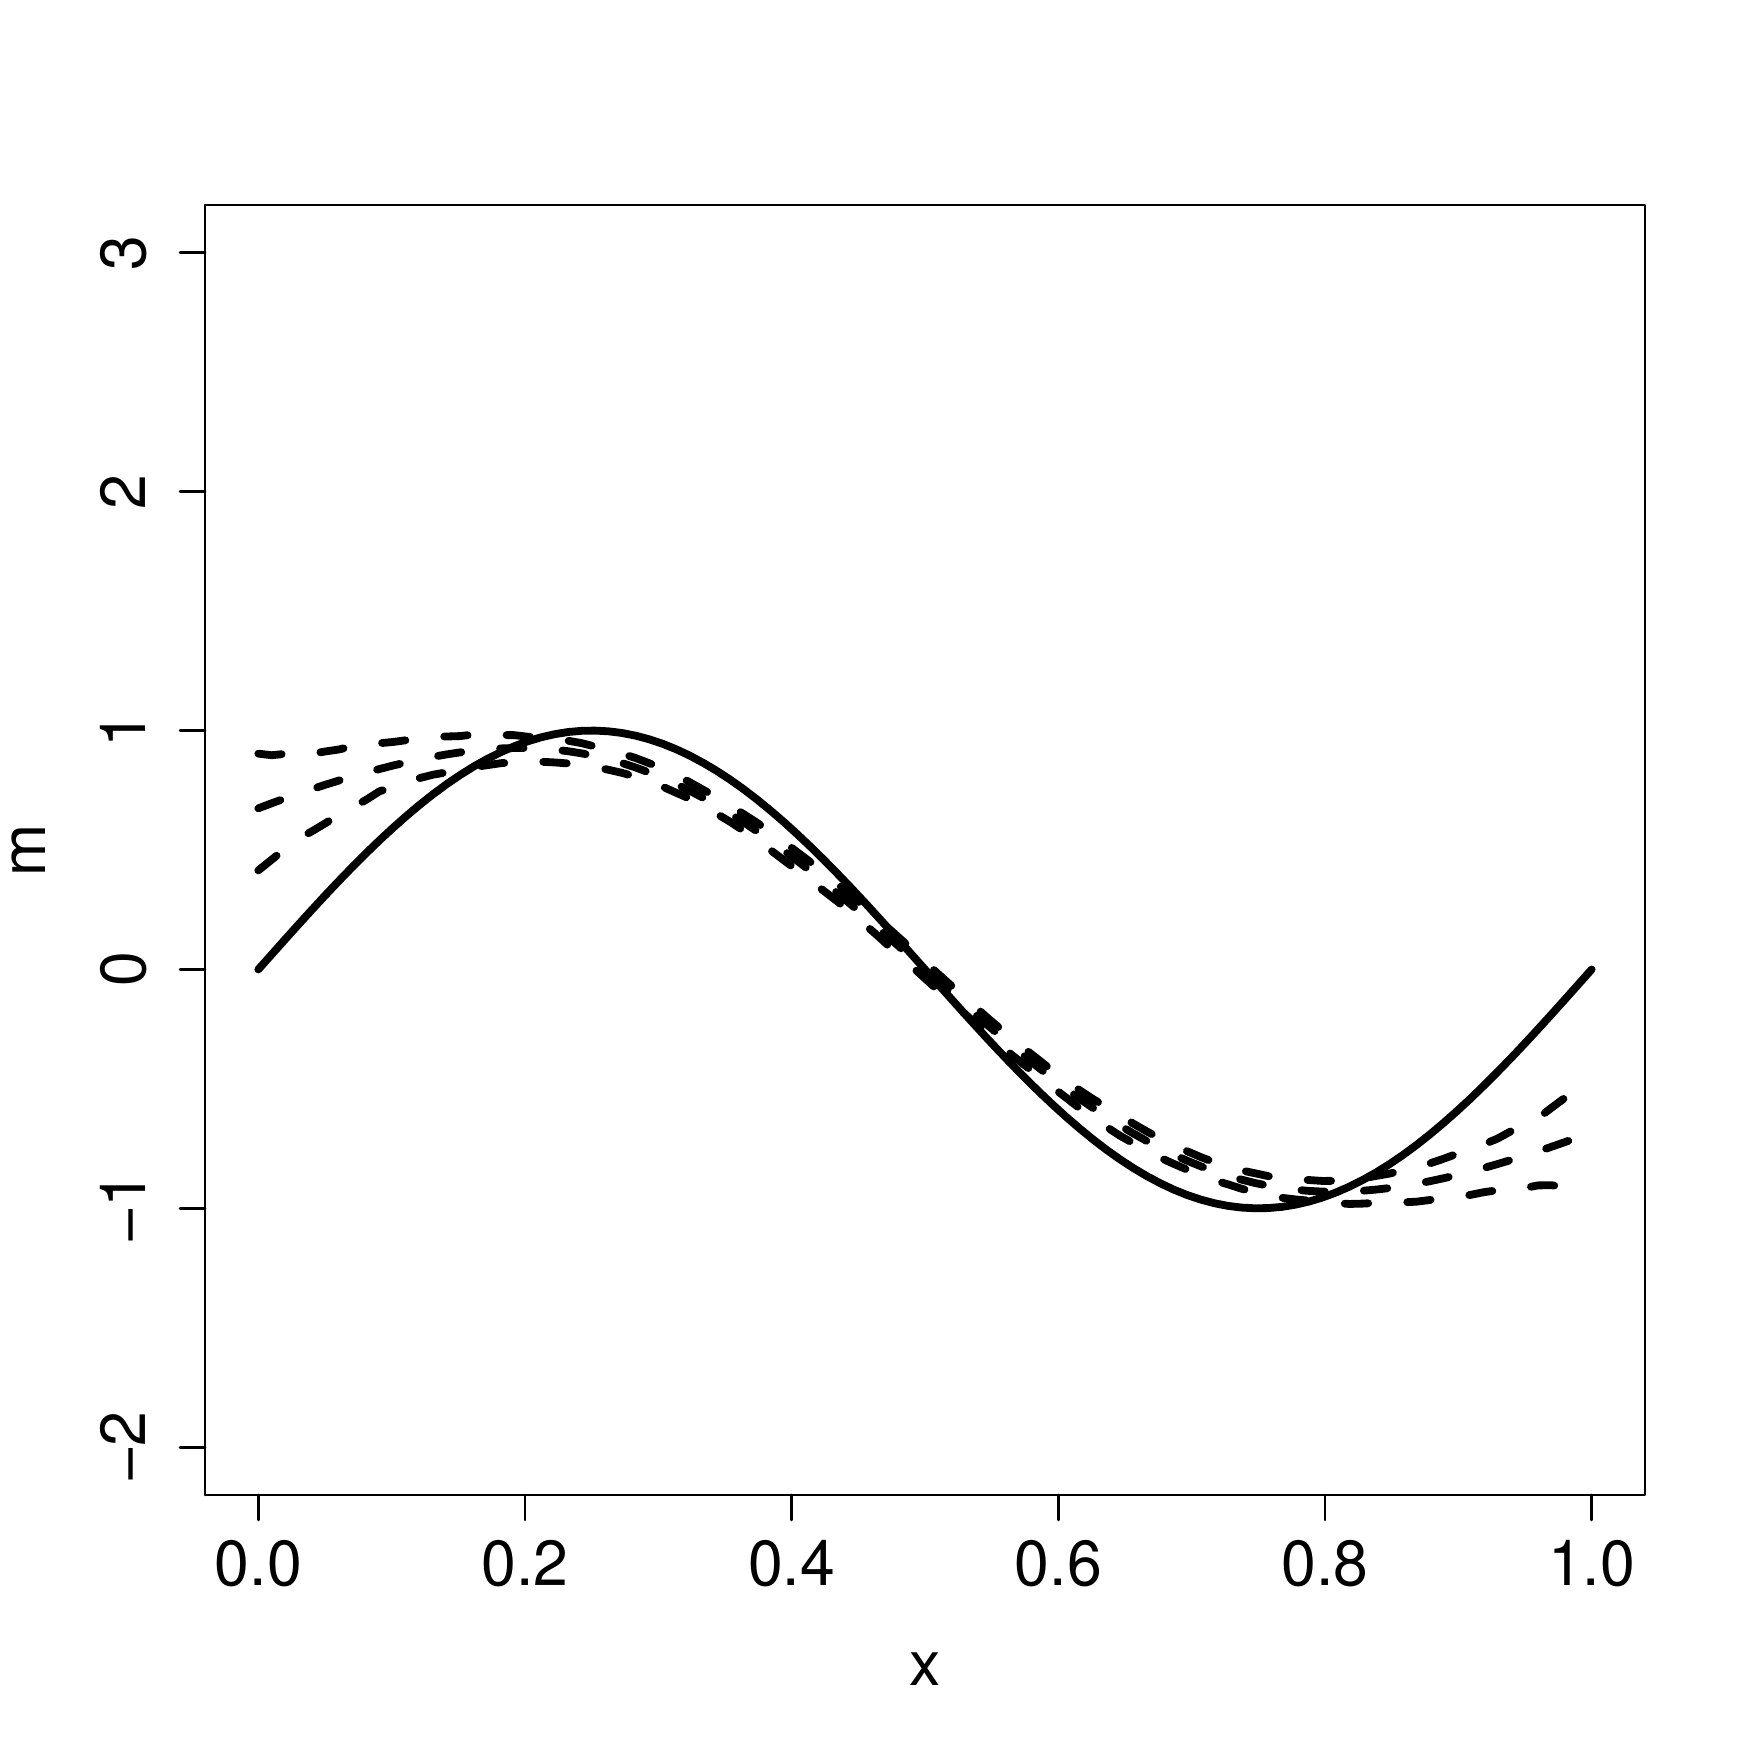}\\
\includegraphics[scale = 0.35]{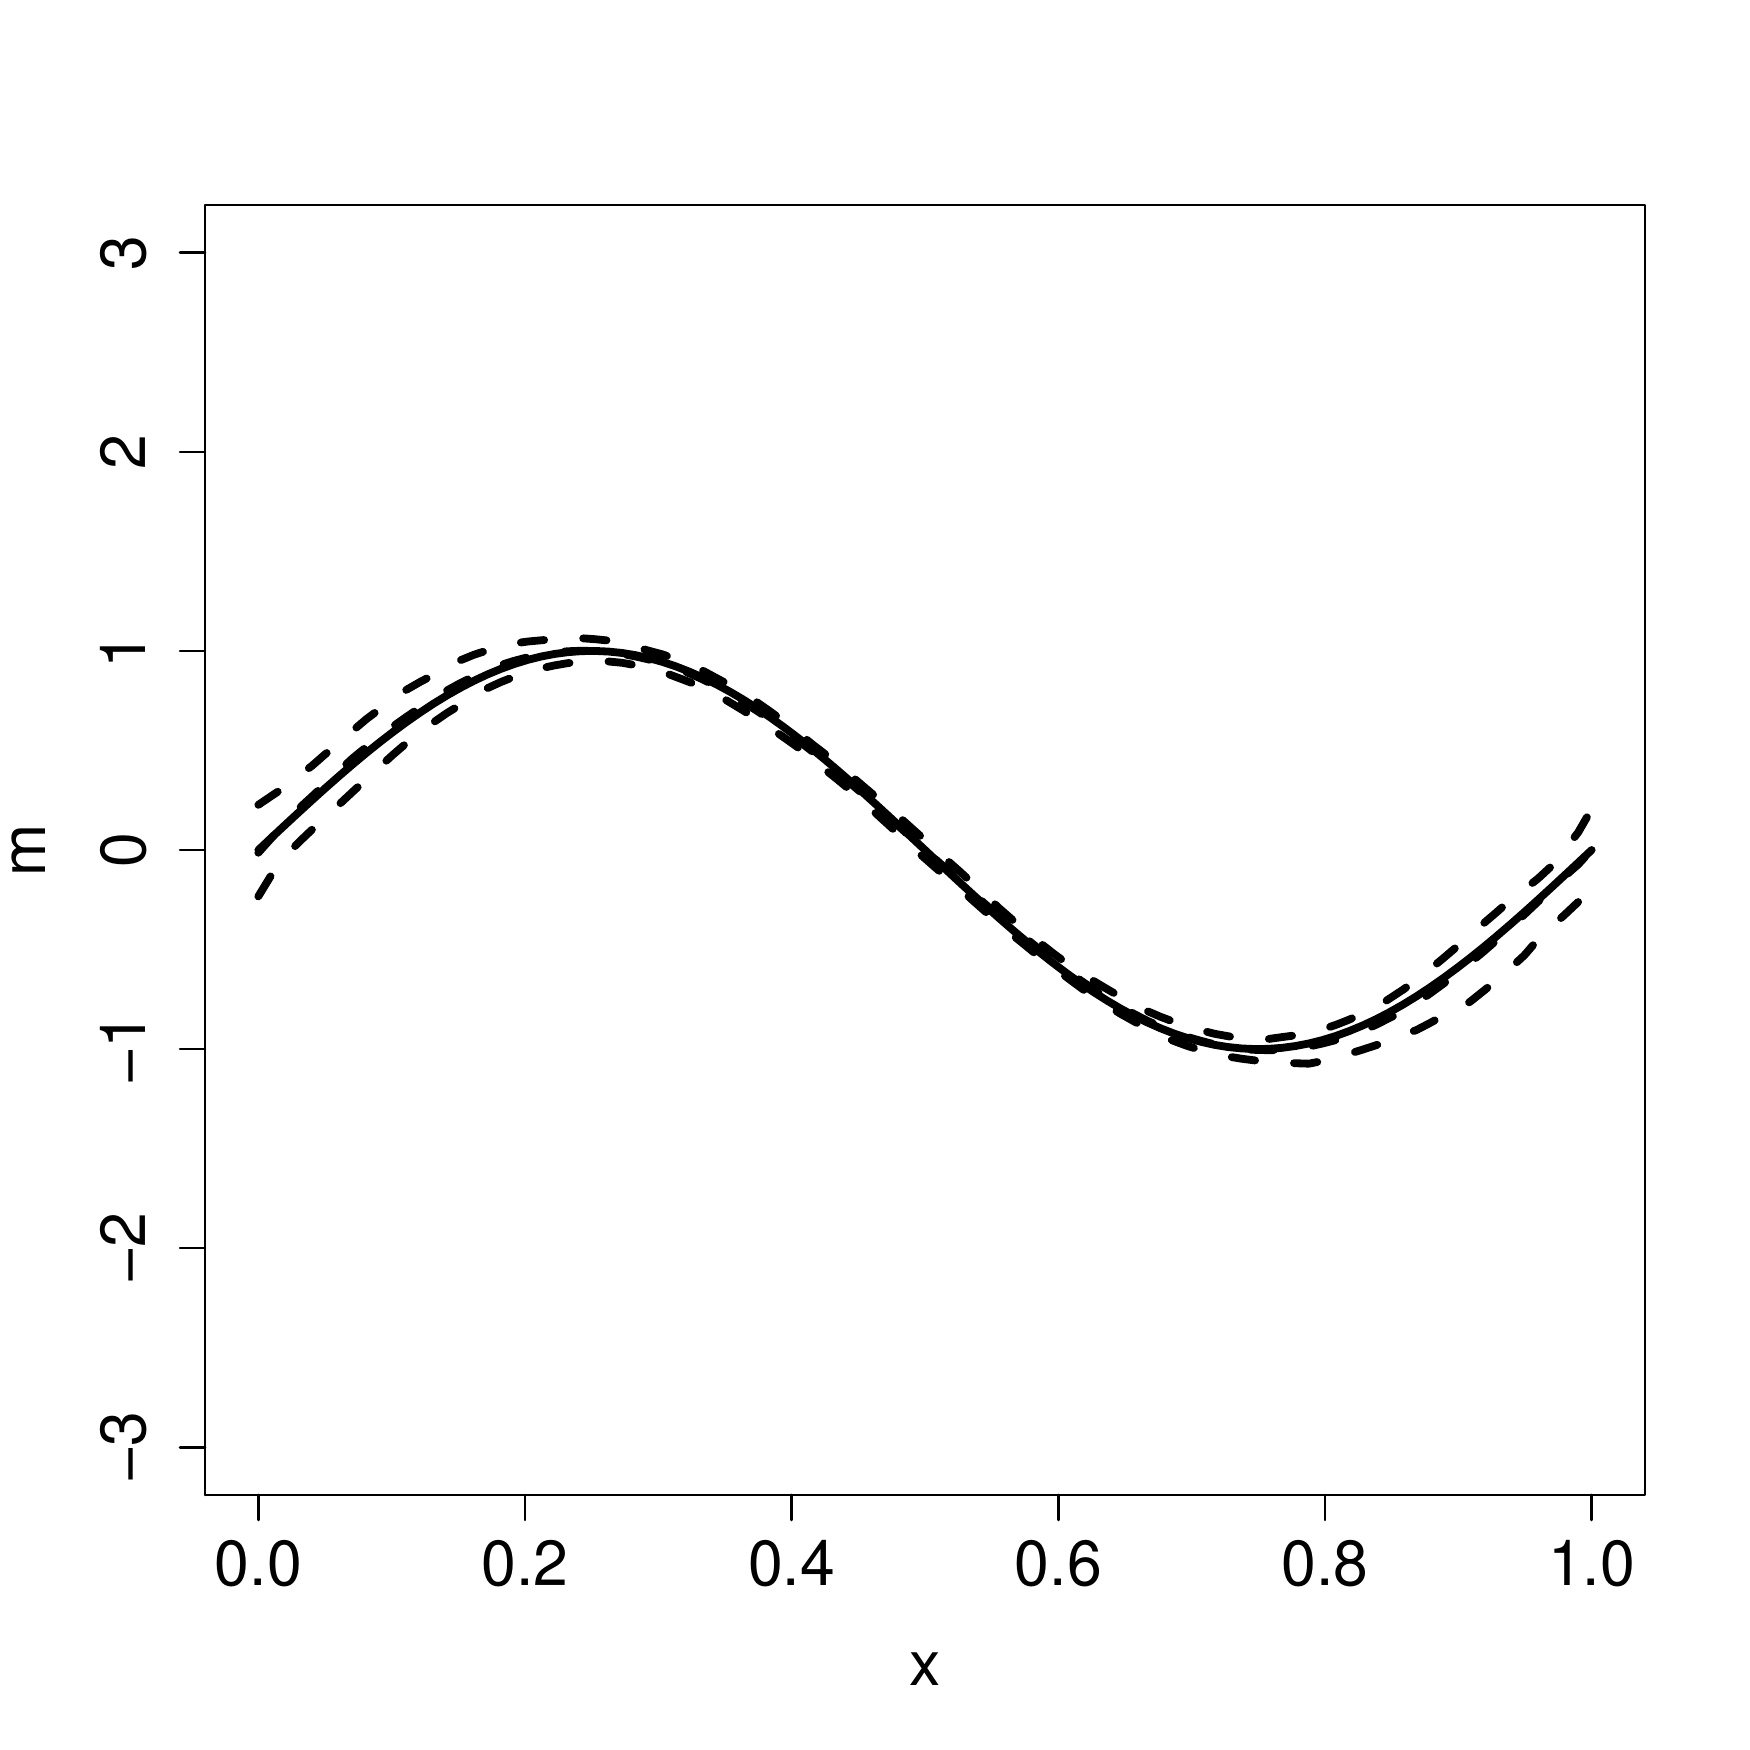}
\includegraphics[scale = 0.35]{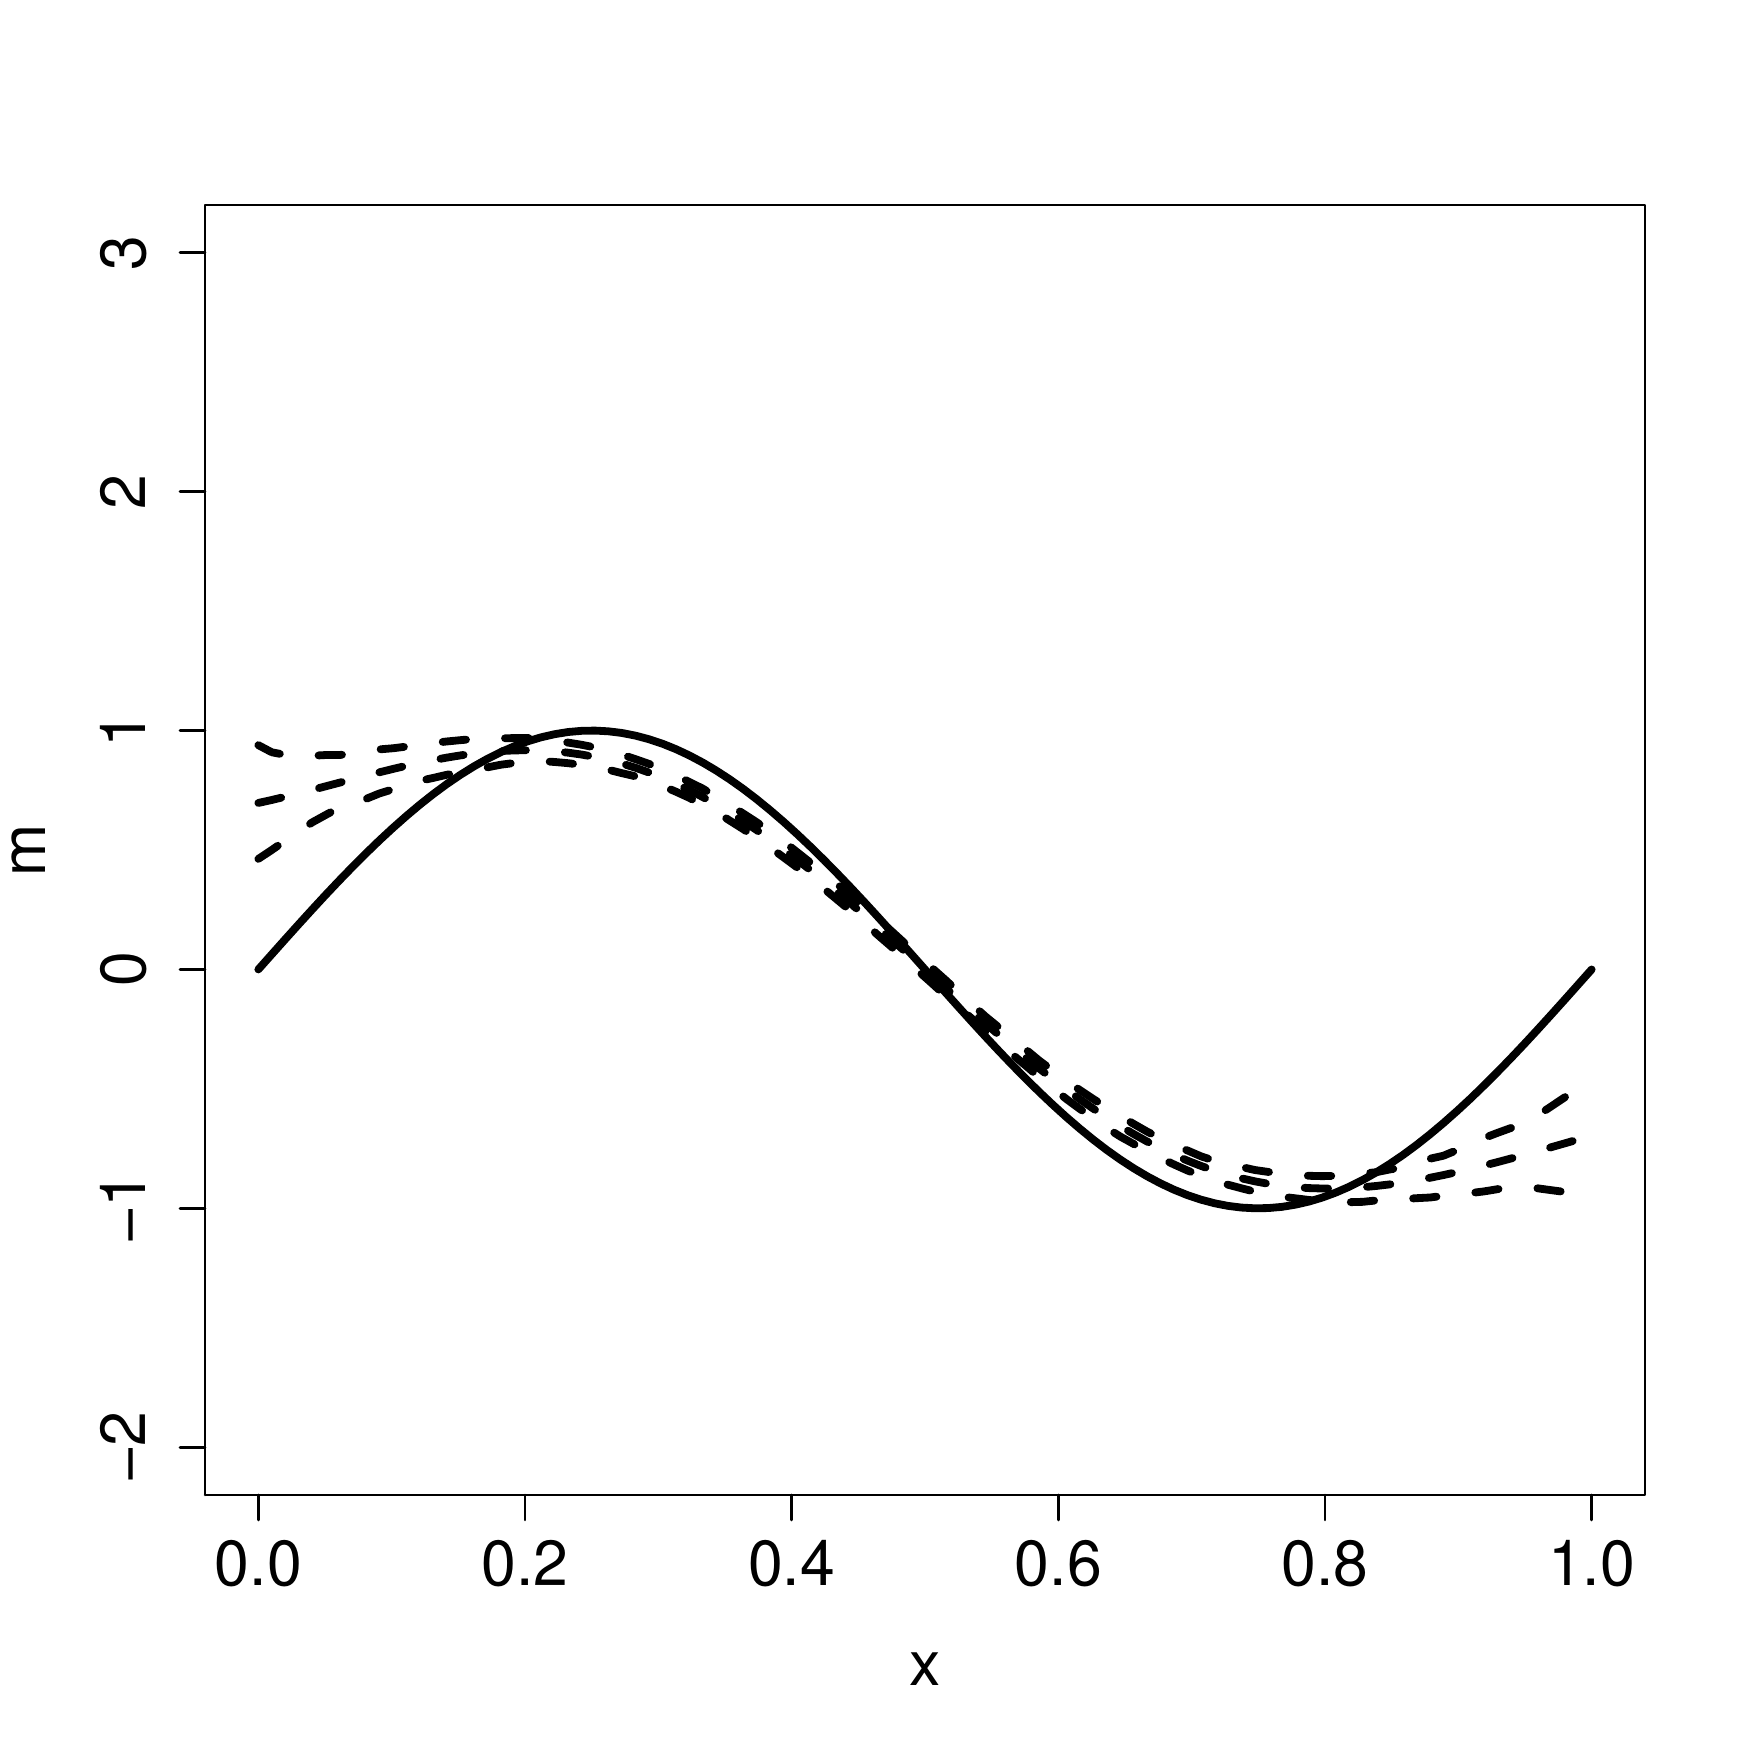}\\
\includegraphics[scale = 0.35]{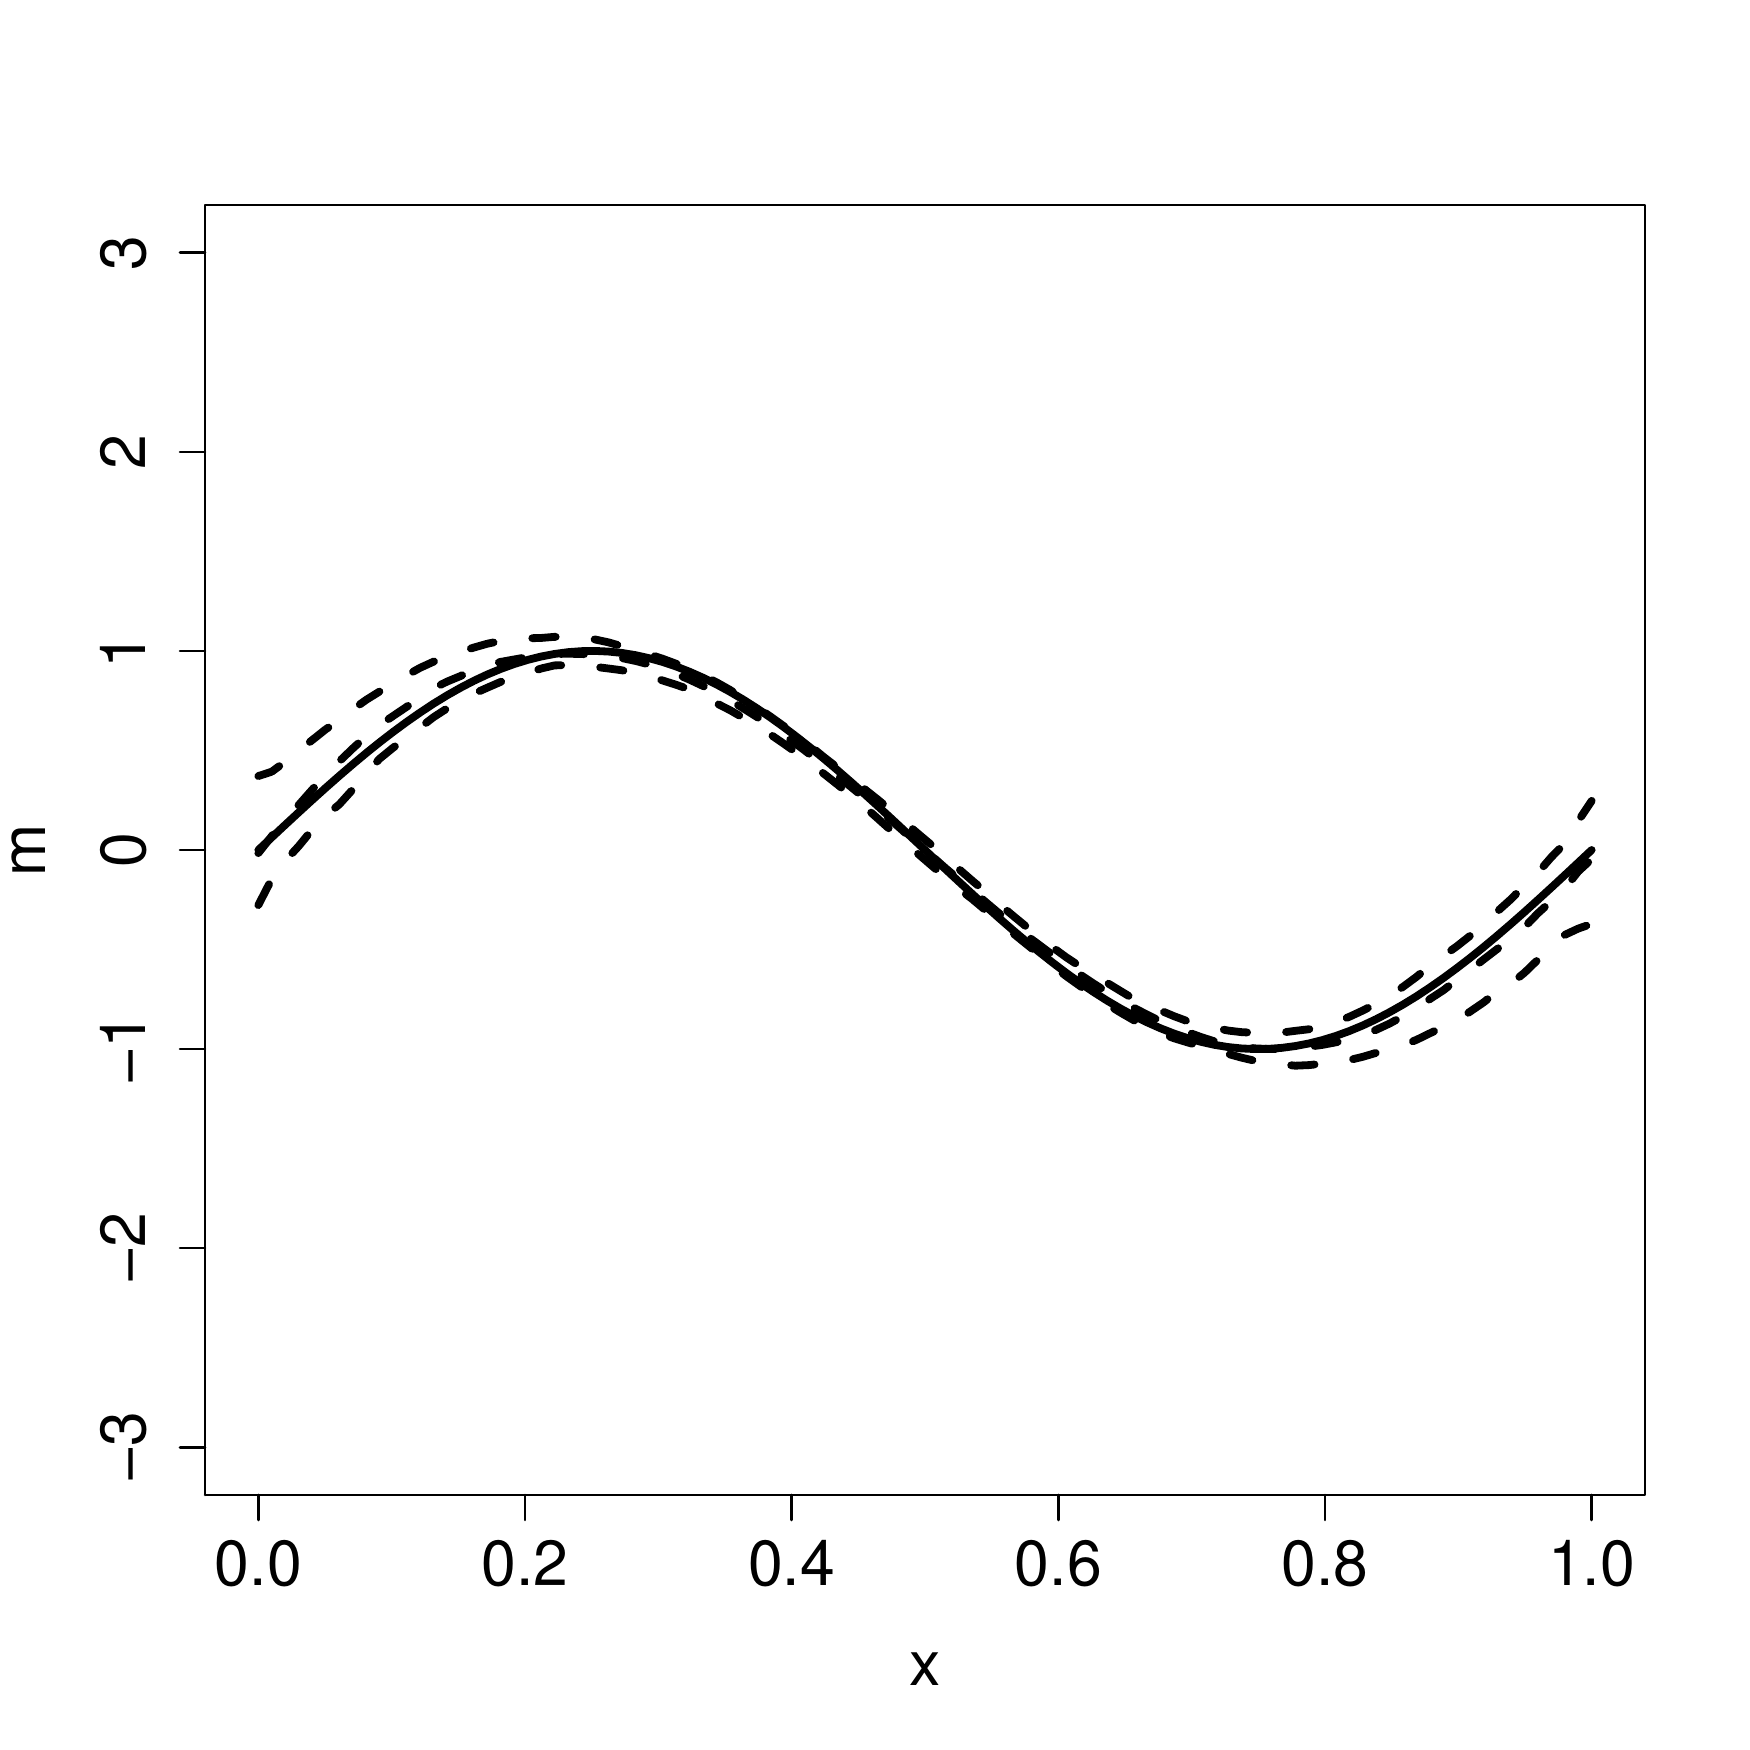}
\includegraphics[scale = 0.35]{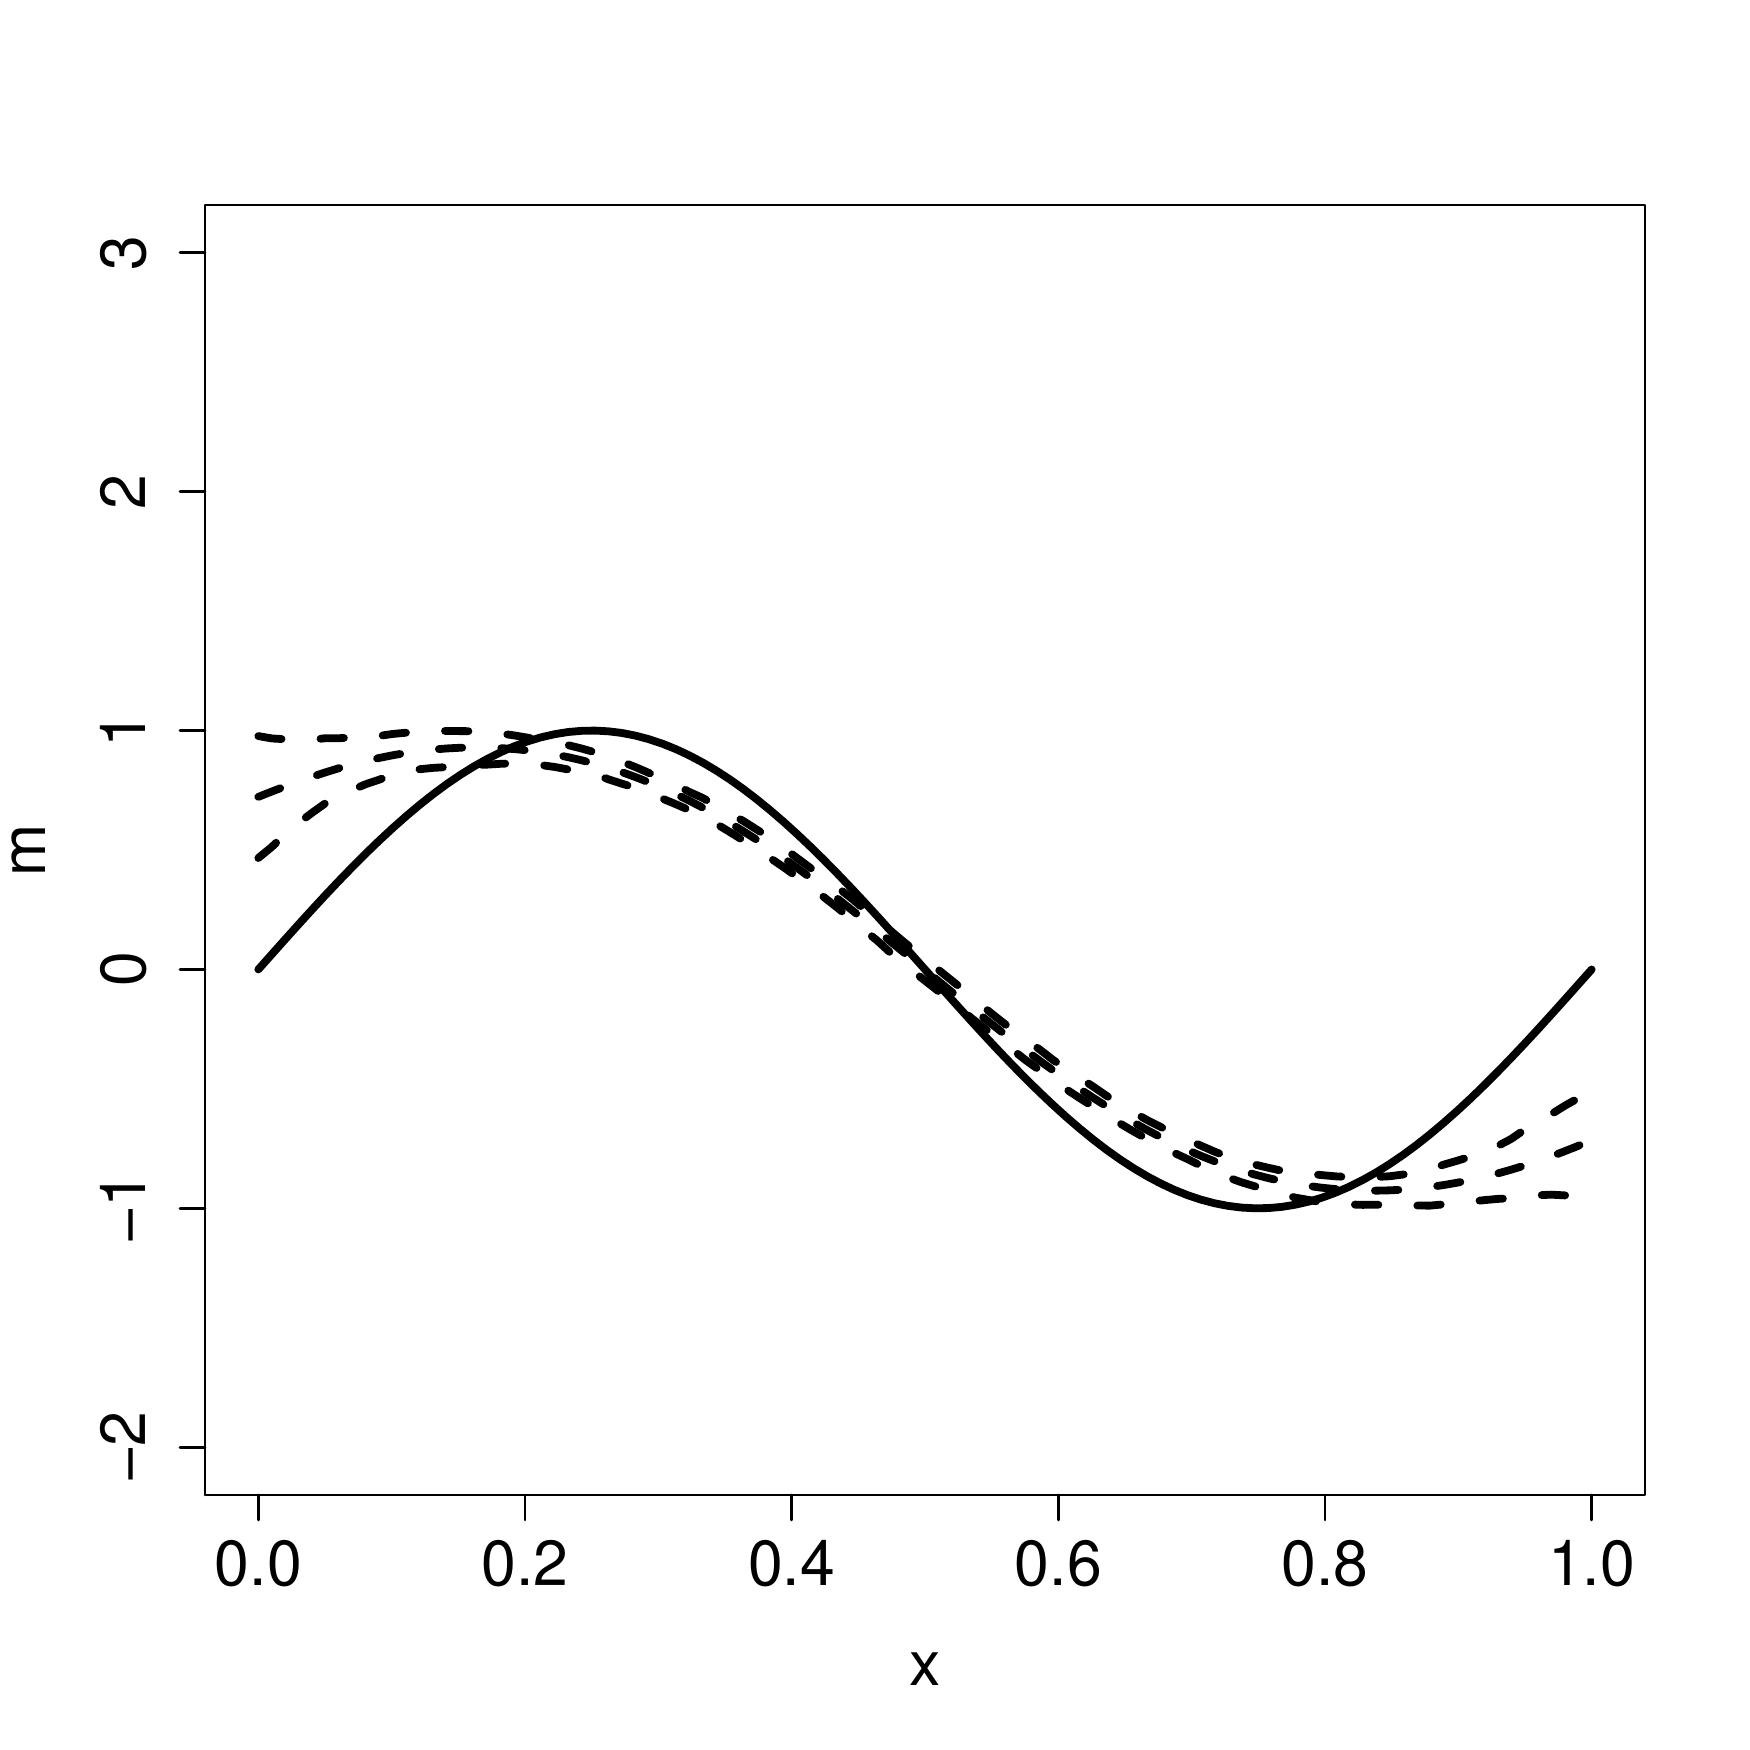}
\end{center}
\end{figure}

\begin{figure}[!h]
\caption{Bspline semiparametric regression estimation (left) and 
deconvolution estimation (right) 
from 200 
  simulations: The solid lines represent the true functions and the 
  dash lines represent the estimated functions and their 90\%
  confidence bands. The first row to third row are the results for 
  model II (a)--(c), respectively. Sample size 200.}
{\label{fig:mean0}}
\begin{center}
\includegraphics[scale = 0.35]{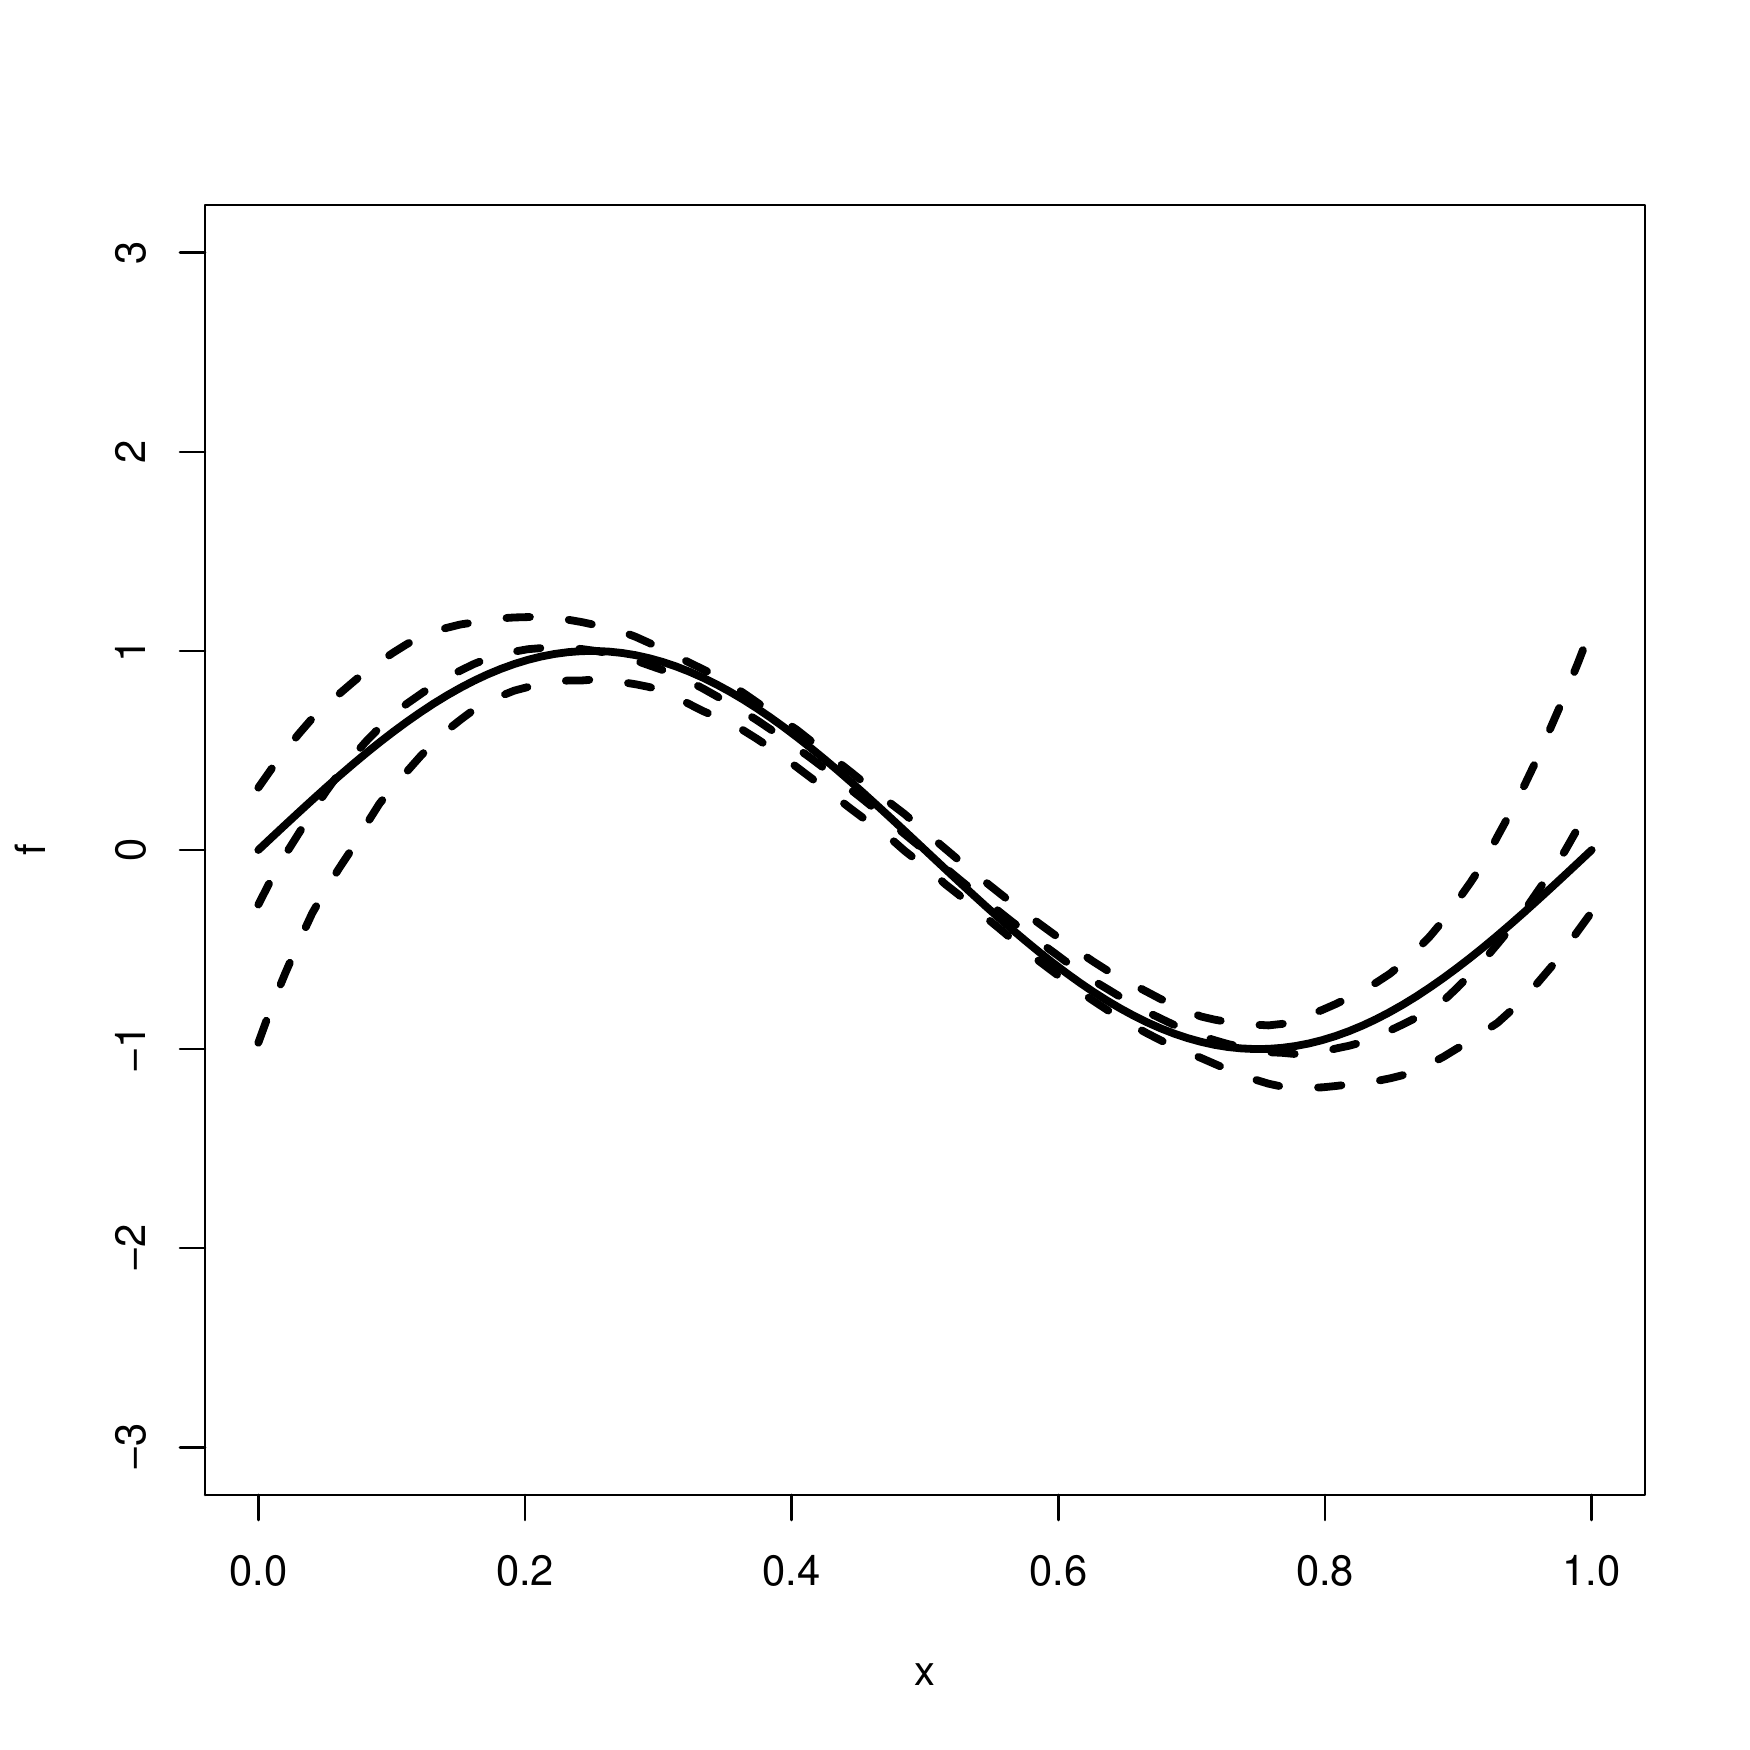}
\includegraphics[scale = 0.35]{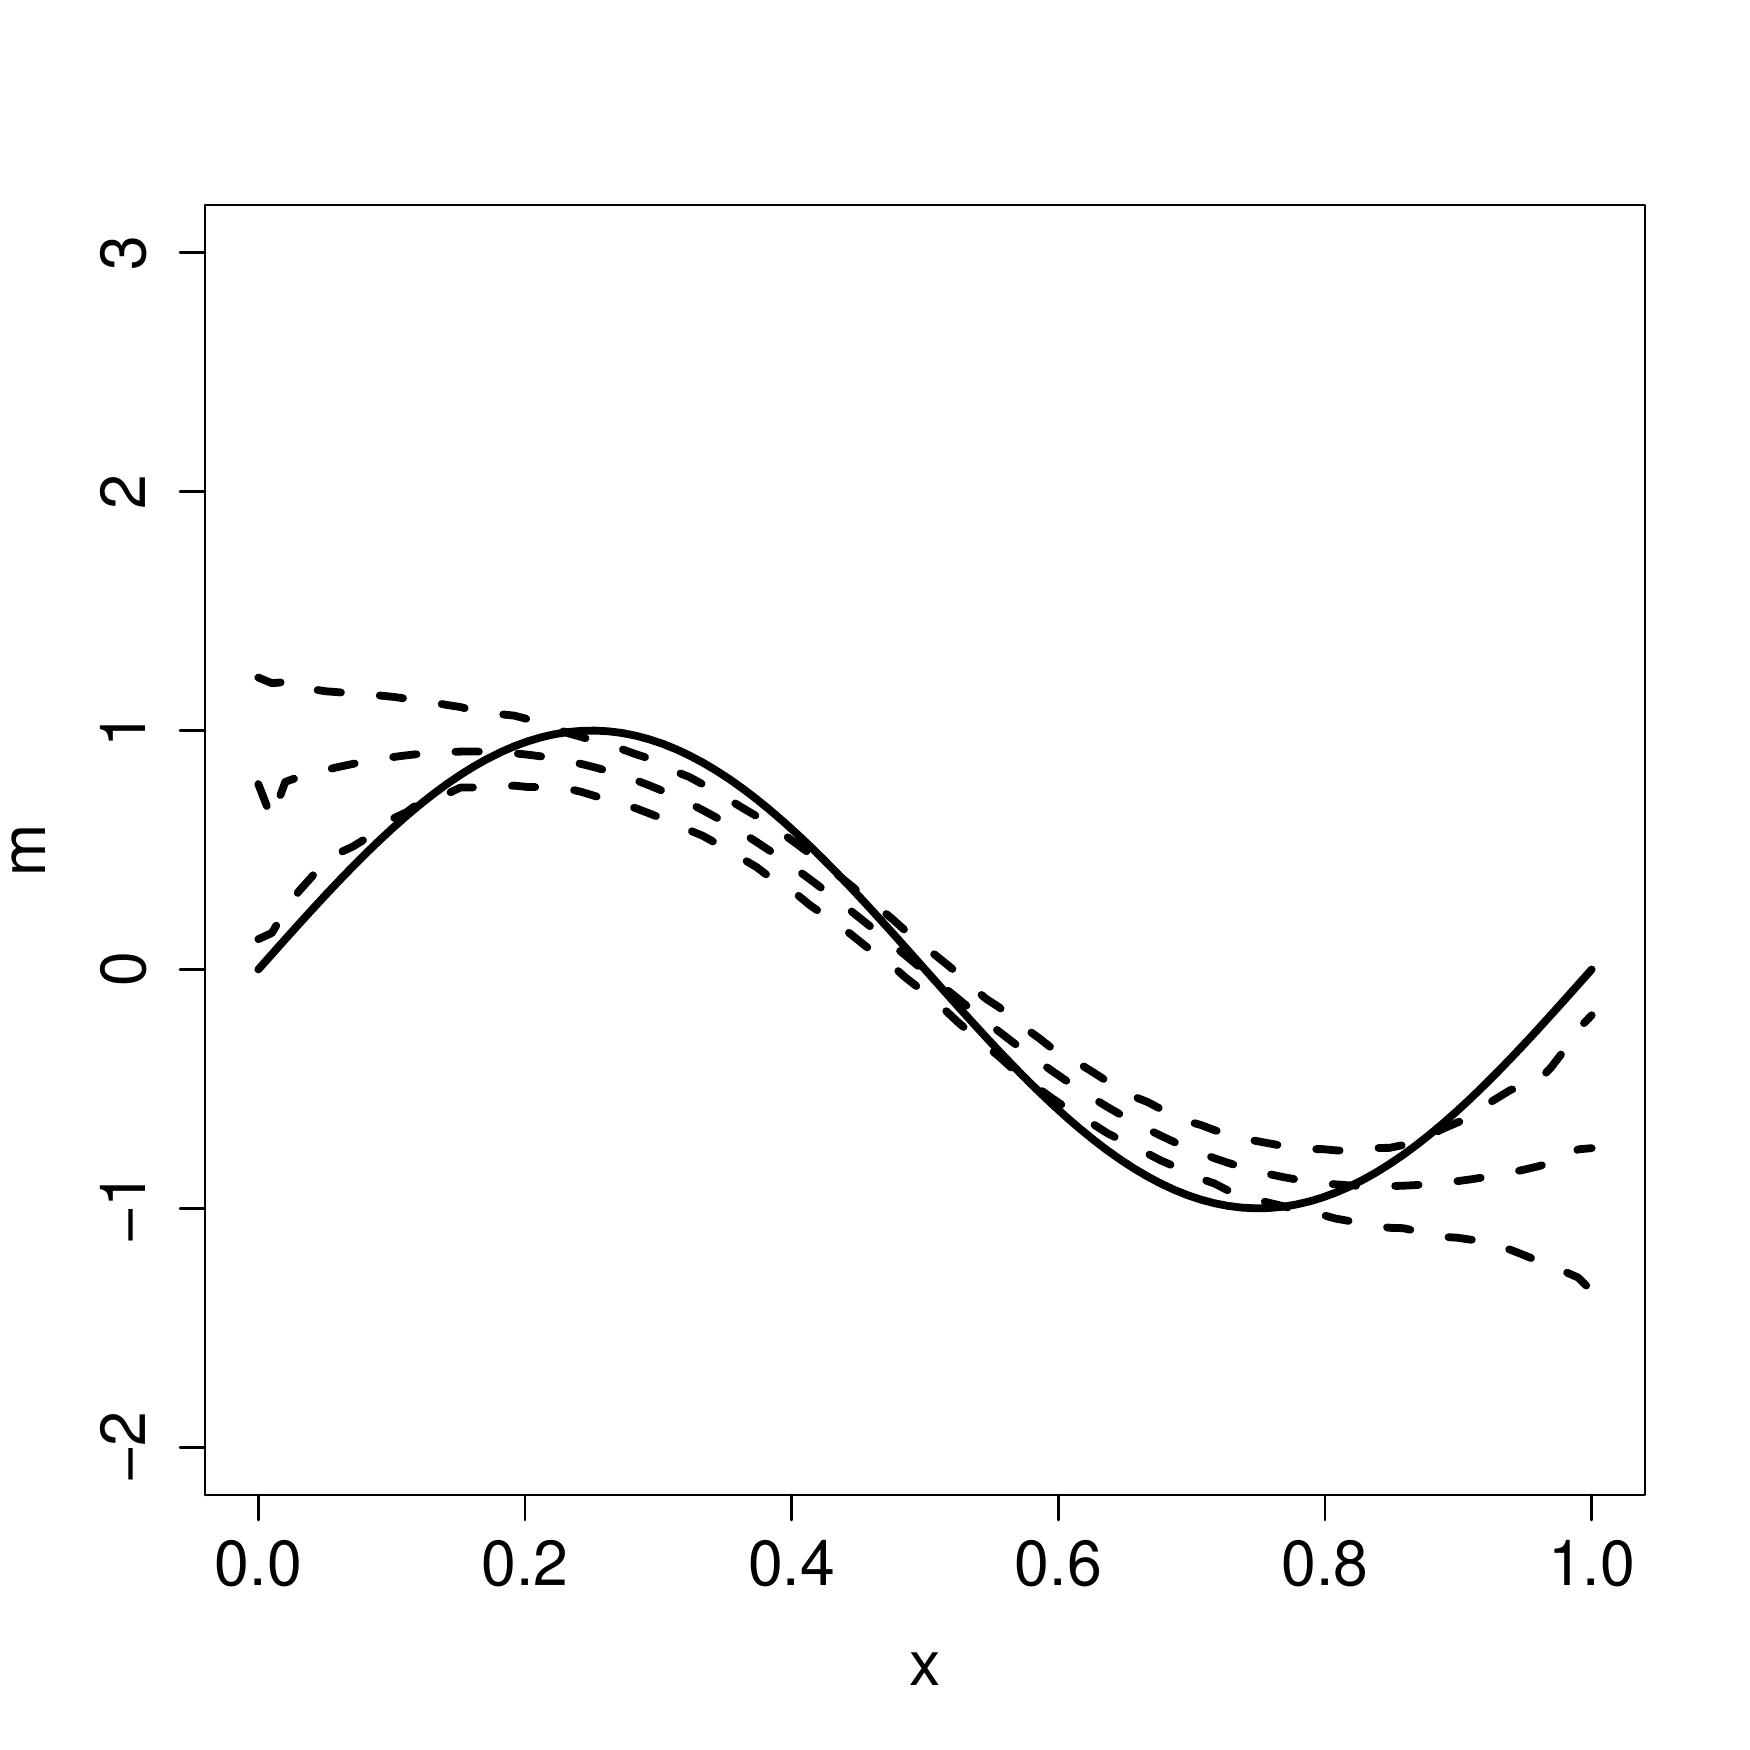}\\
\includegraphics[scale = 0.35]{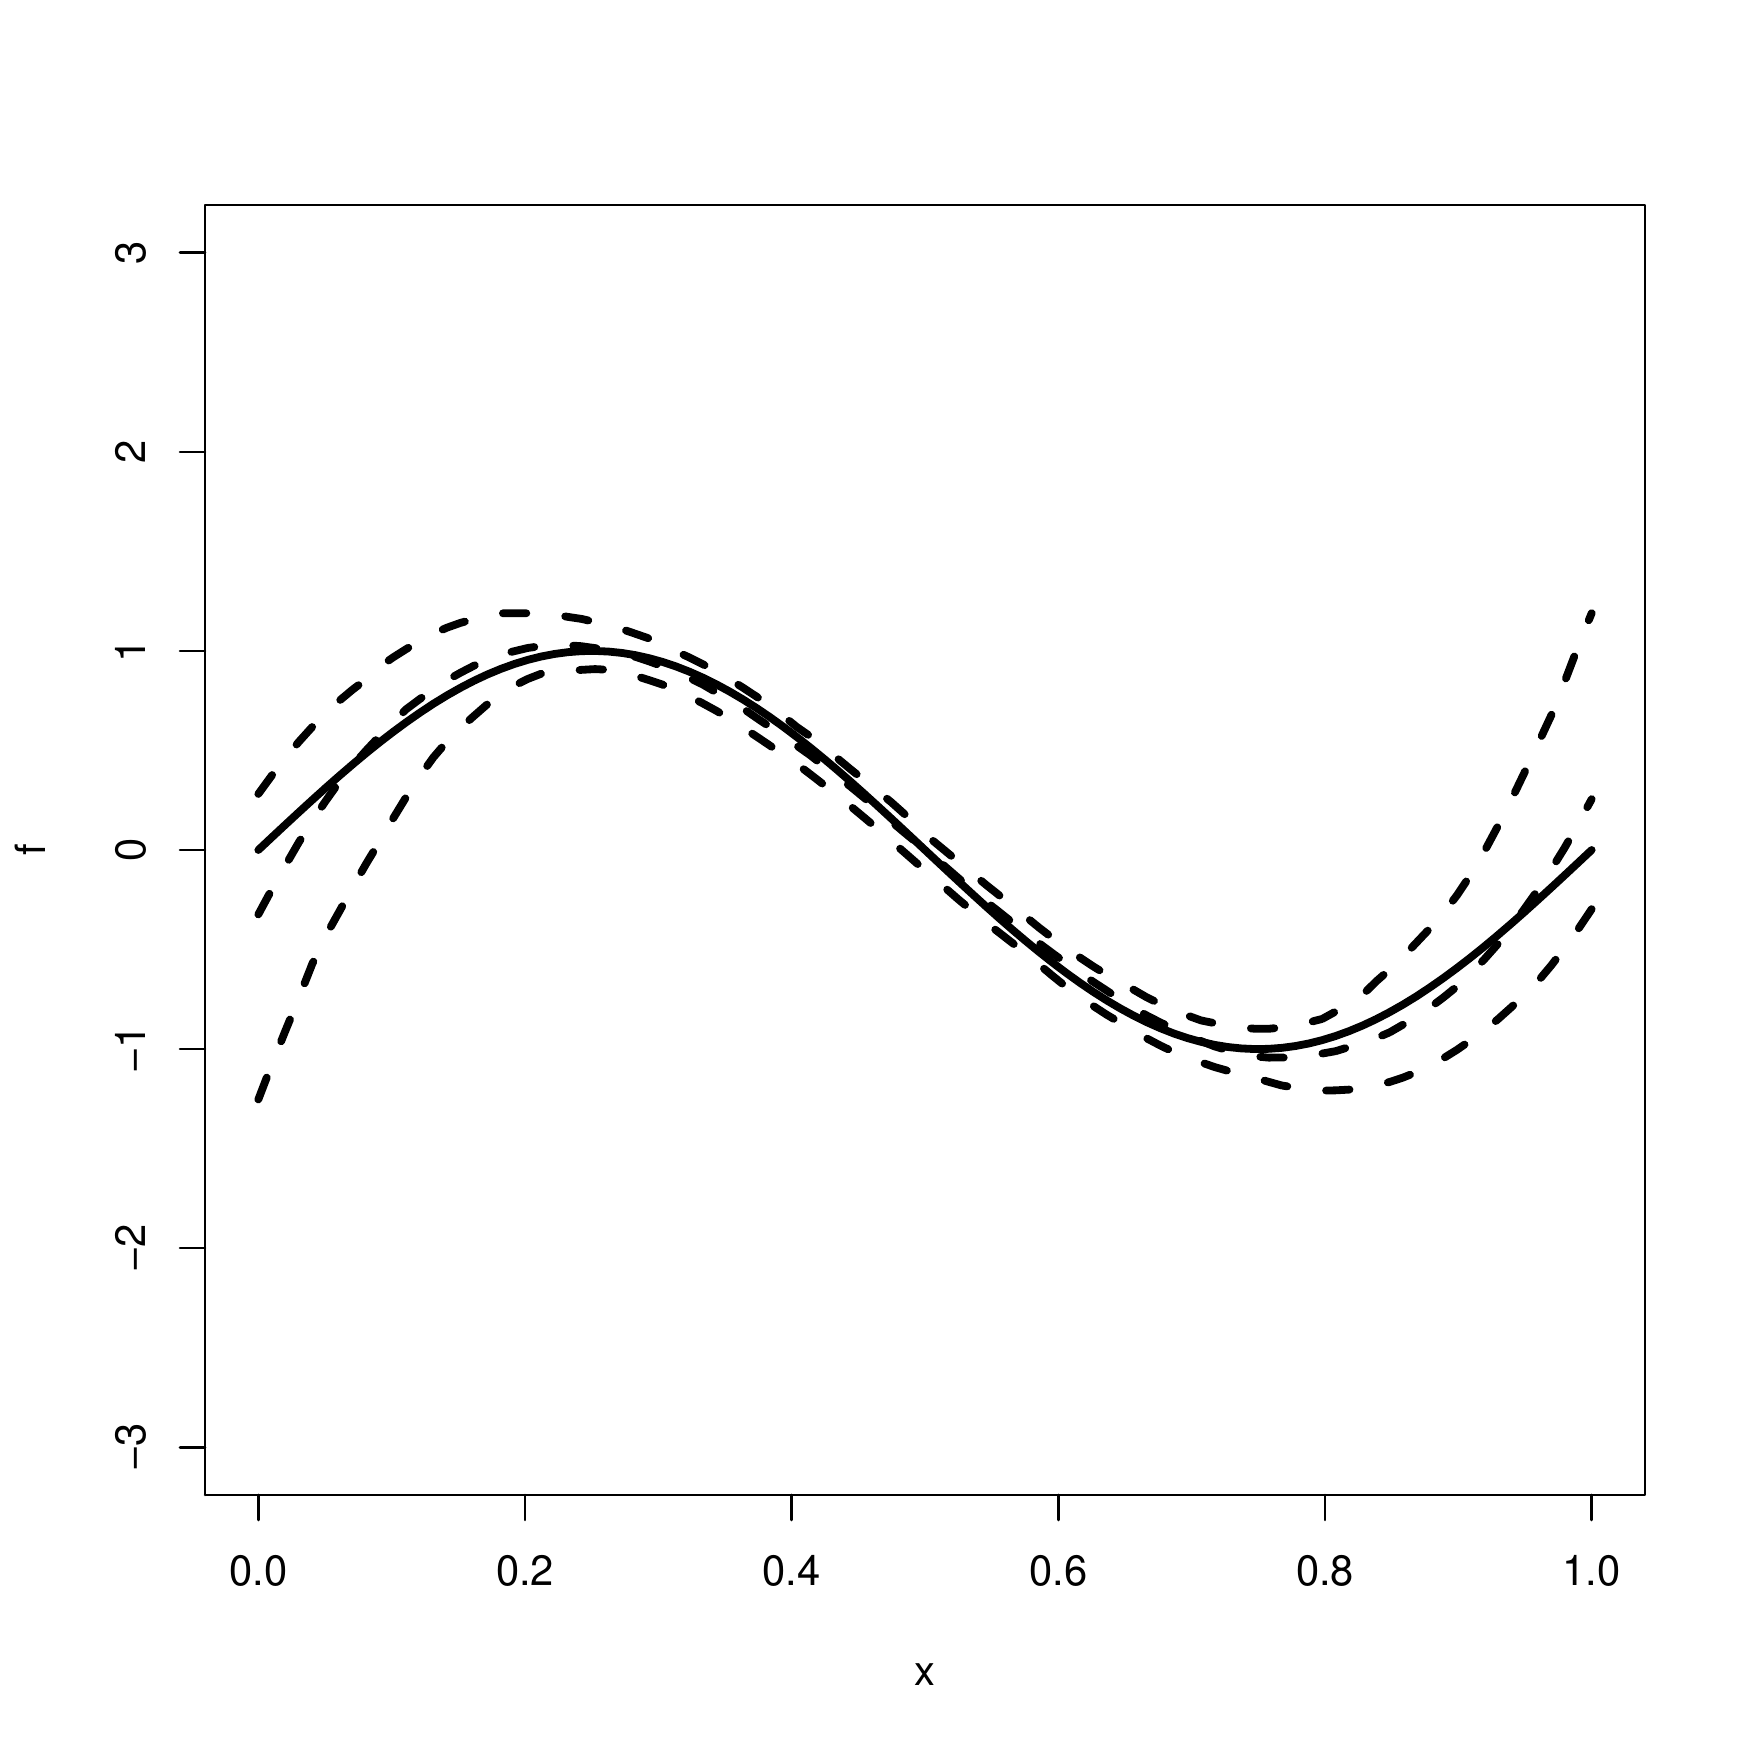}
\includegraphics[scale = 0.35]{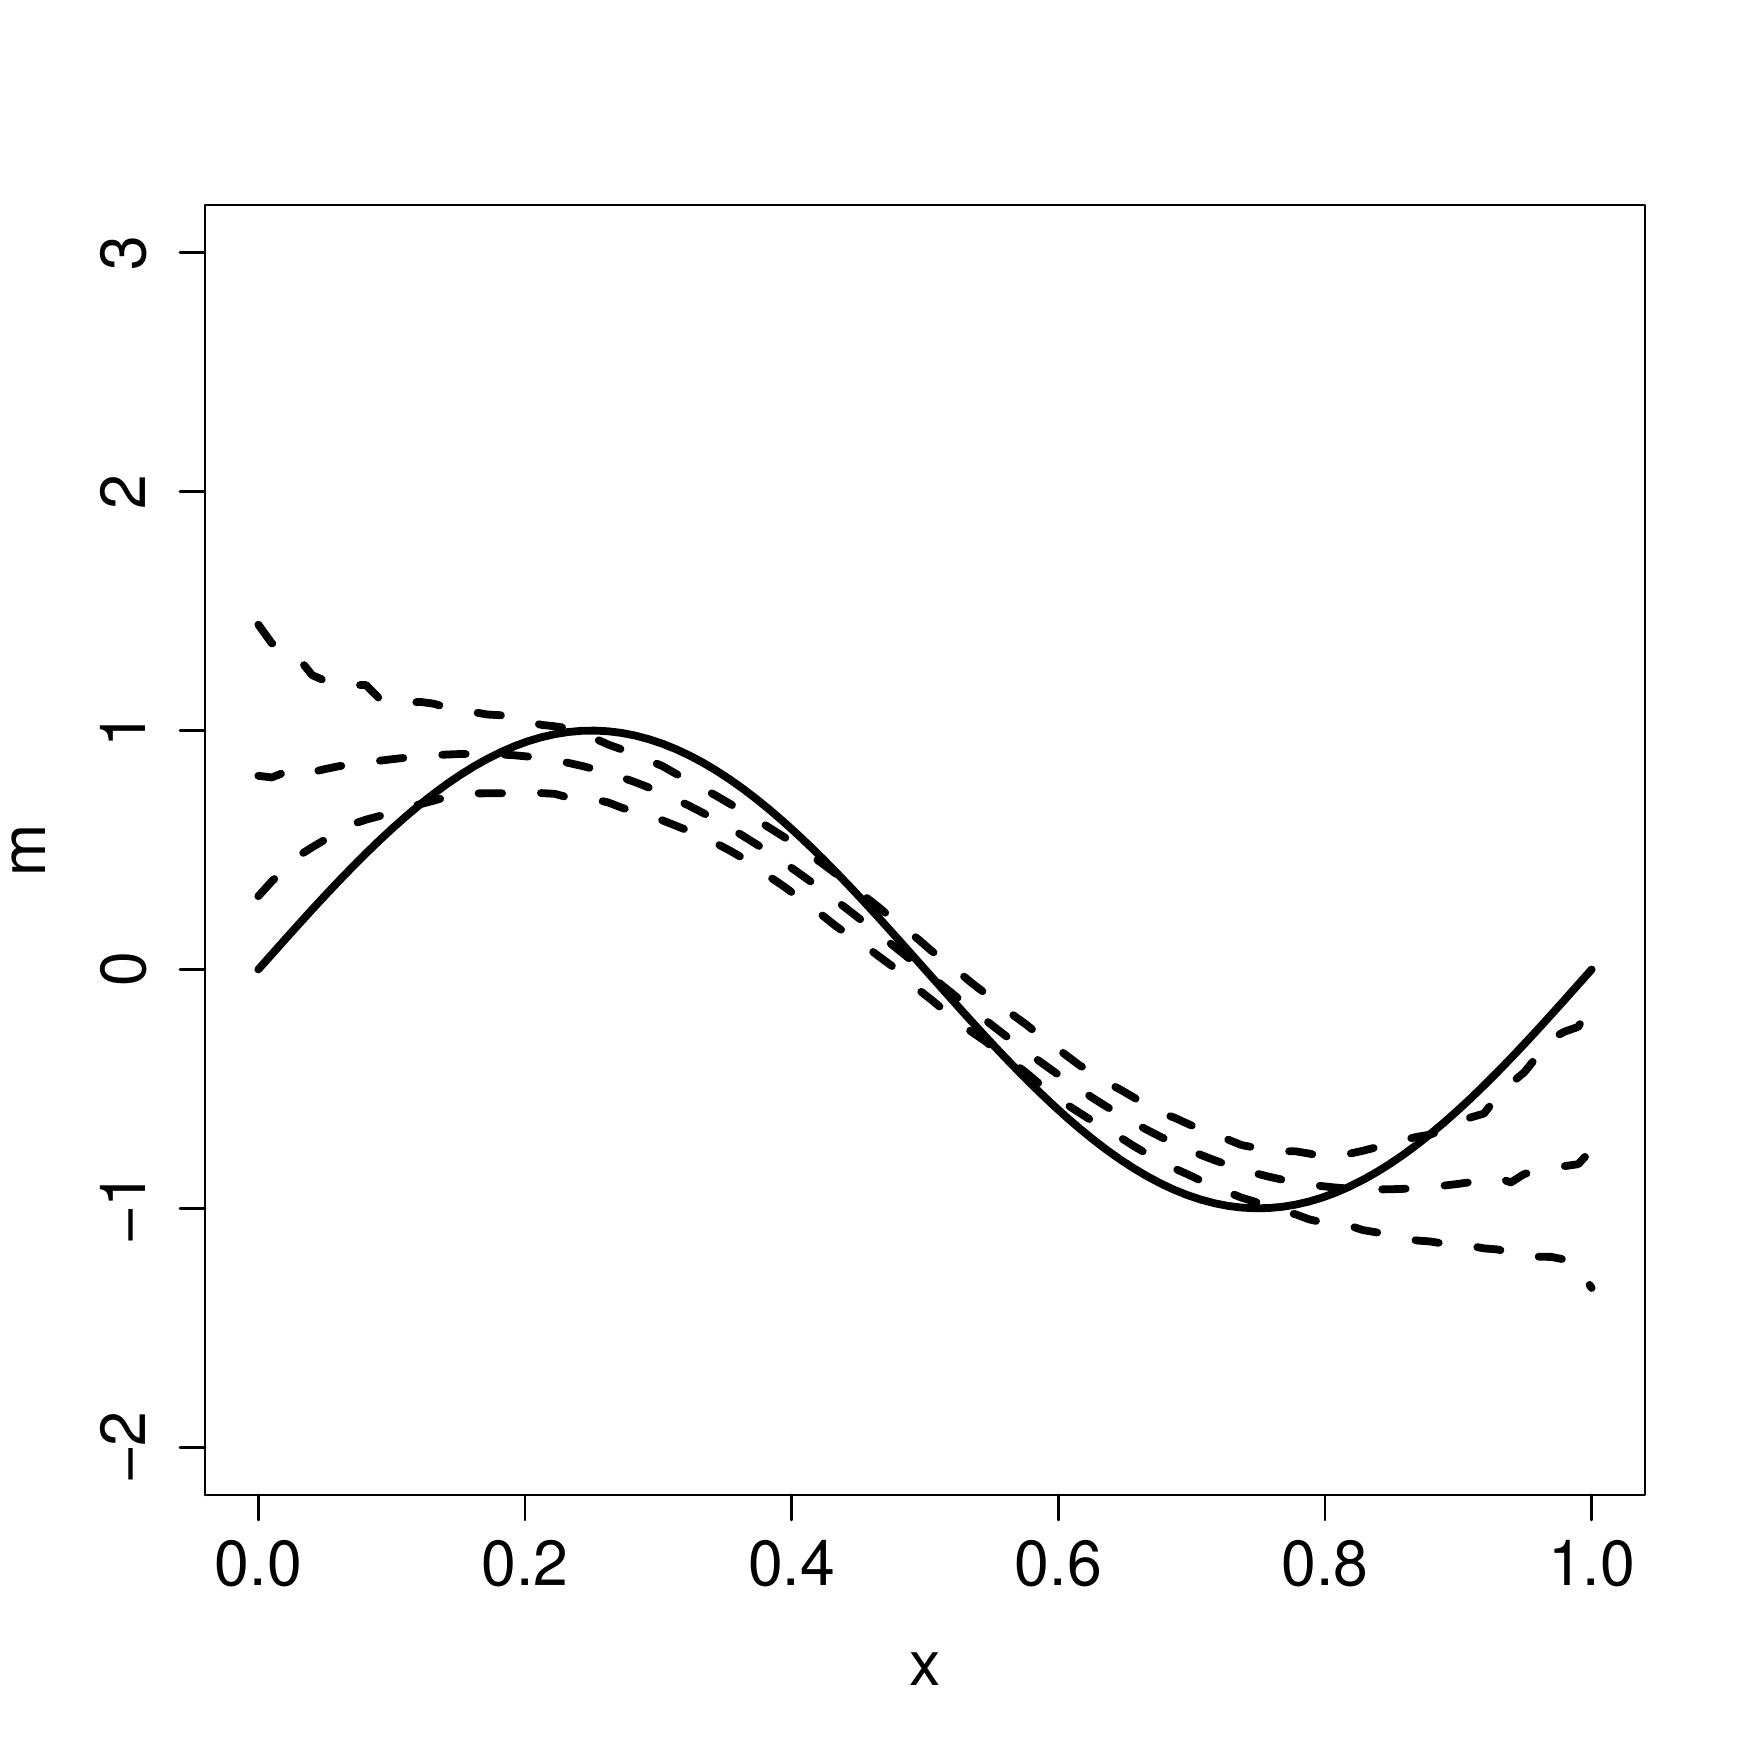}\\
\includegraphics[scale = 0.35]{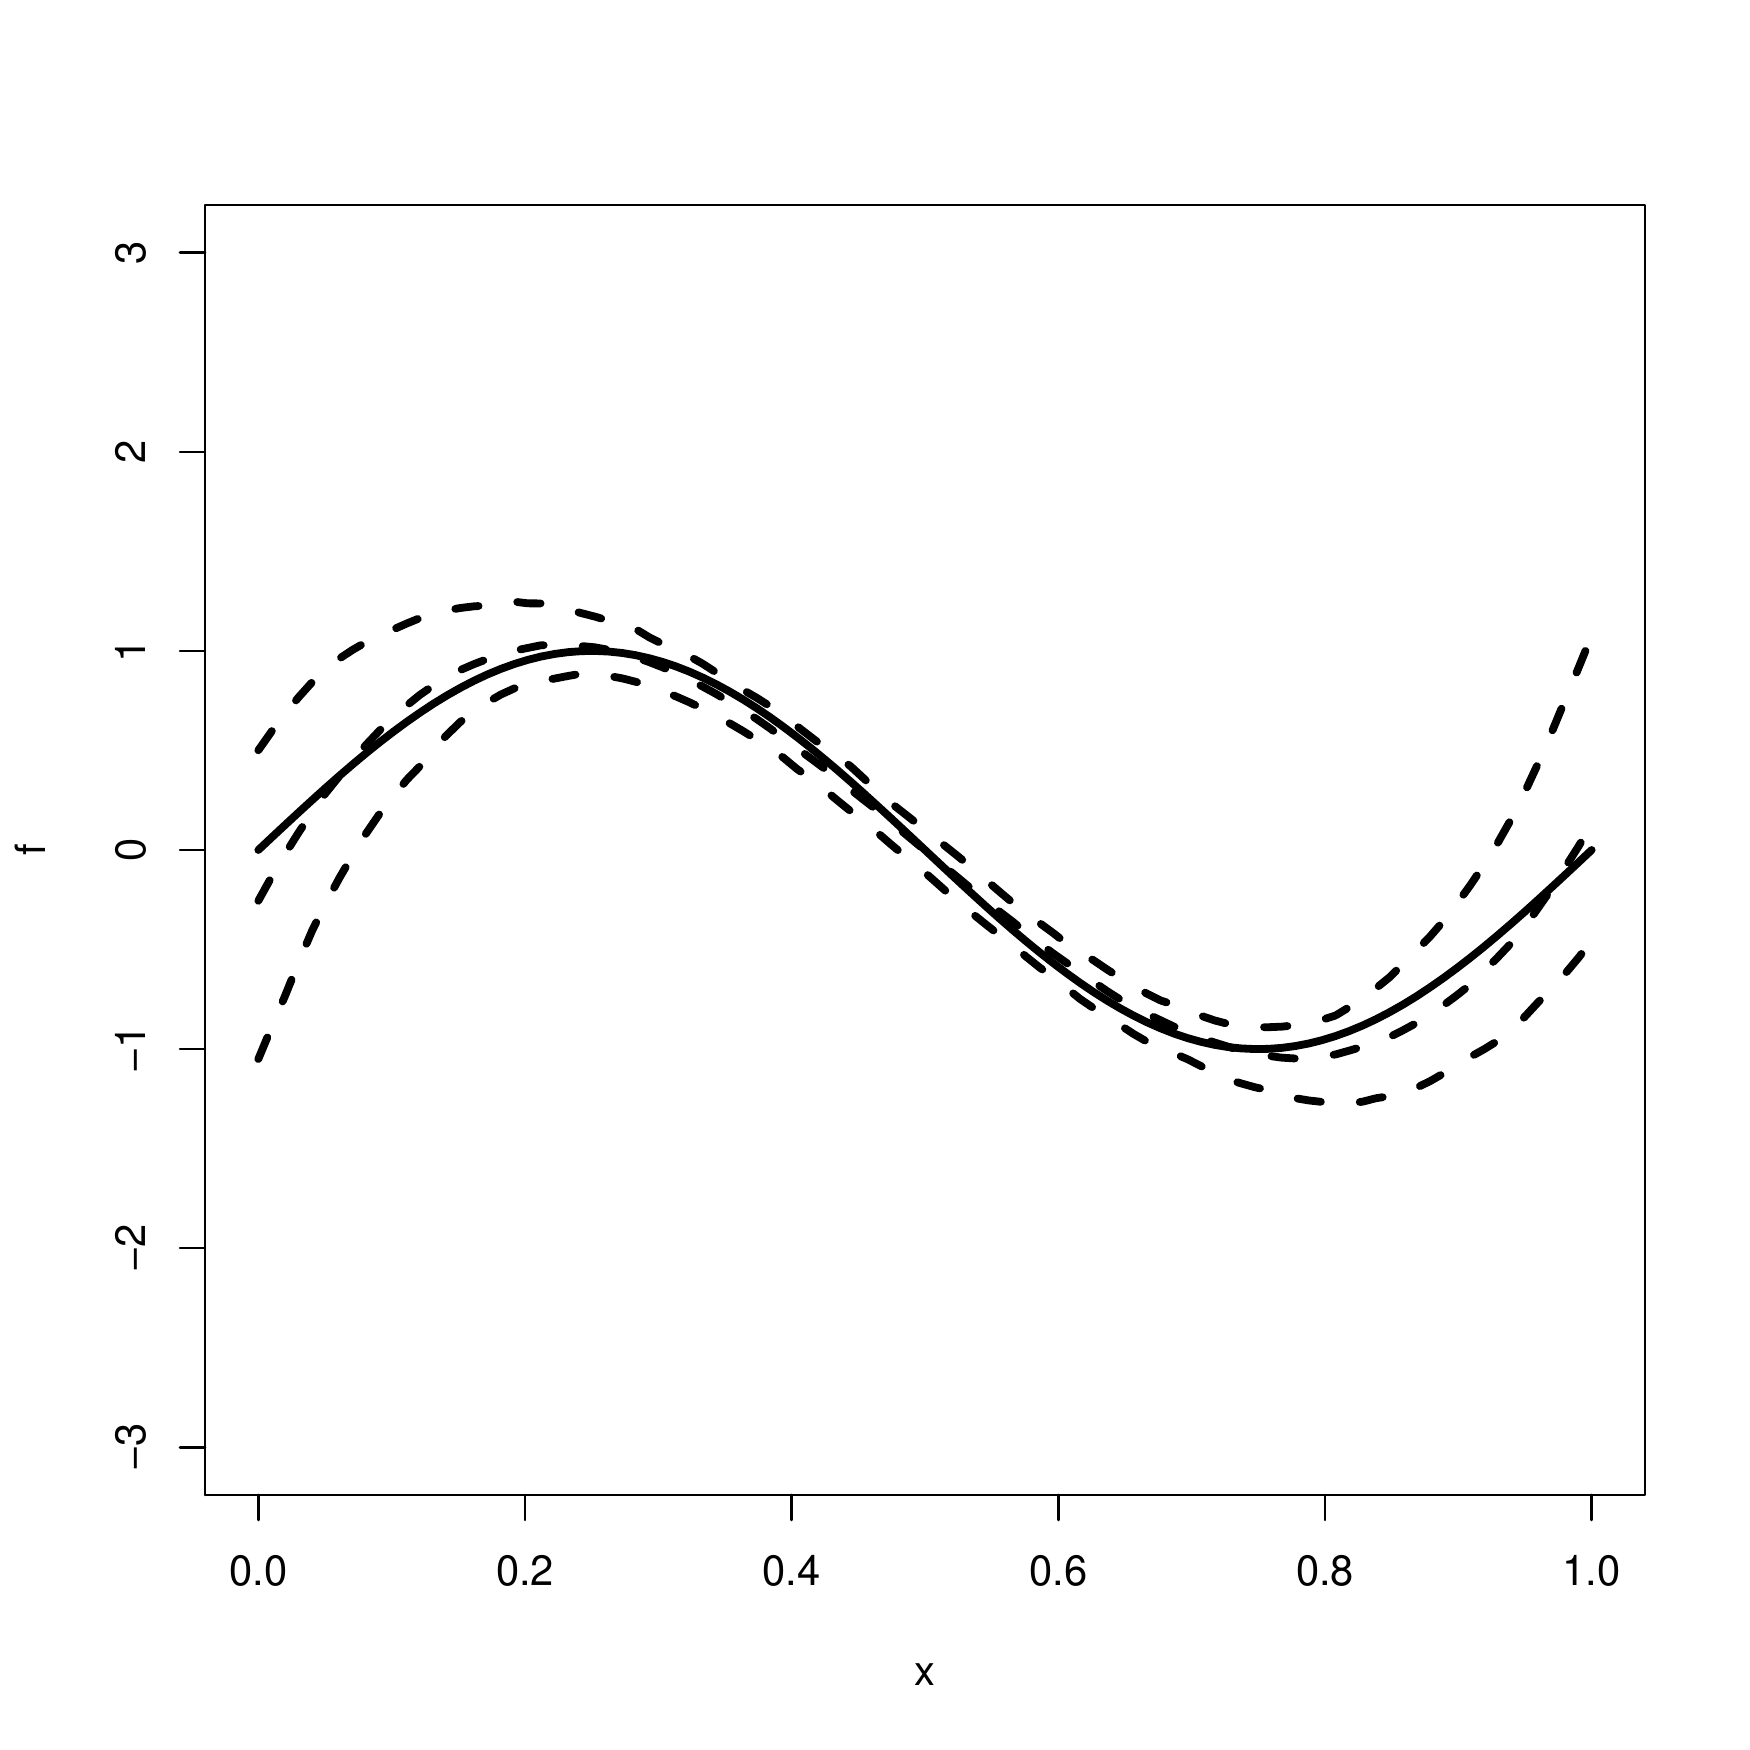}
\includegraphics[scale = 0.35]{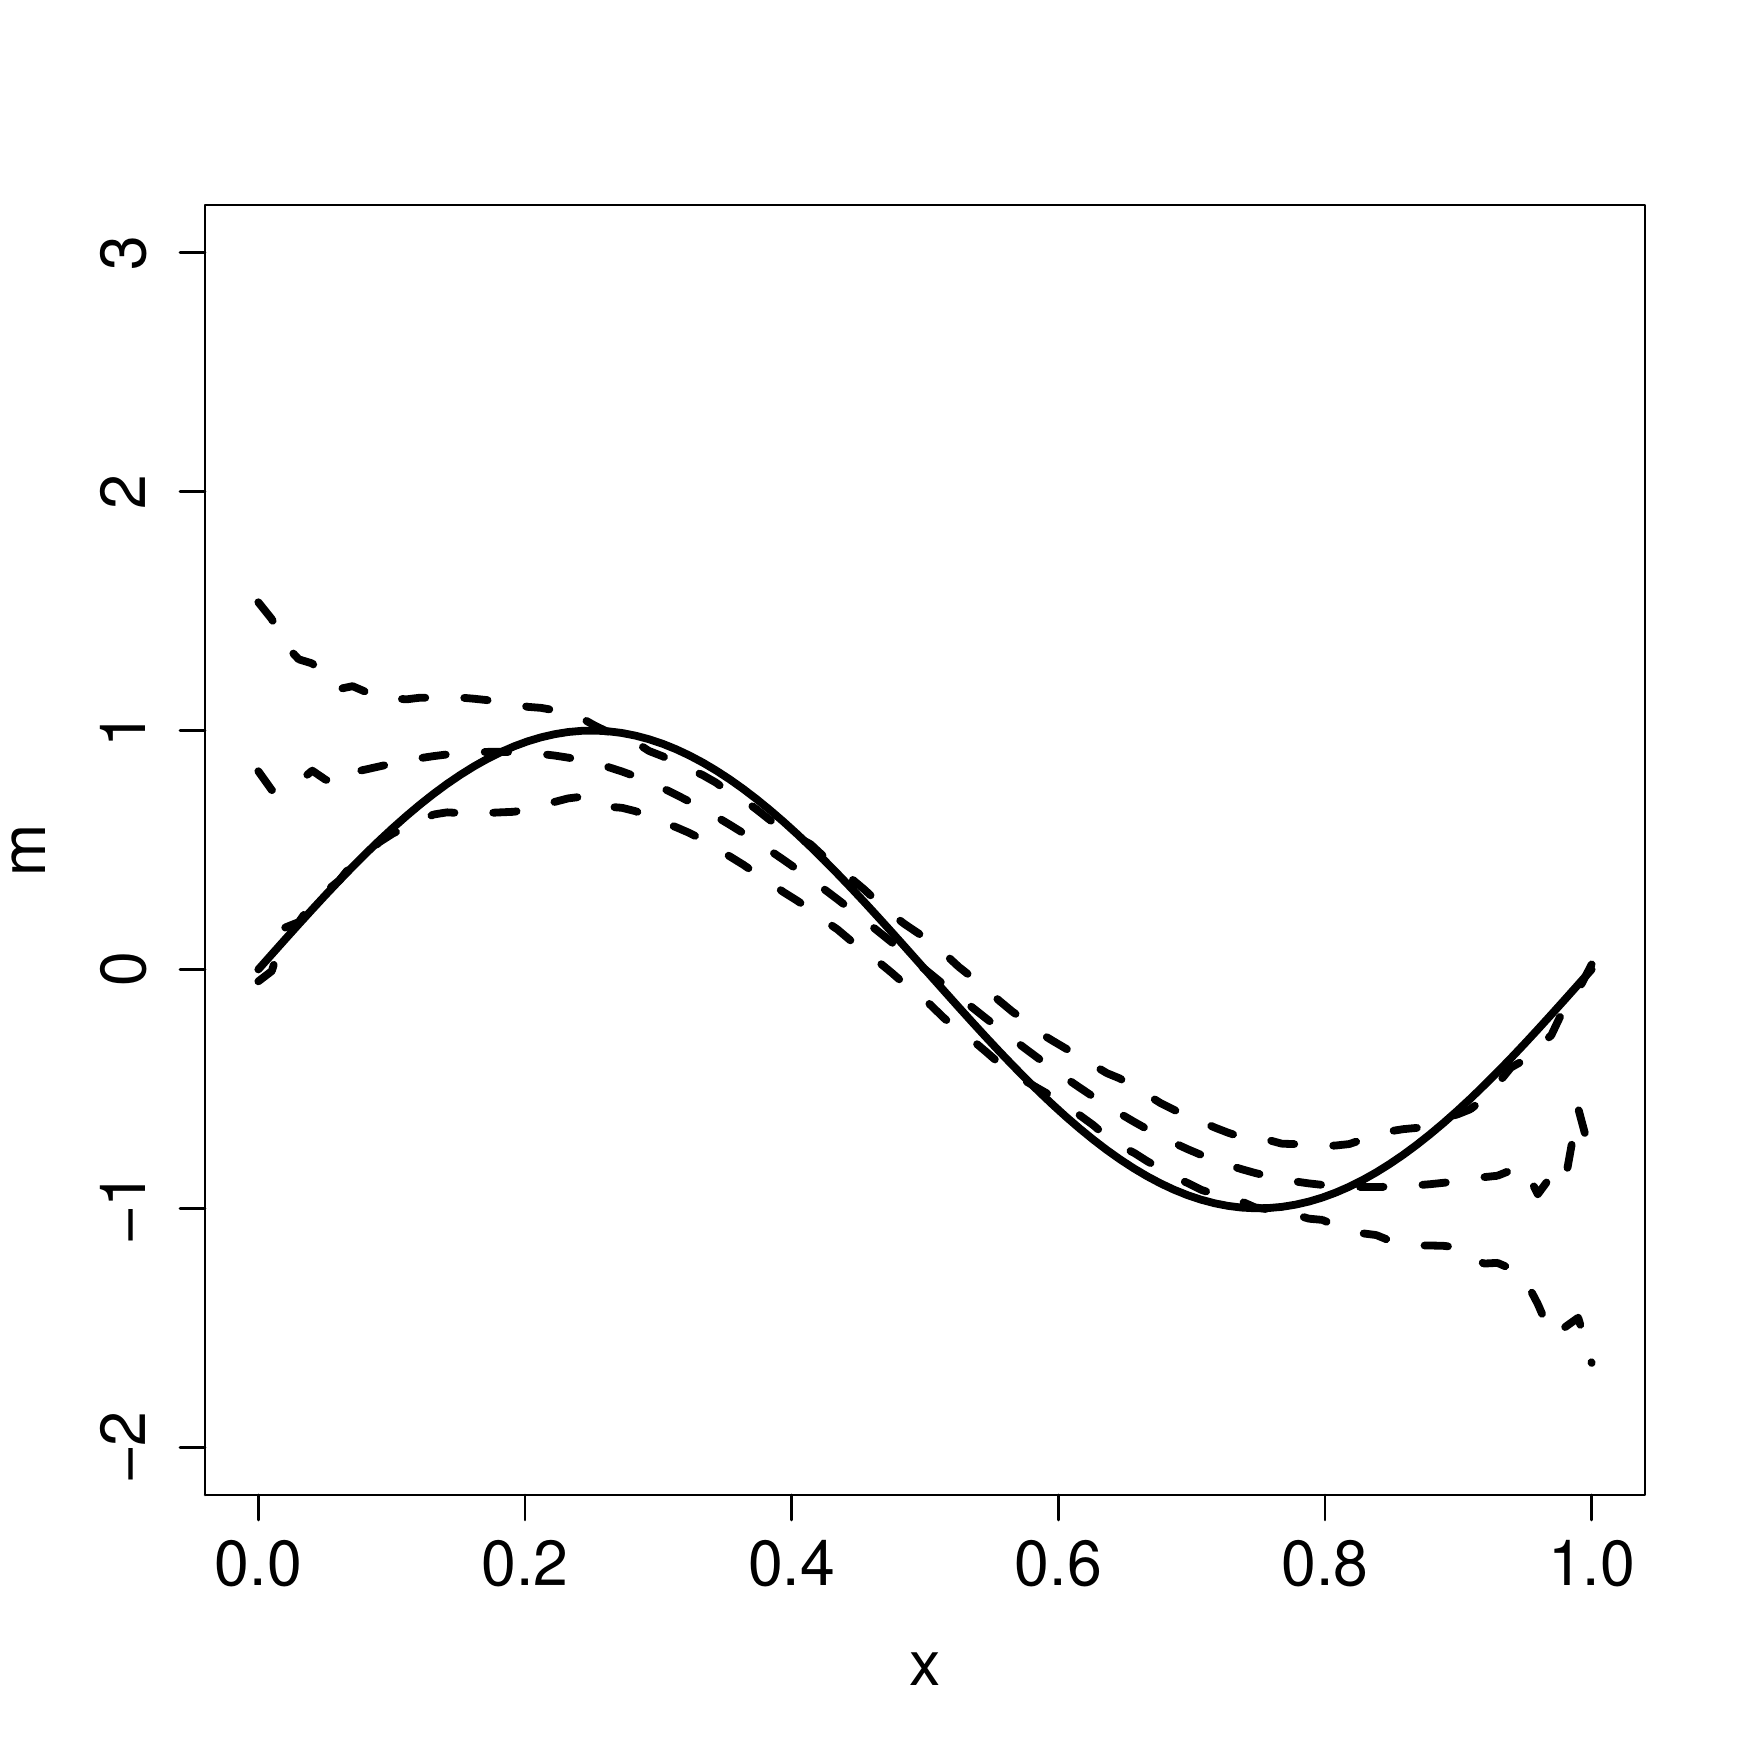}
\end{center}
\end{figure}

\bibliographystyle{agsm}
\bibliography{errorrate}

\end{document}
